# Supplementary material for: Large Cayley graphs of small diameter
Source: arXiv:1708.02425 ancillary file (2018-04-12)
Supplement: Supplementary file 1 [file LargeCayleyGraphsAncillary.pdf]

# Ancillary file for *Large Cayley graphs of small diameter*

Grahame Erskine and James Tuite

## Introduction

This document lists the results of the computer search for constructions of optimal Cayley graphs of given diameter. For full details of the construction, and the notation used, see the main paper. For each optimal result in Tables 1–6 in the main paper, we tabulate the following items:

- The target diameter  $k$ ;
- The target set size  $s = |S|$ ;
- The target order  $n$  for our group  $K$ ;
- A description and presentation of the group  $K$ , and its identity number in the small groups library of GAP;
- The homomorphism  $\varphi : K \rightarrow S_k$ , defined by the images of the generators in the presentation;
- The set  $S$  of  $s$  elements of  $K$ ;
- The set  $V$  of 0/1 vectors;
- For each element  $i$  of  $K$ :
  - The expression of  $i$  as a product of exactly  $k$  elements of  $S$ ;
  - The mapping matrix  $M$  corresponding to this product;
  - The determinant of  $M$  (always  $\pm 1$  since  $M$  must be invertible over  $\mathbb{Z}$ ).

## Solution for undirected graphs of diameter 3

|                               |                                                                                                                                         |
|-------------------------------|-----------------------------------------------------------------------------------------------------------------------------------------|
| Diameter                      | 3                                                                                                                                       |
| Set size                      | 6                                                                                                                                       |
| Group $K$                     | $(\mathbb{Z}_4 \times \mathbb{Z}_4) \rtimes \mathbb{Z}_3$ (order 48; id 3)<br>$\langle x, y \mid x^3, y^4, (yx)^3, (x^{-1}y)^3 \rangle$ |
| $\varphi : K \rightarrow S_3$ | $x \mapsto (1\ 2\ 3)$<br>$y \mapsto ()$                                                                                                 |
| Set $S$                       | $\{s_1, s_2, s_3, s_4, s_5, s_6\} =$<br>$\{x, x^2, xy, (xy)^2, yx, x^2y^3\}$                                                            |
| Set $V$                       | $\{001, 010, 110, 101, 111, 111\}$                                                                                                      |

| No. | Element       | Product       | Mapping matrix $M$                                                  | $\det M$ |
|-----|---------------|---------------|---------------------------------------------------------------------|----------|
| 1.  | 1             | $s_1 s_1 s_1$ | $\begin{pmatrix} 0 & 1 & 0 \\ 1 & 0 & 0 \\ 0 & 0 & 1 \end{pmatrix}$ | -1       |
| 2.  | $x$           | $s_3 s_1 s_6$ | $\begin{pmatrix} 1 & 0 & 1 \\ 1 & 1 & 1 \\ 0 & 0 & 1 \end{pmatrix}$ | 1        |
| 3.  | $y$           | $s_2 s_4 s_4$ | $\begin{pmatrix} 0 & 0 & 1 \\ 0 & 1 & 0 \\ 1 & 1 & 1 \end{pmatrix}$ | -1       |
| 4.  | $x^2 y x$     | $s_1 s_1 s_5$ | $\begin{pmatrix} 0 & 1 & 1 \\ 1 & 0 & 1 \\ 0 & 0 & 1 \end{pmatrix}$ | -1       |
| 5.  | $x^2 y^2 x$   | $s_1 s_3 s_5$ | $\begin{pmatrix} 0 & 0 & 1 \\ 1 & 1 & 1 \\ 0 & 1 & 1 \end{pmatrix}$ | 1        |
| 6.  | $xy^2 x^2$    | $s_2 s_6 s_4$ | $\begin{pmatrix} 0 & 1 & 1 \\ 0 & 1 & 0 \\ 1 & 1 & 1 \end{pmatrix}$ | -1       |
| 7.  | $x^2$         | $s_5 s_2 s_4$ | $\begin{pmatrix} 1 & 1 & 1 \\ 1 & 0 & 0 \\ 1 & 0 & 1 \end{pmatrix}$ | -1       |
| 8.  | $xy$          | $s_1 s_5 s_2$ | $\begin{pmatrix} 0 & 1 & 0 \\ 0 & 1 & 1 \\ 1 & 1 & 0 \end{pmatrix}$ | 1        |
| 9.  | $yx$          | $s_2 s_3 s_1$ | $\begin{pmatrix} 1 & 0 & 0 \\ 0 & 1 & 0 \\ 0 & 1 & 1 \end{pmatrix}$ | 1        |
| 10. | $y^2 x$       | $s_4 s_5 s_3$ | $\begin{pmatrix} 0 & 1 & 1 \\ 1 & 1 & 1 \\ 1 & 1 & 0 \end{pmatrix}$ | 1        |
| 11. | $x^2 y^2 x^2$ | $s_6 s_3 s_3$ | $\begin{pmatrix} 1 & 0 & 1 \\ 1 & 1 & 1 \\ 1 & 1 & 0 \end{pmatrix}$ | -1       |
| 12. | $x(xy)^2$     | $s_1 s_3 s_3$ | $\begin{pmatrix} 0 & 0 & 1 \\ 1 & 1 & 1 \\ 0 & 1 & 0 \end{pmatrix}$ | 1        |

|     |              |             |                                                                     |    |
|-----|--------------|-------------|---------------------------------------------------------------------|----|
| 13. | $x^2y^2xy$   | $s_4s_6s_4$ | $\begin{pmatrix} 1 & 1 & 1 \\ 1 & 1 & 0 \\ 0 & 1 & 1 \end{pmatrix}$ | 1  |
| 14. | $xy^2x^2y$   | $s_3s_5s_3$ | $\begin{pmatrix} 1 & 1 & 1 \\ 0 & 1 & 1 \\ 1 & 1 & 0 \end{pmatrix}$ | -1 |
| 15. | $xyx^2y$     | $s_1s_5s_3$ | $\begin{pmatrix} 0 & 1 & 1 \\ 1 & 1 & 1 \\ 0 & 1 & 0 \end{pmatrix}$ | 1  |
| 16. | $xy(yx)^2$   | $s_4s_4s_6$ | $\begin{pmatrix} 1 & 0 & 1 \\ 1 & 1 & 1 \\ 0 & 1 & 1 \end{pmatrix}$ | 1  |
| 17. | $y^2$        | $s_5s_1s_3$ | $\begin{pmatrix} 1 & 1 & 1 \\ 1 & 0 & 1 \\ 1 & 0 & 0 \end{pmatrix}$ | 1  |
| 18. | $x^2y$       | $s_1s_4s_4$ | $\begin{pmatrix} 1 & 0 & 1 \\ 0 & 1 & 0 \\ 0 & 1 & 1 \end{pmatrix}$ | 1  |
| 19. | $xyx$        | $s_2s_2s_5$ | $\begin{pmatrix} 0 & 0 & 1 \\ 1 & 0 & 1 \\ 0 & 1 & 1 \end{pmatrix}$ | 1  |
| 20. | $xy^2x$      | $s_4s_4s_5$ | $\begin{pmatrix} 1 & 1 & 1 \\ 0 & 1 & 1 \\ 1 & 0 & 1 \end{pmatrix}$ | 1  |
| 21. | $y^2x^2$     | $s_1s_6s_4$ | $\begin{pmatrix} 1 & 1 & 1 \\ 0 & 1 & 0 \\ 0 & 1 & 1 \end{pmatrix}$ | 1  |
| 22. | $yxy$        | $s_1s_1s_4$ | $\begin{pmatrix} 0 & 0 & 1 \\ 0 & 1 & 0 \\ 1 & 0 & 1 \end{pmatrix}$ | -1 |
| 23. | $y^2xy$      | $s_6s_3s_1$ | $\begin{pmatrix} 1 & 0 & 0 \\ 1 & 1 & 0 \\ 1 & 1 & 1 \end{pmatrix}$ | 1  |
| 24. | $x^2y^2x^2y$ | $s_4s_5s_1$ | $\begin{pmatrix} 0 & 1 & 0 \\ 1 & 1 & 0 \\ 1 & 1 & 1 \end{pmatrix}$ | -1 |
| 25. | $(x^2y)^2$   | $s_2s_5s_3$ | $\begin{pmatrix} 1 & 1 & 1 \\ 0 & 1 & 1 \\ 0 & 1 & 0 \end{pmatrix}$ | -1 |
| 26. | $x^2y(yx)^2$ | $s_1s_3s_6$ | $\begin{pmatrix} 0 & 1 & 1 \\ 0 & 0 & 1 \\ 1 & 1 & 1 \end{pmatrix}$ | 1  |
| 27. | $xy^2$       | $s_3s_5s_2$ | $\begin{pmatrix} 1 & 1 & 0 \\ 1 & 1 & 1 \\ 0 & 1 & 0 \end{pmatrix}$ | -1 |
| 28. | $xyx^2y^2$   | $s_6s_4s_4$ | $\begin{pmatrix} 1 & 0 & 1 \\ 1 & 1 & 0 \\ 1 & 1 & 1 \end{pmatrix}$ | 1  |

|     |             |             |                                                                     |    |
|-----|-------------|-------------|---------------------------------------------------------------------|----|
| 29. | $xyx^2$     | $s_1s_5s_1$ | $\begin{pmatrix} 0 & 1 & 0 \\ 1 & 1 & 0 \\ 0 & 1 & 1 \end{pmatrix}$ | -1 |
| 30. | $y^3$       | $s_2s_2s_6$ | $\begin{pmatrix} 0 & 1 & 1 \\ 0 & 0 & 1 \\ 1 & 0 & 1 \end{pmatrix}$ | 1  |
| 31. | $x(xy)^2y$  | $s_5s_3s_3$ | $\begin{pmatrix} 1 & 0 & 1 \\ 1 & 1 & 1 \\ 1 & 1 & 0 \end{pmatrix}$ | -1 |
| 32. | $(xy)^2$    | $s_1s_6s_2$ | $\begin{pmatrix} 1 & 1 & 0 \\ 0 & 1 & 1 \\ 0 & 1 & 0 \end{pmatrix}$ | -1 |
| 33. | $xy^2xy$    | $s_3s_2s_4$ | $\begin{pmatrix} 0 & 1 & 1 \\ 1 & 0 & 0 \\ 1 & 0 & 1 \end{pmatrix}$ | -1 |
| 34. | $y^2x^2y$   | $s_5s_4s_2$ | $\begin{pmatrix} 1 & 0 & 0 \\ 1 & 1 & 1 \\ 1 & 1 & 0 \end{pmatrix}$ | -1 |
| 35. | $yx^2y$     | $s_1s_4s_2$ | $\begin{pmatrix} 1 & 0 & 0 \\ 0 & 1 & 1 \\ 0 & 1 & 0 \end{pmatrix}$ | -1 |
| 36. | $y(yx)^2$   | $s_3s_6s_4$ | $\begin{pmatrix} 0 & 1 & 1 \\ 1 & 1 & 0 \\ 1 & 1 & 1 \end{pmatrix}$ | -1 |
| 37. | $x^2y^2$    | $s_4s_6s_3$ | $\begin{pmatrix} 1 & 1 & 1 \\ 0 & 1 & 1 \\ 1 & 1 & 0 \end{pmatrix}$ | -1 |
| 38. | $(x^2y)^2y$ | $s_4s_1s_3$ | $\begin{pmatrix} 0 & 1 & 1 \\ 1 & 0 & 1 \\ 1 & 0 & 0 \end{pmatrix}$ | 1  |
| 39. | $x^2yx^2$   | $s_1s_3s_2$ | $\begin{pmatrix} 0 & 1 & 0 \\ 0 & 0 & 1 \\ 1 & 1 & 0 \end{pmatrix}$ | 1  |
| 40. | $xy^3$      | $s_1s_1s_6$ | $\begin{pmatrix} 0 & 0 & 1 \\ 0 & 1 & 1 \\ 1 & 0 & 1 \end{pmatrix}$ | -1 |
| 41. | $xyxy^2$    | $s_1s_5s_4$ | $\begin{pmatrix} 0 & 1 & 1 \\ 0 & 1 & 0 \\ 1 & 1 & 1 \end{pmatrix}$ | -1 |
| 42. | $(xy)^2yx$  | $s_3s_3s_5$ | $\begin{pmatrix} 1 & 0 & 1 \\ 0 & 1 & 1 \\ 1 & 1 & 1 \end{pmatrix}$ | -1 |
| 43. | $yx^2y^2$   | $s_2s_6s_3$ | $\begin{pmatrix} 0 & 1 & 1 \\ 1 & 1 & 1 \\ 0 & 1 & 0 \end{pmatrix}$ | 1  |
| 44. | $yx^2$      | $s_5s_2s_2$ | $\begin{pmatrix} 1 & 1 & 0 \\ 1 & 0 & 1 \\ 1 & 0 & 0 \end{pmatrix}$ | 1  |

|     |             |             |                                                                     |      |
|-----|-------------|-------------|---------------------------------------------------------------------|------|
| 45. | $x^2y^3$    | $s_2s_4s_1$ | $\begin{pmatrix} 0 & 1 & 0 \\ 1 & 1 & 0 \\ 0 & 0 & 1 \end{pmatrix}$ | $-1$ |
| 46. | $(xy)^2y$   | $s_4s_2s_3$ | $\begin{pmatrix} 1 & 0 & 1 \\ 0 & 0 & 1 \\ 1 & 1 & 0 \end{pmatrix}$ | $-1$ |
| 47. | $x(xy)^2yx$ | $s_3s_5s_4$ | $\begin{pmatrix} 1 & 1 & 1 \\ 1 & 1 & 0 \\ 0 & 1 & 1 \end{pmatrix}$ | $1$  |
| 48. | $yxxy^2x$   | $s_2s_4s_5$ | $\begin{pmatrix} 0 & 1 & 1 \\ 1 & 1 & 1 \\ 0 & 0 & 1 \end{pmatrix}$ | $-1$ |

## Solution for undirected graphs of diameter 4

|                               |                                                                                                                                         |
|-------------------------------|-----------------------------------------------------------------------------------------------------------------------------------------|
| Diameter                      | 4                                                                                                                                       |
| Set size                      | 5                                                                                                                                       |
| Group $K$                     | $\mathbb{Z}_{15} \rtimes \mathbb{Z}_4$ (order 60; id 7)<br>$\langle x, y \mid x^4, y^{15}, xyx^{-1}y^{-2}, (xy^{-1})^4, (xy)^4 \rangle$ |
| $\varphi : K \rightarrow S_4$ | $x \mapsto (1\ 2\ 3\ 4)$<br>$y \mapsto ()$                                                                                              |
| Set $S$                       | $\{s_1, s_2, s_3, s_4, s_5\} =$<br>$\{x, x^3, xy, (xy)^3, yx^2y^2\}$                                                                    |
| Set $V$                       | $\{0001, 0010, 1011, 0111, 0101\}$                                                                                                      |

| No. | Element      | Product           | Mapping matrix $M$                                                                               | $\det M$ |
|-----|--------------|-------------------|--------------------------------------------------------------------------------------------------|----------|
| 1.  | 1            | $s_1 s_1 s_1 s_1$ | $\begin{pmatrix} 0 & 0 & 1 & 0 \\ 0 & 1 & 0 & 0 \\ 1 & 0 & 0 & 0 \\ 0 & 0 & 0 & 1 \end{pmatrix}$ | -1       |
| 2.  | $x$          | $s_2 s_4 s_5 s_3$ | $\begin{pmatrix} 1 & 1 & 1 & 1 \\ 0 & 1 & 0 & 0 \\ 0 & 1 & 1 & 1 \\ 0 & 0 & 0 & 1 \end{pmatrix}$ | 1        |
| 3.  | $x^2$        | $s_5 s_4 s_5 s_4$ | $\begin{pmatrix} 0 & 1 & 1 & 0 \\ 1 & 0 & 0 & 1 \\ 0 & 1 & 1 & 1 \\ 1 & 1 & 0 & 1 \end{pmatrix}$ | -1       |
| 4.  | $x^2(xy)^2y$ | $s_3 s_1 s_3 s_1$ | $\begin{pmatrix} 0 & 0 & 1 & 0 \\ 1 & 1 & 1 & 0 \\ 1 & 0 & 0 & 0 \\ 1 & 0 & 1 & 1 \end{pmatrix}$ | -1       |
| 5.  | $(x^2y)^2y$  | $s_3 s_3 s_2 s_2$ | $\begin{pmatrix} 0 & 1 & 0 & 0 \\ 1 & 1 & 1 & 0 \\ 1 & 1 & 0 & 1 \\ 1 & 0 & 0 & 0 \end{pmatrix}$ | -1       |
| 6.  | $x^3$        | $s_4 s_5 s_3 s_1$ | $\begin{pmatrix} 0 & 0 & 1 & 0 \\ 1 & 1 & 1 & 0 \\ 1 & 0 & 0 & 0 \\ 1 & 1 & 1 & 1 \end{pmatrix}$ | -1       |
| 7.  | $xyx^2$      | $s_1 s_1 s_3 s_5$ | $\begin{pmatrix} 0 & 0 & 1 & 0 \\ 0 & 0 & 1 & 1 \\ 0 & 1 & 1 & 0 \\ 1 & 0 & 0 & 1 \end{pmatrix}$ | -1       |
| 8.  | $x(x^2y)^2y$ | $s_5 s_1 s_3 s_3$ | $\begin{pmatrix} 1 & 0 & 1 & 1 \\ 0 & 1 & 1 & 0 \\ 1 & 0 & 0 & 1 \\ 0 & 0 & 1 & 1 \end{pmatrix}$ | -1       |
| 9.  | $(xy)^2y$    | $s_5 s_1 s_5 s_3$ | $\begin{pmatrix} 0 & 0 & 1 & 1 \\ 1 & 0 & 0 & 0 \\ 0 & 1 & 1 & 1 \\ 1 & 0 & 0 & 1 \end{pmatrix}$ | 1        |

|     |              |                |                                                                                                  |    |
|-----|--------------|----------------|--------------------------------------------------------------------------------------------------|----|
| 10. | $yx^2y^2$    | $s_3s_1s_1s_4$ | $\begin{pmatrix} 1 & 0 & 0 & 0 \\ 1 & 0 & 0 & 1 \\ 0 & 0 & 1 & 1 \\ 1 & 1 & 0 & 1 \end{pmatrix}$ | -1 |
| 11. | $(x^2y)^2$   | $s_1s_3s_1s_3$ | $\begin{pmatrix} 0 & 1 & 1 & 1 \\ 0 & 1 & 0 & 0 \\ 1 & 1 & 0 & 1 \\ 0 & 0 & 0 & 1 \end{pmatrix}$ | -1 |
| 12. | $y$          | $s_1s_1s_1s_3$ | $\begin{pmatrix} 0 & 0 & 1 & 1 \\ 0 & 1 & 0 & 0 \\ 1 & 0 & 0 & 1 \\ 0 & 0 & 0 & 1 \end{pmatrix}$ | -1 |
| 13. | $x(xy)^2x$   | $s_1s_4s_4s_1$ | $\begin{pmatrix} 0 & 0 & 1 & 0 \\ 0 & 1 & 0 & 0 \\ 1 & 1 & 1 & 0 \\ 0 & 1 & 1 & 1 \end{pmatrix}$ | -1 |
| 14. | $x(xy)^2y$   | $s_1s_1s_5s_4$ | $\begin{pmatrix} 0 & 1 & 1 & 0 \\ 1 & 0 & 0 & 1 \\ 0 & 0 & 1 & 1 \\ 0 & 0 & 0 & 1 \end{pmatrix}$ | -1 |
| 15. | $xyx^2y^2$   | $s_2s_2s_2s_5$ | $\begin{pmatrix} 0 & 0 & 1 & 0 \\ 0 & 0 & 0 & 1 \\ 1 & 0 & 0 & 0 \\ 0 & 1 & 0 & 1 \end{pmatrix}$ | 1  |
| 16. | $x(x^2y)^2$  | $s_1s_5s_4s_2$ | $\begin{pmatrix} 0 & 0 & 1 & 0 \\ 0 & 1 & 1 & 0 \\ 0 & 0 & 1 & 1 \\ 1 & 1 & 0 & 0 \end{pmatrix}$ | 1  |
| 17. | $xy$         | $s_5s_3s_1s_1$ | $\begin{pmatrix} 1 & 1 & 1 & 0 \\ 0 & 1 & 0 & 0 \\ 1 & 1 & 0 & 0 \\ 0 & 0 & 0 & 1 \end{pmatrix}$ | -1 |
| 18. | $x^2(xy)^2x$ | $s_1s_3s_3s_5$ | $\begin{pmatrix} 0 & 0 & 1 & 0 \\ 0 & 1 & 1 & 1 \\ 0 & 1 & 1 & 0 \\ 1 & 1 & 0 & 1 \end{pmatrix}$ | -1 |
| 19. | $yx^2y$      | $s_1s_4s_2s_4$ | $\begin{pmatrix} 1 & 1 & 0 & 0 \\ 0 & 1 & 1 & 1 \\ 0 & 0 & 0 & 1 \\ 0 & 1 & 0 & 1 \end{pmatrix}$ | 1  |
| 20. | $x^2y$       | $s_1s_4s_4s_4$ | $\begin{pmatrix} 1 & 1 & 1 & 0 \\ 0 & 1 & 1 & 1 \\ 0 & 0 & 1 & 1 \\ 0 & 1 & 0 & 1 \end{pmatrix}$ | 1  |
| 21. | $(yx)^2$     | $s_2s_3s_3s_1$ | $\begin{pmatrix} 0 & 1 & 1 & 0 \\ 1 & 1 & 1 & 0 \\ 0 & 1 & 0 & 0 \\ 0 & 0 & 1 & 1 \end{pmatrix}$ | 1  |

|     |                |                |                                                                                                  |    |
|-----|----------------|----------------|--------------------------------------------------------------------------------------------------|----|
| 22. | $x^2(xy)^2y^2$ | $s_2s_2s_4s_2$ | $\begin{pmatrix} 0 & 1 & 1 & 0 \\ 0 & 0 & 1 & 0 \\ 0 & 0 & 1 & 1 \\ 1 & 0 & 0 & 0 \end{pmatrix}$ | -1 |
| 23. | $(x^2y)^2y^2$  | $s_2s_4s_2s_2$ | $\begin{pmatrix} 0 & 1 & 0 & 0 \\ 0 & 1 & 1 & 0 \\ 0 & 0 & 0 & 1 \\ 1 & 1 & 0 & 0 \end{pmatrix}$ | -1 |
| 24. | $y^3$          | $s_2s_3s_3s_2$ | $\begin{pmatrix} 0 & 1 & 0 & 0 \\ 0 & 0 & 1 & 0 \\ 0 & 1 & 1 & 1 \\ 1 & 1 & 1 & 0 \end{pmatrix}$ | -1 |
| 25. | $xyx^2y$       | $s_1s_3s_5s_2$ | $\begin{pmatrix} 0 & 1 & 1 & 0 \\ 1 & 1 & 0 & 0 \\ 0 & 0 & 1 & 1 \\ 0 & 1 & 0 & 0 \end{pmatrix}$ | -1 |
| 26. | $x^3y$         | $s_5s_1s_1s_4$ | $\begin{pmatrix} 1 & 0 & 0 & 0 \\ 0 & 0 & 0 & 1 \\ 1 & 0 & 1 & 1 \\ 0 & 1 & 0 & 1 \end{pmatrix}$ | -1 |
| 27. | $(xy)^2x$      | $s_2s_4s_4s_5$ | $\begin{pmatrix} 0 & 1 & 1 & 0 \\ 0 & 0 & 1 & 1 \\ 1 & 1 & 0 & 0 \\ 0 & 1 & 1 & 1 \end{pmatrix}$ | 1  |
| 28. | $xyx^3$        | $s_4s_2s_5s_3$ | $\begin{pmatrix} 1 & 0 & 1 & 1 \\ 1 & 1 & 0 & 0 \\ 0 & 0 & 1 & 1 \\ 1 & 0 & 0 & 1 \end{pmatrix}$ | 1  |
| 29. | $x(x^2y)^2y^2$ | $s_2s_5s_2s_3$ | $\begin{pmatrix} 1 & 0 & 0 & 1 \\ 0 & 1 & 0 & 0 \\ 0 & 0 & 0 & 1 \\ 0 & 1 & 1 & 1 \end{pmatrix}$ | -1 |
| 30. | $xy^3$         | $s_1s_5s_3s_3$ | $\begin{pmatrix} 0 & 0 & 1 & 1 \\ 0 & 1 & 1 & 0 \\ 0 & 0 & 0 & 1 \\ 1 & 1 & 1 & 1 \end{pmatrix}$ | 1  |
| 31. | $(xy)^2y^2$    | $s_5s_3s_5s_1$ | $\begin{pmatrix} 0 & 0 & 1 & 0 \\ 1 & 1 & 0 & 0 \\ 0 & 1 & 1 & 0 \\ 1 & 1 & 0 & 1 \end{pmatrix}$ | 1  |
| 32. | $yx^2y^3$      | $s_1s_5s_3s_5$ | $\begin{pmatrix} 1 & 1 & 1 & 0 \\ 0 & 0 & 1 & 1 \\ 0 & 1 & 1 & 0 \\ 0 & 0 & 0 & 1 \end{pmatrix}$ | -1 |
| 33. | $x^2y^3$       | $s_1s_5s_1s_5$ | $\begin{pmatrix} 1 & 1 & 0 & 0 \\ 0 & 0 & 1 & 1 \\ 0 & 1 & 0 & 0 \\ 0 & 0 & 0 & 1 \end{pmatrix}$ | -1 |



|     |               |                   |                                                                                                  |    |
|-----|---------------|-------------------|--------------------------------------------------------------------------------------------------|----|
| 34. | $y^2$         | $s_1 s_3 s_2 s_4$ | $\begin{pmatrix} 0 & 1 & 0 & 0 \\ 0 & 1 & 1 & 1 \\ 1 & 1 & 0 & 1 \\ 0 & 0 & 0 & 1 \end{pmatrix}$ | 1  |
| 35. | $x(xy)^3$     | $s_1 s_3 s_3 s_3$ | $\begin{pmatrix} 0 & 1 & 1 & 1 \\ 0 & 1 & 1 & 0 \\ 1 & 1 & 0 & 1 \\ 0 & 0 & 1 & 1 \end{pmatrix}$ | 1  |
| 36. | $x^2(xy)^2$   | $s_1 s_1 s_4 s_4$ | $\begin{pmatrix} 0 & 0 & 1 & 0 \\ 0 & 1 & 1 & 1 \\ 1 & 0 & 1 & 1 \\ 0 & 0 & 0 & 1 \end{pmatrix}$ | -1 |
| 37. | $x(xy)^2 y^2$ | $s_5 s_2 s_3 s_1$ | $\begin{pmatrix} 1 & 1 & 1 & 0 \\ 0 & 0 & 1 & 0 \\ 1 & 0 & 0 & 0 \\ 0 & 0 & 1 & 1 \end{pmatrix}$ | 1  |
| 38. | $xyx^2 y^3$   | $s_4 s_5 s_1 s_1$ | $\begin{pmatrix} 0 & 0 & 1 & 0 \\ 1 & 1 & 0 & 0 \\ 1 & 0 & 0 & 0 \\ 1 & 1 & 0 & 1 \end{pmatrix}$ | -1 |
| 39. | $x^3 y^3$     | $s_2 s_5 s_3 s_3$ | $\begin{pmatrix} 0 & 0 & 1 & 1 \\ 0 & 1 & 1 & 0 \\ 1 & 0 & 0 & 1 \\ 0 & 1 & 1 & 1 \end{pmatrix}$ | -1 |
| 40. | $xy^2$        | $s_2 s_4 s_1 s_5$ | $\begin{pmatrix} 1 & 1 & 0 & 0 \\ 0 & 1 & 1 & 1 \\ 0 & 1 & 0 & 0 \\ 0 & 0 & 0 & 1 \end{pmatrix}$ | -1 |
| 41. | $x^2(xy)^3$   | $s_5 s_1 s_1 s_3$ | $\begin{pmatrix} 1 & 0 & 1 & 1 \\ 0 & 1 & 0 & 0 \\ 1 & 0 & 0 & 1 \\ 0 & 0 & 0 & 1 \end{pmatrix}$ | -1 |
| 42. | $xyx$         | $s_5 s_3 s_3 s_1$ | $\begin{pmatrix} 1 & 1 & 1 & 0 \\ 0 & 1 & 1 & 0 \\ 1 & 1 & 0 & 0 \\ 0 & 0 & 1 & 1 \end{pmatrix}$ | -1 |
| 43. | $x^2 y^2$     | $s_1 s_1 s_3 s_2$ | $\begin{pmatrix} 1 & 0 & 0 & 0 \\ 0 & 0 & 1 & 0 \\ 0 & 0 & 1 & 1 \\ 0 & 1 & 1 & 0 \end{pmatrix}$ | 1  |
| 44. | $(yx)^2 y$    | $s_1 s_1 s_1 s_4$ | $\begin{pmatrix} 1 & 0 & 0 & 0 \\ 0 & 0 & 0 & 1 \\ 0 & 0 & 1 & 1 \\ 0 & 1 & 0 & 1 \end{pmatrix}$ | -1 |
| 45. | $(xy)^2$      | $s_2 s_5 s_2 s_5$ | $\begin{pmatrix} 0 & 1 & 1 & 0 \\ 1 & 0 & 0 & 1 \\ 0 & 1 & 0 & 0 \\ 0 & 0 & 0 & 1 \end{pmatrix}$ | 1  |

|     |           |                |                                                                                                  |    |
|-----|-----------|----------------|--------------------------------------------------------------------------------------------------|----|
| 46. | $x^3yx$   | $s_1s_1s_3s_1$ | $\begin{pmatrix} 0 & 0 & 1 & 0 \\ 0 & 1 & 1 & 0 \\ 1 & 0 & 0 & 0 \\ 0 & 0 & 1 & 1 \end{pmatrix}$ | -1 |
| 47. | $x^2yx^2$ | $s_1s_3s_1s_1$ | $\begin{pmatrix} 0 & 1 & 1 & 0 \\ 0 & 1 & 0 & 0 \\ 1 & 1 & 0 & 0 \\ 0 & 0 & 0 & 1 \end{pmatrix}$ | -1 |
| 48. | $x^3y^2$  | $s_2s_5s_3s_1$ | $\begin{pmatrix} 0 & 0 & 1 & 0 \\ 0 & 1 & 1 & 0 \\ 1 & 0 & 0 & 0 \\ 0 & 1 & 1 & 1 \end{pmatrix}$ | -1 |
| 49. | $(xy)^3$  | $s_2s_2s_4s_5$ | $\begin{pmatrix} 0 & 0 & 1 & 0 \\ 0 & 0 & 1 & 1 \\ 1 & 0 & 0 & 0 \\ 0 & 1 & 1 & 1 \end{pmatrix}$ | 1  |
| 50. | $x(xy)^2$ | $s_2s_5s_1s_1$ | $\begin{pmatrix} 0 & 0 & 1 & 0 \\ 0 & 1 & 0 & 0 \\ 1 & 0 & 0 & 0 \\ 0 & 1 & 0 & 1 \end{pmatrix}$ | -1 |
| 51. | $yx$      | $s_3s_5s_2s_4$ | $\begin{pmatrix} 1 & 0 & 0 & 0 \\ 0 & 1 & 1 & 1 \\ 1 & 0 & 0 & 1 \\ 1 & 1 & 0 & 1 \end{pmatrix}$ | 1  |
| 52. | $x^3yx^2$ | $s_2s_2s_5s_3$ | $\begin{pmatrix} 1 & 0 & 1 & 1 \\ 0 & 1 & 0 & 0 \\ 0 & 0 & 1 & 1 \\ 0 & 0 & 0 & 1 \end{pmatrix}$ | 1  |
| 53. | $xyx$     | $s_3s_2s_2s_2$ | $\begin{pmatrix} 1 & 1 & 0 & 0 \\ 1 & 0 & 1 & 0 \\ 0 & 0 & 0 & 1 \\ 1 & 0 & 0 & 0 \end{pmatrix}$ | -1 |
| 54. | $yx^2$    | $s_2s_3s_1s_1$ | $\begin{pmatrix} 0 & 1 & 1 & 0 \\ 1 & 1 & 0 & 0 \\ 0 & 1 & 0 & 0 \\ 0 & 0 & 0 & 1 \end{pmatrix}$ | 1  |
| 55. | $(xy)^3x$ | $s_1s_4s_2s_3$ | $\begin{pmatrix} 0 & 0 & 0 & 1 \\ 0 & 1 & 0 & 0 \\ 1 & 1 & 0 & 1 \\ 0 & 1 & 1 & 1 \end{pmatrix}$ | 1  |
| 56. | $x^2yx$   | $s_4s_5s_1s_3$ | $\begin{pmatrix} 0 & 0 & 1 & 1 \\ 1 & 1 & 0 & 0 \\ 1 & 0 & 0 & 1 \\ 1 & 1 & 0 & 1 \end{pmatrix}$ | -1 |
| 57. | $xyx^2$   | $s_4s_2s_2s_5$ | $\begin{pmatrix} 0 & 0 & 1 & 0 \\ 1 & 0 & 0 & 1 \\ 1 & 0 & 0 & 0 \\ 1 & 1 & 0 & 1 \end{pmatrix}$ | 1  |

|     |              |                |                                                                                                  |    |
|-----|--------------|----------------|--------------------------------------------------------------------------------------------------|----|
| 58. | $x(xy)^3x$   | $s_2s_4s_5s_1$ | $\begin{pmatrix} 1 & 1 & 1 & 0 \\ 0 & 1 & 0 & 0 \\ 0 & 1 & 1 & 0 \\ 0 & 0 & 0 & 1 \end{pmatrix}$ | 1  |
| 59. | $x^2(xy)^3x$ | $s_1s_3s_1s_4$ | $\begin{pmatrix} 1 & 1 & 0 & 0 \\ 0 & 0 & 0 & 1 \\ 0 & 1 & 1 & 1 \\ 0 & 1 & 0 & 1 \end{pmatrix}$ | -1 |
| 60. | $(yx)^3$     | $s_3s_1s_5s_4$ | $\begin{pmatrix} 1 & 1 & 1 & 0 \\ 1 & 0 & 0 & 1 \\ 1 & 0 & 1 & 1 \\ 0 & 0 & 0 & 1 \end{pmatrix}$ | -1 |

## Solution for undirected graphs of diameter 5

|                               |                                                                                       |
|-------------------------------|---------------------------------------------------------------------------------------|
| Diameter                      | 5                                                                                     |
| Set size                      | 4                                                                                     |
| Group $K$                     | $A_5$ (order 60; id 5)<br>$\langle x, y \mid x^5, y^3, (x^2y)^2, (yx^{-1})^3 \rangle$ |
| $\varphi : K \rightarrow S_5$ | $x \mapsto (1\ 4\ 5\ 2\ 3)$<br>$y \mapsto (1\ 4\ 3)$                                  |
| Set $S$                       | $\{s_1, s_2, s_3, s_4\} =$<br>$\{(yx)^2y, (xy)^2x, x^2(xy)^3, x(xy)^3y\}$             |
| Set $V$                       | $\{10000, 00001, 10110, 10111\}$                                                      |

| No. | Element     | Product           | Mapping matrix $M$                                                                                                                    | $\det M$ |
|-----|-------------|-------------------|---------------------------------------------------------------------------------------------------------------------------------------|----------|
| 1.  | 1           | $s_1s_1s_1s_1s_1$ | $\begin{pmatrix} 0 & 0 & 0 & 0 & 1 \\ 0 & 0 & 0 & 1 & 0 \\ 0 & 0 & 1 & 0 & 0 \\ 0 & 1 & 0 & 0 & 0 \\ 1 & 0 & 0 & 0 & 0 \end{pmatrix}$ | 1        |
| 2.  | $x^4y^2x^2$ | $s_3s_4s_2s_4s_1$ | $\begin{pmatrix} 1 & 1 & 0 & 1 & 1 \\ 1 & 1 & 0 & 1 & 0 \\ 0 & 1 & 0 & 0 & 0 \\ 1 & 1 & 1 & 1 & 0 \\ 0 & 0 & 0 & 1 & 0 \end{pmatrix}$ | 1        |
| 3.  | $x^3yx$     | $s_2s_4s_3s_1s_1$ | $\begin{pmatrix} 0 & 1 & 1 & 0 & 1 \\ 0 & 0 & 0 & 1 & 0 \\ 1 & 1 & 1 & 0 & 0 \\ 0 & 1 & 0 & 0 & 0 \\ 0 & 1 & 1 & 0 & 0 \end{pmatrix}$ | -1       |
| 4.  | $(xy)^3y$   | $s_1s_3s_1s_3s_4$ | $\begin{pmatrix} 1 & 1 & 0 & 1 & 1 \\ 0 & 1 & 0 & 0 & 0 \\ 0 & 1 & 0 & 0 & 1 \\ 0 & 0 & 0 & 1 & 1 \\ 0 & 0 & 1 & 1 & 1 \end{pmatrix}$ | -1       |
| 5.  | $x(xy)^2y$  | $s_3s_2s_2s_3s_2$ | $\begin{pmatrix} 0 & 0 & 1 & 0 & 0 \\ 1 & 0 & 0 & 1 & 0 \\ 1 & 1 & 0 & 1 & 0 \\ 1 & 0 & 0 & 0 & 0 \\ 0 & 0 & 0 & 1 & 1 \end{pmatrix}$ | -1       |
| 6.  | $x(xy)^2x$  | $s_3s_2s_4s_2s_3$ | $\begin{pmatrix} 0 & 0 & 1 & 0 & 1 \\ 0 & 0 & 1 & 1 & 0 \\ 1 & 0 & 0 & 0 & 1 \\ 1 & 0 & 1 & 0 & 1 \\ 1 & 1 & 1 & 0 & 0 \end{pmatrix}$ | 1        |
| 7.  | $yxxy$      | $s_1s_3s_1s_1s_3$ | $\begin{pmatrix} 0 & 1 & 0 & 0 & 1 \\ 1 & 1 & 0 & 0 & 0 \\ 0 & 1 & 0 & 1 & 1 \\ 0 & 0 & 0 & 0 & 1 \\ 0 & 0 & 1 & 0 & 0 \end{pmatrix}$ | -1       |

|     |             |                   |                                                                                                                                       |    |
|-----|-------------|-------------------|---------------------------------------------------------------------------------------------------------------------------------------|----|
| 8.  | $y^2x$      | $s_3s_4s_3s_4s_2$ | $\begin{pmatrix} 1 & 1 & 0 & 0 & 0 \\ 0 & 0 & 0 & 1 & 0 \\ 0 & 1 & 1 & 1 & 0 \\ 1 & 1 & 1 & 1 & 0 \\ 1 & 1 & 1 & 1 & 1 \end{pmatrix}$ | 1  |
| 9.  | $x^2(xy)^3$ | $s_4s_2s_3s_1s_1$ | $\begin{pmatrix} 1 & 0 & 1 & 0 & 1 \\ 1 & 0 & 0 & 1 & 0 \\ 1 & 0 & 1 & 0 & 0 \\ 1 & 1 & 0 & 0 & 0 \\ 0 & 0 & 1 & 0 & 0 \end{pmatrix}$ | -1 |
| 10. | $x^4y^2xy$  | $s_3s_1s_4s_1s_3$ | $\begin{pmatrix} 1 & 0 & 0 & 0 & 1 \\ 0 & 1 & 1 & 0 & 0 \\ 0 & 0 & 1 & 1 & 1 \\ 1 & 0 & 1 & 0 & 1 \\ 1 & 0 & 1 & 0 & 0 \end{pmatrix}$ | 1  |
| 11. | $x^4y$      | $s_3s_1s_3s_1s_1$ | $\begin{pmatrix} 1 & 0 & 1 & 0 & 1 \\ 1 & 0 & 0 & 1 & 0 \\ 0 & 0 & 1 & 0 & 0 \\ 1 & 0 & 0 & 0 & 0 \\ 0 & 1 & 1 & 0 & 0 \end{pmatrix}$ | -1 |
| 12. | $x^3y^2$    | $s_4s_3s_4s_1s_4$ | $\begin{pmatrix} 0 & 0 & 1 & 0 & 1 \\ 1 & 1 & 1 & 0 & 0 \\ 1 & 1 & 1 & 0 & 1 \\ 1 & 1 & 1 & 1 & 1 \\ 1 & 0 & 0 & 0 & 1 \end{pmatrix}$ | 1  |
| 13. | $x^3y^2xy$  | $s_1s_1s_4s_2s_4$ | $\begin{pmatrix} 0 & 0 & 1 & 0 & 1 \\ 0 & 0 & 1 & 0 & 0 \\ 0 & 0 & 1 & 1 & 1 \\ 1 & 0 & 0 & 0 & 1 \\ 0 & 1 & 1 & 0 & 1 \end{pmatrix}$ | 1  |
| 14. | $(yx)^2y^2$ | $s_3s_1s_3s_2s_2$ | $\begin{pmatrix} 0 & 1 & 1 & 0 & 0 \\ 1 & 0 & 1 & 0 & 0 \\ 1 & 0 & 0 & 0 & 0 \\ 0 & 0 & 1 & 1 & 0 \\ 1 & 0 & 0 & 0 & 1 \end{pmatrix}$ | 1  |
| 15. | $x^3(xy)^2$ | $s_3s_2s_3s_1s_3$ | $\begin{pmatrix} 1 & 1 & 0 & 0 & 1 \\ 0 & 0 & 1 & 0 & 0 \\ 1 & 0 & 0 & 1 & 1 \\ 0 & 0 & 1 & 0 & 1 \\ 1 & 0 & 1 & 0 & 0 \end{pmatrix}$ | 1  |
| 16. | $x^4yx$     | $s_3s_2s_3s_4s_1$ | $\begin{pmatrix} 0 & 0 & 1 & 1 & 1 \\ 0 & 0 & 1 & 1 & 0 \\ 1 & 1 & 0 & 0 & 0 \\ 1 & 0 & 0 & 1 & 0 \\ 1 & 0 & 1 & 1 & 0 \end{pmatrix}$ | 1  |
| 17. | $(yx)^2y$   | $s_3s_1s_4s_3s_2$ | $\begin{pmatrix} 0 & 0 & 1 & 0 & 0 \\ 1 & 0 & 1 & 1 & 0 \\ 0 & 1 & 1 & 1 & 0 \\ 1 & 0 & 0 & 0 & 0 \\ 1 & 0 & 1 & 1 & 1 \end{pmatrix}$ | -1 |

|     |              |                   |                                                                                                                                       |    |
|-----|--------------|-------------------|---------------------------------------------------------------------------------------------------------------------------------------|----|
| 18. | $x^3y^2x$    | $s_1s_1s_1s_1s_4$ | $\begin{pmatrix} 1 & 0 & 0 & 0 & 1 \\ 0 & 0 & 1 & 0 & 0 \\ 0 & 0 & 0 & 0 & 1 \\ 0 & 0 & 0 & 1 & 1 \\ 0 & 1 & 0 & 0 & 1 \end{pmatrix}$ | 1  |
| 19. | $x$          | $s_3s_1s_1s_4s_1$ | $\begin{pmatrix} 1 & 0 & 0 & 1 & 1 \\ 0 & 0 & 0 & 1 & 0 \\ 0 & 1 & 0 & 0 & 0 \\ 1 & 0 & 0 & 1 & 0 \\ 1 & 0 & 1 & 1 & 0 \end{pmatrix}$ | 1  |
| 20. | $xy^2$       | $s_4s_1s_4s_1s_4$ | $\begin{pmatrix} 1 & 0 & 1 & 0 & 1 \\ 1 & 0 & 1 & 0 & 0 \\ 1 & 1 & 1 & 0 & 1 \\ 0 & 0 & 1 & 1 & 1 \\ 1 & 0 & 0 & 0 & 1 \end{pmatrix}$ | 1  |
| 21. | $xy$         | $s_1s_4s_3s_1s_3$ | $\begin{pmatrix} 0 & 1 & 0 & 0 & 1 \\ 1 & 1 & 1 & 0 & 0 \\ 0 & 0 & 0 & 1 & 1 \\ 0 & 1 & 1 & 0 & 1 \\ 0 & 1 & 1 & 0 & 0 \end{pmatrix}$ | -1 |
| 22. | $y^2x^2$     | $s_4s_2s_4s_2s_3$ | $\begin{pmatrix} 0 & 0 & 1 & 0 & 1 \\ 1 & 0 & 1 & 1 & 0 \\ 1 & 0 & 0 & 0 & 1 \\ 1 & 0 & 1 & 0 & 1 \\ 1 & 1 & 1 & 0 & 0 \end{pmatrix}$ | 1  |
| 23. | $x^3(xy)^2y$ | $s_1s_3s_4s_2s_2$ | $\begin{pmatrix} 0 & 0 & 1 & 0 & 0 \\ 0 & 1 & 1 & 0 & 0 \\ 1 & 1 & 1 & 0 & 0 \\ 0 & 1 & 1 & 1 & 0 \\ 0 & 0 & 0 & 0 & 1 \end{pmatrix}$ | -1 |
| 24. | $(yx)^2$     | $s_1s_4s_1s_3s_1$ | $\begin{pmatrix} 0 & 1 & 0 & 0 & 1 \\ 0 & 0 & 0 & 1 & 0 \\ 1 & 1 & 0 & 0 & 0 \\ 0 & 1 & 1 & 1 & 0 \\ 0 & 1 & 0 & 1 & 0 \end{pmatrix}$ | 1  |
| 25. | $x^4y^2x$    | $s_3s_4s_1s_1s_3$ | $\begin{pmatrix} 1 & 1 & 0 & 0 & 1 \\ 0 & 1 & 0 & 0 & 0 \\ 1 & 1 & 0 & 1 & 1 \\ 0 & 0 & 0 & 0 & 1 \\ 1 & 1 & 1 & 0 & 0 \end{pmatrix}$ | 1  |
| 26. | $x^3y$       | $s_3s_1s_4s_1s_4$ | $\begin{pmatrix} 1 & 0 & 1 & 0 & 1 \\ 1 & 0 & 1 & 0 & 0 \\ 0 & 1 & 1 & 0 & 1 \\ 0 & 0 & 1 & 1 & 1 \\ 1 & 0 & 0 & 0 & 1 \end{pmatrix}$ | 1  |
| 27. | $x^4$        | $s_3s_4s_3s_4s_1$ | $\begin{pmatrix} 1 & 1 & 1 & 1 & 1 \\ 1 & 1 & 1 & 1 & 0 \\ 1 & 1 & 0 & 0 & 0 \\ 0 & 0 & 0 & 1 & 0 \\ 0 & 1 & 1 & 1 & 0 \end{pmatrix}$ | -1 |

|     |              |                   |                                                                                                                                       |    |
|-----|--------------|-------------------|---------------------------------------------------------------------------------------------------------------------------------------|----|
| 28. | $x^2(xy)^2y$ | $s_3s_2s_4s_2s_4$ | $\begin{pmatrix} 1 & 0 & 1 & 0 & 1 \\ 1 & 1 & 1 & 0 & 0 \\ 0 & 0 & 1 & 1 & 1 \\ 1 & 0 & 0 & 0 & 1 \\ 0 & 0 & 1 & 0 & 1 \end{pmatrix}$ | 1  |
| 29. | $x^2y^2xy$   | $s_3s_1s_3s_1s_3$ | $\begin{pmatrix} 1 & 0 & 0 & 0 & 1 \\ 1 & 0 & 1 & 0 & 0 \\ 1 & 0 & 0 & 1 & 1 \\ 0 & 1 & 1 & 0 & 1 \\ 0 & 0 & 1 & 0 & 0 \end{pmatrix}$ | 1  |
| 30. | $y^2$        | $s_4s_2s_4s_2s_2$ | $\begin{pmatrix} 1 & 1 & 1 & 0 & 0 \\ 0 & 0 & 1 & 0 & 0 \\ 1 & 0 & 1 & 0 & 0 \\ 1 & 0 & 1 & 1 & 0 \\ 1 & 0 & 0 & 0 & 1 \end{pmatrix}$ | 1  |
| 31. | $x^2(xy)^2x$ | $s_3s_4s_1s_3s_1$ | $\begin{pmatrix} 1 & 1 & 0 & 0 & 1 \\ 0 & 0 & 0 & 1 & 0 \\ 1 & 1 & 0 & 0 & 0 \\ 1 & 1 & 1 & 1 & 0 \\ 0 & 1 & 0 & 1 & 0 \end{pmatrix}$ | 1  |
| 32. | $yx$         | $s_1s_3s_1s_4s_1$ | $\begin{pmatrix} 0 & 0 & 0 & 1 & 1 \\ 1 & 1 & 0 & 1 & 0 \\ 0 & 1 & 0 & 0 & 0 \\ 0 & 1 & 0 & 1 & 0 \\ 0 & 0 & 1 & 1 & 0 \end{pmatrix}$ | -1 |
| 33. | $x^2y^2x^2$  | $s_3s_4s_2s_3s_2$ | $\begin{pmatrix} 1 & 1 & 1 & 0 & 0 \\ 0 & 0 & 0 & 1 & 0 \\ 1 & 1 & 0 & 1 & 0 \\ 0 & 1 & 0 & 0 & 0 \\ 1 & 1 & 0 & 1 & 1 \end{pmatrix}$ | 1  |
| 34. | $x(xy)^3y$   | $s_3s_1s_4s_2s_2$ | $\begin{pmatrix} 1 & 0 & 1 & 0 & 0 \\ 0 & 1 & 1 & 0 & 0 \\ 0 & 0 & 1 & 0 & 0 \\ 1 & 0 & 1 & 1 & 0 \\ 1 & 0 & 0 & 0 & 1 \end{pmatrix}$ | 1  |
| 35. | $(xy)^3$     | $s_3s_1s_3s_4s_2$ | $\begin{pmatrix} 1 & 0 & 0 & 0 & 0 \\ 1 & 0 & 0 & 1 & 0 \\ 0 & 0 & 1 & 1 & 0 \\ 0 & 1 & 1 & 1 & 0 \\ 1 & 0 & 1 & 1 & 1 \end{pmatrix}$ | -1 |
| 36. | $x(xy)^2$    | $s_1s_3s_1s_1s_4$ | $\begin{pmatrix} 0 & 0 & 0 & 0 & 1 \\ 0 & 0 & 1 & 0 & 0 \\ 1 & 1 & 0 & 0 & 1 \\ 0 & 1 & 0 & 1 & 1 \\ 0 & 1 & 0 & 0 & 1 \end{pmatrix}$ | -1 |
| 37. | $x^2y^2$     | $s_4s_2s_2s_2s_2$ | $\begin{pmatrix} 1 & 0 & 0 & 0 & 0 \\ 1 & 1 & 0 & 0 & 0 \\ 0 & 0 & 1 & 0 & 0 \\ 1 & 0 & 0 & 1 & 0 \\ 1 & 0 & 0 & 0 & 1 \end{pmatrix}$ | 1  |

|     |              |                   |                                                                                                                                       |    |
|-----|--------------|-------------------|---------------------------------------------------------------------------------------------------------------------------------------|----|
| 38. | $x^3y^2x^2$  | $s_1s_4s_1s_4s_1$ | $\begin{pmatrix} 0 & 0 & 0 & 1 & 1 \\ 0 & 1 & 0 & 1 & 0 \\ 0 & 1 & 0 & 0 & 0 \\ 1 & 1 & 0 & 1 & 0 \\ 0 & 1 & 1 & 1 & 0 \end{pmatrix}$ | 1  |
| 39. | $(xy)^2y$    | $s_2s_3s_2s_4s_2$ | $\begin{pmatrix} 0 & 1 & 0 & 0 & 0 \\ 0 & 1 & 1 & 1 & 0 \\ 1 & 0 & 0 & 1 & 0 \\ 0 & 1 & 0 & 1 & 0 \\ 0 & 0 & 0 & 1 & 1 \end{pmatrix}$ | 1  |
| 40. | $x^3(xy)^3$  | $s_3s_2s_3s_2s_3$ | $\begin{pmatrix} 0 & 0 & 1 & 0 & 1 \\ 1 & 0 & 1 & 1 & 0 \\ 1 & 1 & 0 & 0 & 1 \\ 1 & 0 & 0 & 0 & 1 \\ 0 & 0 & 1 & 0 & 0 \end{pmatrix}$ | 1  |
| 41. | $x^3(xy)^2x$ | $s_4s_1s_3s_4s_2$ | $\begin{pmatrix} 1 & 0 & 0 & 0 & 0 \\ 1 & 0 & 0 & 1 & 0 \\ 0 & 0 & 1 & 1 & 0 \\ 1 & 1 & 1 & 1 & 0 \\ 1 & 0 & 1 & 1 & 1 \end{pmatrix}$ | -1 |
| 42. | $x^3(xy)^3y$ | $s_4s_2s_2s_4s_1$ | $\begin{pmatrix} 1 & 0 & 0 & 1 & 1 \\ 1 & 1 & 0 & 1 & 0 \\ 1 & 0 & 0 & 0 & 0 \\ 0 & 0 & 1 & 1 & 0 \\ 1 & 0 & 0 & 1 & 0 \end{pmatrix}$ | -1 |
| 43. | $(xy)^2$     | $s_3s_2s_4s_1s_1$ | $\begin{pmatrix} 0 & 0 & 1 & 0 & 1 \\ 1 & 0 & 1 & 1 & 0 \\ 0 & 0 & 1 & 0 & 0 \\ 1 & 0 & 0 & 0 & 0 \\ 1 & 1 & 1 & 0 & 0 \end{pmatrix}$ | -1 |
| 44. | $x^2y$       | $s_3s_4s_3s_4s_3$ | $\begin{pmatrix} 0 & 0 & 0 & 1 & 1 \\ 1 & 1 & 1 & 1 & 0 \\ 1 & 1 & 1 & 1 & 1 \\ 0 & 1 & 1 & 1 & 1 \\ 1 & 1 & 0 & 0 & 0 \end{pmatrix}$ | 1  |
| 45. | $xy^2xy$     | $s_1s_1s_3s_2s_4$ | $\begin{pmatrix} 1 & 0 & 0 & 0 & 1 \\ 0 & 1 & 1 & 0 & 0 \\ 0 & 0 & 1 & 1 & 1 \\ 0 & 0 & 0 & 0 & 1 \\ 0 & 0 & 1 & 0 & 1 \end{pmatrix}$ | 1  |
| 46. | $xy^2x$      | $s_3s_1s_1s_1s_4$ | $\begin{pmatrix} 1 & 0 & 0 & 0 & 1 \\ 1 & 0 & 1 & 0 & 0 \\ 0 & 0 & 0 & 0 & 1 \\ 1 & 0 & 0 & 1 & 1 \\ 0 & 1 & 0 & 0 & 1 \end{pmatrix}$ | 1  |
| 47. | $x^2$        | $s_3s_4s_2s_4s_2$ | $\begin{pmatrix} 0 & 1 & 0 & 0 & 0 \\ 1 & 1 & 1 & 1 & 0 \\ 0 & 0 & 0 & 1 & 0 \\ 1 & 1 & 0 & 1 & 0 \\ 1 & 1 & 0 & 1 & 1 \end{pmatrix}$ | -1 |



|     |             |                   |                                                                                                                                       |    |
|-----|-------------|-------------------|---------------------------------------------------------------------------------------------------------------------------------------|----|
| 48. | $xyx$       | $s_3s_1s_1s_3s_2$ | $\begin{pmatrix} 1 & 0 & 0 & 0 & 0 \\ 1 & 0 & 1 & 1 & 0 \\ 0 & 0 & 0 & 1 & 0 \\ 0 & 1 & 0 & 0 & 0 \\ 1 & 0 & 0 & 1 & 1 \end{pmatrix}$ | 1  |
| 49. | $(xy)^2x$   | $s_3s_4s_1s_3s_4$ | $\begin{pmatrix} 0 & 1 & 0 & 1 & 1 \\ 1 & 1 & 0 & 0 & 0 \\ 1 & 1 & 0 & 0 & 1 \\ 0 & 0 & 0 & 1 & 1 \\ 1 & 1 & 1 & 1 & 1 \end{pmatrix}$ | 1  |
| 50. | $x(xy)^3$   | $s_1s_1s_4s_3s_2$ | $\begin{pmatrix} 0 & 0 & 1 & 0 & 0 \\ 0 & 0 & 1 & 1 & 0 \\ 0 & 1 & 1 & 1 & 0 \\ 1 & 0 & 0 & 0 & 0 \\ 0 & 0 & 1 & 1 & 1 \end{pmatrix}$ | -1 |
| 51. | $x^2yx$     | $s_3s_2s_3s_4s_2$ | $\begin{pmatrix} 1 & 1 & 0 & 0 & 0 \\ 1 & 0 & 0 & 1 & 0 \\ 1 & 0 & 1 & 1 & 0 \\ 0 & 0 & 1 & 1 & 0 \\ 0 & 0 & 1 & 1 & 1 \end{pmatrix}$ | -1 |
| 52. | $y$         | $s_1s_1s_4s_1s_4$ | $\begin{pmatrix} 0 & 0 & 1 & 0 & 1 \\ 0 & 0 & 1 & 0 & 0 \\ 0 & 1 & 1 & 0 & 1 \\ 0 & 0 & 1 & 1 & 1 \\ 1 & 0 & 0 & 0 & 1 \end{pmatrix}$ | 1  |
| 53. | $x^2(xy)^2$ | $s_1s_4s_3s_2s_4$ | $\begin{pmatrix} 0 & 0 & 0 & 0 & 1 \\ 0 & 1 & 1 & 0 & 0 \\ 0 & 1 & 1 & 1 & 1 \\ 0 & 1 & 0 & 0 & 1 \\ 1 & 1 & 1 & 0 & 1 \end{pmatrix}$ | -1 |
| 54. | $x^2y^2x$   | $s_3s_2s_3s_1s_1$ | $\begin{pmatrix} 0 & 0 & 1 & 0 & 1 \\ 1 & 0 & 0 & 1 & 0 \\ 1 & 0 & 1 & 0 & 0 \\ 1 & 1 & 0 & 0 & 0 \\ 0 & 0 & 1 & 0 & 0 \end{pmatrix}$ | -1 |
| 55. | $x^4y^2$    | $s_2s_4s_2s_3s_2$ | $\begin{pmatrix} 0 & 1 & 1 & 0 & 0 \\ 0 & 0 & 0 & 1 & 0 \\ 0 & 1 & 0 & 1 & 0 \\ 1 & 1 & 0 & 0 & 0 \\ 0 & 1 & 0 & 1 & 1 \end{pmatrix}$ | -1 |
| 56. | $xy^2x^2$   | $s_3s_4s_1s_4s_1$ | $\begin{pmatrix} 0 & 0 & 0 & 1 & 1 \\ 0 & 1 & 0 & 1 & 0 \\ 1 & 1 & 0 & 0 & 0 \\ 1 & 1 & 0 & 1 & 0 \\ 1 & 1 & 1 & 1 & 0 \end{pmatrix}$ | 1  |
| 57. | $x^3$       | $s_3s_1s_1s_1s_1$ | $\begin{pmatrix} 0 & 0 & 0 & 0 & 1 \\ 1 & 0 & 0 & 1 & 0 \\ 1 & 0 & 1 & 0 & 0 \\ 0 & 1 & 0 & 0 & 0 \\ 1 & 0 & 0 & 0 & 0 \end{pmatrix}$ | 1  |

$$\begin{array}{llll}
58. & y^2xy & s_4s_3s_2s_3s_4 & \begin{pmatrix} 0 & 0 & 0 & 1 & 1 \\ 1 & 1 & 1 & 0 & 0 \\ 1 & 1 & 0 & 0 & 1 \\ 1 & 1 & 0 & 1 & 1 \\ 1 & 0 & 0 & 1 & 1 \end{pmatrix} & 1 \\
59. & yxy^2 & s_3s_2s_4s_2s_2 & \begin{pmatrix} 1 & 1 & 1 & 0 & 0 \\ 0 & 0 & 1 & 0 & 0 \\ 1 & 0 & 1 & 0 & 0 \\ 0 & 0 & 1 & 1 & 0 \\ 1 & 0 & 0 & 0 & 1 \end{pmatrix} & 1 \\
60. & x^2(xy)^3y & s_3s_2s_3s_2s_4 & \begin{pmatrix} 1 & 0 & 0 & 0 & 1 \\ 0 & 0 & 1 & 0 & 0 \\ 1 & 0 & 1 & 1 & 1 \\ 1 & 1 & 0 & 0 & 1 \\ 0 & 0 & 1 & 0 & 1 \end{pmatrix} & 1
\end{array}$$

## Solution for undirected graphs of diameter 6

|                               |                                                                                                                                                                           |
|-------------------------------|---------------------------------------------------------------------------------------------------------------------------------------------------------------------------|
| Diameter                      | 6                                                                                                                                                                         |
| Set size                      | 4                                                                                                                                                                         |
| Group $K$                     | $\mathbb{Z}_2 \times (\mathbb{Z}_{13} \rtimes \mathbb{Z}_3)$ (order 78; id 2)<br>$\langle x, y \mid x^{13}, y^6, x^{-1}yx^3y^{-1}, y^{-1}(x^{-1}y)^2x^{-1}y^{-1} \rangle$ |
| $\varphi : K \rightarrow S_6$ | $x \mapsto ()$<br>$y \mapsto (1\ 2\ 3\ 4\ 5\ 6)$                                                                                                                          |
| Set $S$                       | $\{s_1, s_2, s_3, s_4\} =$<br>$\{y^4, y^2, x^9y, x^{-1}y^5\}$                                                                                                             |
| Set $V$                       | $\{010111, 110101, 000001, 000010\}$                                                                                                                                      |

| No. | Element | Product              | Mapping matrix $M$                                                                                                                                                                 | $\det M$ |
|-----|---------|----------------------|------------------------------------------------------------------------------------------------------------------------------------------------------------------------------------|----------|
| 1.  | 1       | $s_3s_3s_3s_3s_3s_3$ | $\begin{pmatrix} 0 & 0 & 0 & 0 & 1 & 0 \\ 0 & 0 & 0 & 1 & 0 & 0 \\ 0 & 0 & 1 & 0 & 0 & 0 \\ 0 & 1 & 0 & 0 & 0 & 0 \\ 1 & 0 & 0 & 0 & 0 & 0 \\ 0 & 0 & 0 & 0 & 0 & 1 \end{pmatrix}$ | 1        |
| 2.  | $y^3$   | $s_1s_1s_1s_4s_4s_4$ | $\begin{pmatrix} 1 & 1 & 1 & 0 & 0 & 0 \\ 0 & 0 & 1 & 0 & 0 & 0 \\ 1 & 1 & 1 & 1 & 0 & 0 \\ 1 & 0 & 0 & 0 & 1 & 0 \\ 1 & 1 & 1 & 0 & 0 & 1 \\ 0 & 1 & 0 & 0 & 0 & 0 \end{pmatrix}$ | 1        |
| 3.  | $y^4$   | $s_3s_3s_2s_4s_2s_4$ | $\begin{pmatrix} 0 & 0 & 1 & 0 & 1 & 0 \\ 0 & 1 & 1 & 0 & 0 & 0 \\ 1 & 0 & 0 & 0 & 1 & 0 \\ 0 & 0 & 1 & 0 & 0 & 0 \\ 0 & 0 & 0 & 0 & 1 & 1 \\ 0 & 0 & 1 & 1 & 1 & 0 \end{pmatrix}$ | 1        |
| 4.  | $x$     | $s_1s_4s_4s_4s_1s_3$ | $\begin{pmatrix} 1 & 0 & 0 & 0 & 1 & 0 \\ 1 & 1 & 0 & 0 & 0 & 0 \\ 0 & 0 & 1 & 0 & 1 & 0 \\ 1 & 0 & 0 & 1 & 0 & 0 \\ 0 & 0 & 0 & 0 & 1 & 0 \\ 1 & 0 & 0 & 0 & 1 & 1 \end{pmatrix}$ | 1        |
| 5.  | $y$     | $s_2s_3s_3s_3s_1s_1$ | $\begin{pmatrix} 1 & 0 & 0 & 0 & 0 & 0 \\ 0 & 0 & 0 & 1 & 1 & 1 \\ 1 & 0 & 1 & 0 & 1 & 0 \\ 0 & 1 & 0 & 0 & 1 & 1 \\ 1 & 0 & 0 & 0 & 0 & 1 \\ 1 & 0 & 0 & 0 & 1 & 1 \end{pmatrix}$ | 1        |
| 6.  | $xy^3$  | $s_1s_3s_3s_2s_4s_2$ | $\begin{pmatrix} 1 & 0 & 0 & 1 & 1 & 1 \\ 0 & 0 & 0 & 1 & 0 & 1 \\ 1 & 0 & 1 & 1 & 0 & 0 \\ 1 & 1 & 0 & 0 & 0 & 1 \\ 1 & 0 & 0 & 1 & 0 & 0 \\ 0 & 0 & 0 & 0 & 0 & 1 \end{pmatrix}$ | 1        |

|     |           |                           |                                                                                                                                                                                    |    |
|-----|-----------|---------------------------|------------------------------------------------------------------------------------------------------------------------------------------------------------------------------------|----|
| 7.  | $y^2$     | $s_3 s_1 s_3 s_1 s_4 s_4$ | $\begin{pmatrix} 1 & 1 & 0 & 0 & 0 & 0 \\ 0 & 1 & 1 & 1 & 0 & 0 \\ 0 & 1 & 0 & 1 & 0 & 0 \\ 0 & 0 & 0 & 1 & 1 & 0 \\ 0 & 1 & 0 & 0 & 0 & 1 \\ 0 & 0 & 0 & 1 & 0 & 0 \end{pmatrix}$ | -1 |
| 8.  | $x^9 y^4$ | $s_1 s_3 s_3 s_3 s_2 s_3$ | $\begin{pmatrix} 0 & 0 & 0 & 0 & 1 & 0 \\ 1 & 0 & 0 & 0 & 1 & 0 \\ 0 & 0 & 0 & 1 & 1 & 0 \\ 1 & 0 & 1 & 0 & 0 & 0 \\ 1 & 1 & 0 & 0 & 1 & 0 \\ 1 & 0 & 0 & 0 & 0 & 1 \end{pmatrix}$ | -1 |
| 9.  | $x^2$     | $s_1 s_1 s_3 s_1 s_1 s_3$ | $\begin{pmatrix} 1 & 0 & 0 & 1 & 1 & 0 \\ 1 & 1 & 0 & 0 & 0 & 0 \\ 0 & 1 & 1 & 1 & 1 & 0 \\ 1 & 1 & 0 & 1 & 0 & 0 \\ 0 & 0 & 0 & 1 & 1 & 0 \\ 1 & 1 & 0 & 0 & 1 & 1 \end{pmatrix}$ | 1  |
| 10. | $y^5$     | $s_2 s_2 s_4 s_4 s_4 s_1$ | $\begin{pmatrix} 1 & 1 & 1 & 0 & 0 & 0 \\ 0 & 1 & 0 & 1 & 0 & 1 \\ 1 & 1 & 0 & 0 & 1 & 0 \\ 1 & 0 & 0 & 0 & 0 & 1 \\ 1 & 1 & 0 & 0 & 0 & 1 \\ 0 & 0 & 0 & 0 & 0 & 1 \end{pmatrix}$ | 1  |
| 11. | $x^9 y$   | $s_1 s_3 s_1 s_3 s_1 s_4$ | $\begin{pmatrix} 1 & 0 & 0 & 0 & 1 & 0 \\ 1 & 1 & 1 & 0 & 0 & 0 \\ 1 & 0 & 1 & 1 & 1 & 0 \\ 0 & 0 & 1 & 0 & 1 & 0 \\ 1 & 0 & 0 & 0 & 1 & 1 \\ 0 & 0 & 1 & 0 & 0 & 0 \end{pmatrix}$ | -1 |
| 12. | $x^2 y^3$ | $s_2 s_3 s_1 s_1 s_4 s_4$ | $\begin{pmatrix} 1 & 0 & 1 & 0 & 0 & 0 \\ 1 & 0 & 1 & 1 & 0 & 0 \\ 1 & 0 & 0 & 1 & 0 & 0 \\ 0 & 0 & 1 & 1 & 1 & 0 \\ 1 & 0 & 0 & 0 & 0 & 1 \\ 0 & 1 & 1 & 1 & 0 & 0 \end{pmatrix}$ | 1  |
| 13. | $x^3 y^2$ | $s_1 s_4 s_1 s_1 s_1 s_4$ | $\begin{pmatrix} 0 & 0 & 1 & 1 & 1 & 0 \\ 1 & 0 & 0 & 1 & 0 & 0 \\ 1 & 0 & 1 & 1 & 1 & 0 \\ 1 & 1 & 0 & 0 & 1 & 0 \\ 0 & 0 & 1 & 1 & 1 & 1 \\ 1 & 0 & 1 & 0 & 0 & 0 \end{pmatrix}$ | 1  |
| 14. | $x^5 y^4$ | $s_1 s_1 s_1 s_3 s_2 s_3$ | $\begin{pmatrix} 0 & 1 & 0 & 0 & 1 & 0 \\ 1 & 1 & 1 & 0 & 1 & 0 \\ 0 & 0 & 1 & 1 & 1 & 0 \\ 1 & 1 & 1 & 0 & 0 & 0 \\ 1 & 0 & 0 & 0 & 1 & 0 \\ 1 & 1 & 1 & 0 & 0 & 1 \end{pmatrix}$ | -1 |

|     |           |                           |                                                                                                                                                                                    |    |
|-----|-----------|---------------------------|------------------------------------------------------------------------------------------------------------------------------------------------------------------------------------|----|
| 15. | $x^3$     | $s_1 s_3 s_1 s_4 s_4 s_4$ | $\begin{pmatrix} 1 & 1 & 1 & 0 & 0 & 0 \\ 1 & 0 & 1 & 0 & 0 & 0 \\ 0 & 0 & 1 & 1 & 0 & 0 \\ 1 & 0 & 0 & 0 & 1 & 0 \\ 0 & 0 & 1 & 0 & 0 & 1 \\ 1 & 0 & 0 & 0 & 0 & 0 \end{pmatrix}$ | -1 |
| 16. | $x^3 y^5$ | $s_1 s_4 s_4 s_4 s_4 s_4$ | $\begin{pmatrix} 1 & 1 & 0 & 0 & 0 & 0 \\ 0 & 0 & 1 & 0 & 0 & 0 \\ 1 & 0 & 0 & 1 & 0 & 0 \\ 0 & 0 & 0 & 0 & 1 & 0 \\ 1 & 0 & 0 & 0 & 0 & 1 \\ 1 & 0 & 0 & 0 & 0 & 0 \end{pmatrix}$ | -1 |
| 17. | $x^5 y$   | $s_1 s_3 s_3 s_2 s_3 s_1$ | $\begin{pmatrix} 1 & 0 & 1 & 1 & 0 & 0 \\ 1 & 1 & 0 & 0 & 0 & 1 \\ 1 & 0 & 0 & 1 & 0 & 0 \\ 0 & 0 & 0 & 0 & 1 & 1 \\ 1 & 0 & 0 & 1 & 0 & 1 \\ 0 & 0 & 0 & 1 & 0 & 1 \end{pmatrix}$ | -1 |
| 18. | $x^3 y^3$ | $s_3 s_1 s_4 s_1 s_4 s_2$ | $\begin{pmatrix} 0 & 0 & 0 & 1 & 1 & 1 \\ 1 & 1 & 0 & 0 & 0 & 1 \\ 0 & 1 & 0 & 1 & 0 & 0 \\ 0 & 1 & 1 & 0 & 0 & 1 \\ 0 & 0 & 0 & 1 & 0 & 0 \\ 0 & 1 & 0 & 1 & 0 & 1 \end{pmatrix}$ | 1  |
| 19. | $x^6 y^2$ | $s_2 s_4 s_1 s_1 s_3 s_1$ | $\begin{pmatrix} 1 & 0 & 1 & 1 & 0 & 0 \\ 1 & 0 & 1 & 0 & 0 & 1 \\ 0 & 0 & 1 & 1 & 0 & 0 \\ 1 & 0 & 0 & 1 & 1 & 1 \\ 0 & 0 & 1 & 1 & 0 & 1 \\ 1 & 1 & 0 & 0 & 0 & 1 \end{pmatrix}$ | 1  |
| 20. | $xy^4$    | $s_1 s_3 s_3 s_2 s_3 s_3$ | $\begin{pmatrix} 0 & 0 & 0 & 0 & 1 & 0 \\ 1 & 0 & 0 & 1 & 0 & 0 \\ 0 & 0 & 0 & 1 & 0 & 0 \\ 1 & 0 & 1 & 1 & 0 & 0 \\ 1 & 1 & 0 & 0 & 0 & 0 \\ 1 & 0 & 0 & 1 & 0 & 1 \end{pmatrix}$ | -1 |
| 21. | $x^4$     | $s_2 s_3 s_3 s_3 s_2 s_4$ | $\begin{pmatrix} 0 & 0 & 0 & 1 & 1 & 0 \\ 1 & 0 & 1 & 0 & 0 & 0 \\ 0 & 1 & 0 & 0 & 1 & 0 \\ 1 & 0 & 0 & 0 & 0 & 0 \\ 1 & 0 & 0 & 0 & 1 & 1 \\ 1 & 0 & 0 & 0 & 1 & 0 \end{pmatrix}$ | -1 |
| 22. | $x^6 y^5$ | $s_1 s_4 s_1 s_3 s_1 s_4$ | $\begin{pmatrix} 1 & 1 & 0 & 0 & 1 & 0 \\ 0 & 0 & 1 & 0 & 0 & 0 \\ 1 & 0 & 1 & 1 & 1 & 0 \\ 0 & 0 & 1 & 0 & 1 & 0 \\ 1 & 0 & 0 & 0 & 1 & 1 \\ 1 & 0 & 1 & 0 & 0 & 0 \end{pmatrix}$ | -1 |

|     |              |                           |                                                                                                                                                                                    |    |
|-----|--------------|---------------------------|------------------------------------------------------------------------------------------------------------------------------------------------------------------------------------|----|
| 23. | $xy$         | $s_1 s_4 s_1 s_1 s_3 s_3$ | $\begin{pmatrix} 1 & 0 & 0 & 1 & 1 & 0 \\ 1 & 0 & 1 & 1 & 0 & 0 \\ 1 & 1 & 0 & 0 & 0 & 0 \\ 0 & 0 & 1 & 1 & 0 & 0 \\ 1 & 0 & 1 & 0 & 0 & 0 \\ 0 & 0 & 1 & 1 & 0 & 1 \end{pmatrix}$ | -1 |
| 24. | $x^4 y^3$    | $s_1 s_3 s_3 s_3 s_3 s_3$ | $\begin{pmatrix} 1 & 0 & 0 & 0 & 1 & 0 \\ 0 & 0 & 0 & 1 & 0 & 0 \\ 1 & 0 & 1 & 0 & 0 & 0 \\ 1 & 1 & 0 & 0 & 0 & 0 \\ 1 & 0 & 0 & 0 & 0 & 0 \\ 0 & 0 & 0 & 0 & 0 & 1 \end{pmatrix}$ | 1  |
| 25. | $x^9 y^2$    | $s_2 s_3 s_3 s_2 s_3 s_3$ | $\begin{pmatrix} 1 & 0 & 0 & 0 & 1 & 0 \\ 1 & 0 & 0 & 1 & 0 & 0 \\ 0 & 0 & 0 & 1 & 0 & 0 \\ 1 & 0 & 1 & 1 & 0 & 0 \\ 0 & 1 & 0 & 0 & 0 & 0 \\ 1 & 0 & 0 & 1 & 0 & 1 \end{pmatrix}$ | -1 |
| 26. | $x^{-3} y^4$ | $s_1 s_1 s_4 s_4 s_4 s_4$ | $\begin{pmatrix} 0 & 1 & 0 & 0 & 0 & 0 \\ 1 & 1 & 1 & 0 & 0 & 0 \\ 0 & 0 & 0 & 1 & 0 & 0 \\ 1 & 1 & 0 & 0 & 1 & 0 \\ 1 & 0 & 0 & 0 & 0 & 1 \\ 1 & 1 & 0 & 0 & 0 & 0 \end{pmatrix}$ | -1 |
| 27. | $x^5$        | $s_1 s_1 s_3 s_2 s_2 s_4$ | $\begin{pmatrix} 1 & 0 & 0 & 1 & 1 & 0 \\ 1 & 1 & 0 & 1 & 0 & 0 \\ 0 & 1 & 1 & 1 & 1 & 0 \\ 1 & 1 & 0 & 0 & 0 & 0 \\ 0 & 0 & 0 & 1 & 1 & 1 \\ 1 & 1 & 0 & 0 & 1 & 0 \end{pmatrix}$ | 1  |
| 28. | $x^9 y^5$    | $s_1 s_1 s_1 s_3 s_2 s_2$ | $\begin{pmatrix} 1 & 1 & 1 & 0 & 0 & 1 \\ 0 & 1 & 0 & 0 & 1 & 1 \\ 1 & 1 & 1 & 0 & 1 & 0 \\ 0 & 0 & 1 & 1 & 1 & 1 \\ 1 & 1 & 1 & 0 & 0 & 0 \\ 1 & 0 & 0 & 0 & 1 & 1 \end{pmatrix}$ | 1  |
| 29. | $x^{-3} y$   | $s_1 s_1 s_4 s_1 s_1 s_1$ | $\begin{pmatrix} 1 & 1 & 0 & 1 & 0 & 0 \\ 1 & 0 & 0 & 1 & 1 & 1 \\ 1 & 1 & 0 & 0 & 1 & 0 \\ 0 & 1 & 0 & 1 & 1 & 1 \\ 1 & 1 & 1 & 0 & 0 & 1 \\ 0 & 0 & 0 & 1 & 1 & 1 \end{pmatrix}$ | -1 |
| 30. | $x^5 y^3$    | $s_3 s_1 s_1 s_4 s_4 s_2$ | $\begin{pmatrix} 0 & 0 & 0 & 0 & 1 & 1 \\ 1 & 1 & 1 & 0 & 0 & 1 \\ 0 & 1 & 0 & 0 & 0 & 0 \\ 0 & 1 & 1 & 0 & 0 & 1 \\ 0 & 0 & 1 & 0 & 0 & 0 \\ 0 & 1 & 1 & 1 & 0 & 1 \end{pmatrix}$ | 1  |

|     |             |                      |                                                                                                                                                                                    |    |
|-----|-------------|----------------------|------------------------------------------------------------------------------------------------------------------------------------------------------------------------------------|----|
| 31. | $x^{-1}y^2$ | $s_1s_3s_3s_3s_2s_4$ | $\begin{pmatrix} 0 & 0 & 0 & 1 & 1 & 0 \\ 1 & 0 & 1 & 0 & 0 & 0 \\ 1 & 1 & 0 & 0 & 1 & 0 \\ 1 & 0 & 0 & 0 & 0 & 0 \\ 0 & 0 & 0 & 0 & 1 & 1 \\ 1 & 0 & 0 & 0 & 1 & 0 \end{pmatrix}$ | -1 |
| 32. | $x^6y^4$    | $s_1s_1s_4s_1s_1s_3$ | $\begin{pmatrix} 0 & 1 & 0 & 1 & 1 & 0 \\ 1 & 1 & 1 & 0 & 0 & 0 \\ 0 & 0 & 0 & 1 & 1 & 0 \\ 1 & 1 & 0 & 1 & 0 & 0 \\ 1 & 0 & 0 & 1 & 1 & 0 \\ 1 & 1 & 0 & 0 & 1 & 1 \end{pmatrix}$ | -1 |
| 33. | $x^6$       | $s_1s_3s_1s_1s_3s_1$ | $\begin{pmatrix} 1 & 1 & 1 & 1 & 0 & 0 \\ 1 & 0 & 1 & 0 & 0 & 1 \\ 0 & 0 & 1 & 1 & 0 & 0 \\ 1 & 0 & 0 & 1 & 1 & 1 \\ 0 & 0 & 1 & 1 & 0 & 1 \\ 1 & 0 & 0 & 0 & 0 & 1 \end{pmatrix}$ | -1 |
| 34. | $x^{-1}y^5$ | $s_1s_4s_4s_1s_3s_1$ | $\begin{pmatrix} 1 & 1 & 0 & 1 & 0 & 0 \\ 0 & 0 & 1 & 0 & 0 & 1 \\ 1 & 0 & 0 & 1 & 0 & 0 \\ 0 & 0 & 0 & 1 & 1 & 1 \\ 1 & 0 & 0 & 1 & 0 & 1 \\ 1 & 0 & 0 & 0 & 0 & 1 \end{pmatrix}$ | -1 |
| 35. | $x^6y$      | $s_3s_1s_4s_4s_4s_4$ | $\begin{pmatrix} 0 & 1 & 0 & 0 & 0 & 0 \\ 0 & 1 & 1 & 0 & 0 & 0 \\ 0 & 0 & 0 & 1 & 0 & 0 \\ 0 & 1 & 0 & 0 & 1 & 0 \\ 0 & 0 & 0 & 0 & 0 & 1 \\ 1 & 1 & 0 & 0 & 0 & 0 \end{pmatrix}$ | -1 |
| 36. | $x^6y^3$    | $s_1s_3s_2s_4s_4s_1$ | $\begin{pmatrix} 1 & 0 & 0 & 0 & 0 & 0 \\ 0 & 0 & 1 & 1 & 0 & 1 \\ 1 & 0 & 1 & 0 & 1 & 0 \\ 1 & 1 & 1 & 0 & 0 & 1 \\ 1 & 0 & 0 & 0 & 0 & 1 \\ 0 & 0 & 1 & 0 & 0 & 1 \end{pmatrix}$ | -1 |
| 37. | $x^2y^2$    | $s_1s_1s_3s_2s_3s_2$ | $\begin{pmatrix} 0 & 0 & 0 & 1 & 0 & 1 \\ 1 & 1 & 0 & 0 & 1 & 1 \\ 1 & 0 & 0 & 1 & 0 & 0 \\ 1 & 1 & 0 & 1 & 0 & 1 \\ 0 & 1 & 1 & 1 & 0 & 0 \\ 1 & 1 & 0 & 0 & 0 & 1 \end{pmatrix}$ | 1  |
| 38. | $x^2y^4$    | $s_4s_1s_1s_3s_1s_1$ | $\begin{pmatrix} 0 & 1 & 1 & 0 & 0 & 0 \\ 0 & 0 & 1 & 1 & 1 & 1 \\ 0 & 1 & 1 & 0 & 1 & 0 \\ 1 & 0 & 0 & 0 & 1 & 1 \\ 0 & 1 & 1 & 0 & 0 & 1 \\ 0 & 1 & 0 & 0 & 1 & 1 \end{pmatrix}$ | -1 |

|     |              |                           |                                                                                                                                                                                    |    |
|-----|--------------|---------------------------|------------------------------------------------------------------------------------------------------------------------------------------------------------------------------------|----|
| 39. | $x^7$        | $s_1 s_4 s_2 s_2 s_3 s_1$ | $\begin{pmatrix} 1 & 0 & 1 & 1 & 0 & 0 \\ 1 & 1 & 1 & 0 & 0 & 1 \\ 0 & 0 & 1 & 1 & 0 & 0 \\ 1 & 0 & 0 & 0 & 1 & 1 \\ 0 & 0 & 1 & 1 & 0 & 1 \\ 1 & 0 & 0 & 1 & 0 & 1 \end{pmatrix}$ | 1  |
| 40. | $x^2 y^5$    | $s_3 s_2 s_3 s_1 s_4 s_1$ | $\begin{pmatrix} 0 & 0 & 1 & 1 & 0 & 0 \\ 0 & 1 & 0 & 1 & 0 & 1 \\ 0 & 1 & 0 & 1 & 1 & 0 \\ 1 & 1 & 0 & 0 & 0 & 1 \\ 0 & 0 & 0 & 1 & 0 & 1 \\ 0 & 1 & 0 & 0 & 0 & 1 \end{pmatrix}$ | -1 |
| 41. | $x^2 y$      | $s_1 s_4 s_2 s_3 s_2 s_4$ | $\begin{pmatrix} 1 & 0 & 0 & 1 & 1 & 0 \\ 1 & 0 & 1 & 0 & 0 & 0 \\ 1 & 1 & 1 & 0 & 1 & 0 \\ 0 & 0 & 1 & 0 & 0 & 0 \\ 1 & 0 & 0 & 0 & 1 & 1 \\ 0 & 0 & 1 & 0 & 1 & 0 \end{pmatrix}$ | 1  |
| 42. | $x^7 y^3$    | $s_1 s_3 s_1 s_1 s_3 s_3$ | $\begin{pmatrix} 1 & 0 & 0 & 1 & 1 & 0 \\ 0 & 0 & 1 & 1 & 0 & 0 \\ 1 & 0 & 0 & 0 & 0 & 0 \\ 1 & 1 & 1 & 1 & 0 & 0 \\ 1 & 0 & 1 & 0 & 0 & 0 \\ 0 & 0 & 1 & 1 & 0 & 1 \end{pmatrix}$ | -1 |
| 43. | $x^5 y^2$    | $s_1 s_4 s_1 s_1 s_3 s_2$ | $\begin{pmatrix} 0 & 0 & 1 & 1 & 0 & 1 \\ 1 & 0 & 0 & 1 & 1 & 1 \\ 1 & 0 & 1 & 1 & 0 & 0 \\ 1 & 1 & 0 & 0 & 0 & 1 \\ 0 & 0 & 1 & 1 & 0 & 0 \\ 1 & 0 & 1 & 0 & 0 & 1 \end{pmatrix}$ | 1  |
| 44. | $x^{-2} y^4$ | $s_2 s_4 s_2 s_2 s_3 s_1$ | $\begin{pmatrix} 0 & 0 & 1 & 1 & 0 & 0 \\ 1 & 1 & 1 & 0 & 0 & 1 \\ 1 & 0 & 1 & 1 & 0 & 0 \\ 1 & 0 & 0 & 0 & 1 & 1 \\ 0 & 0 & 1 & 1 & 0 & 1 \\ 1 & 0 & 0 & 1 & 0 & 1 \end{pmatrix}$ | -1 |
| 45. | $x^8$        | $s_2 s_2 s_4 s_2 s_2 s_4$ | $\begin{pmatrix} 0 & 0 & 0 & 1 & 1 & 0 \\ 1 & 1 & 1 & 1 & 0 & 0 \\ 0 & 1 & 0 & 1 & 1 & 0 \\ 1 & 1 & 0 & 0 & 0 & 0 \\ 1 & 0 & 0 & 1 & 1 & 1 \\ 1 & 1 & 0 & 0 & 1 & 0 \end{pmatrix}$ | -1 |
| 46. | $x^5 y^5$    | $s_1 s_3 s_2 s_3 s_1 s_4$ | $\begin{pmatrix} 1 & 0 & 0 & 0 & 1 & 0 \\ 0 & 0 & 1 & 0 & 0 & 0 \\ 1 & 0 & 0 & 1 & 1 & 0 \\ 0 & 0 & 1 & 0 & 1 & 0 \\ 1 & 0 & 1 & 0 & 1 & 1 \\ 1 & 1 & 1 & 0 & 0 & 0 \end{pmatrix}$ | 1  |



|     |           |                           |                                                                                                                                                                                    |    |
|-----|-----------|---------------------------|------------------------------------------------------------------------------------------------------------------------------------------------------------------------------------|----|
| 47. | $x^{-2}y$ | $s_1 s_1 s_3 s_2 s_3 s_3$ | $\begin{pmatrix} 1 & 1 & 0 & 0 & 1 & 0 \\ 1 & 0 & 0 & 1 & 0 & 0 \\ 1 & 1 & 0 & 1 & 0 & 0 \\ 0 & 1 & 1 & 1 & 0 & 0 \\ 1 & 1 & 0 & 0 & 0 & 0 \\ 0 & 0 & 0 & 1 & 0 & 1 \end{pmatrix}$ | -1 |
| 48. | $x^8 y^3$ | $s_1 s_3 s_3 s_2 s_2 s_4$ | $\begin{pmatrix} 1 & 0 & 0 & 1 & 1 & 0 \\ 0 & 0 & 0 & 1 & 0 & 0 \\ 1 & 0 & 1 & 1 & 1 & 0 \\ 1 & 1 & 0 & 0 & 0 & 0 \\ 1 & 0 & 0 & 1 & 1 & 1 \\ 0 & 0 & 0 & 0 & 1 & 0 \end{pmatrix}$ | 1  |
| 49. | $x^8 y^2$ | $s_1 s_4 s_2 s_2 s_4 s_2$ | $\begin{pmatrix} 0 & 0 & 1 & 1 & 1 & 1 \\ 1 & 0 & 0 & 1 & 0 & 1 \\ 1 & 0 & 1 & 1 & 0 & 0 \\ 1 & 1 & 1 & 0 & 0 & 1 \\ 0 & 0 & 1 & 1 & 0 & 0 \\ 1 & 0 & 0 & 0 & 0 & 1 \end{pmatrix}$ | -1 |
| 50. | $x^7 y^4$ | $s_1 s_1 s_4 s_2 s_2 s_4$ | $\begin{pmatrix} 0 & 1 & 0 & 1 & 1 & 0 \\ 1 & 1 & 1 & 1 & 0 & 0 \\ 0 & 0 & 0 & 1 & 1 & 0 \\ 1 & 1 & 0 & 0 & 0 & 0 \\ 1 & 0 & 0 & 1 & 1 & 1 \\ 1 & 1 & 0 & 0 & 1 & 0 \end{pmatrix}$ | 1  |
| 51. | $x^9$     | $s_3 s_1 s_4 s_4 s_4 s_1$ | $\begin{pmatrix} 0 & 1 & 1 & 0 & 0 & 0 \\ 0 & 0 & 0 & 1 & 0 & 1 \\ 0 & 1 & 0 & 0 & 1 & 0 \\ 0 & 0 & 0 & 0 & 0 & 1 \\ 1 & 1 & 0 & 0 & 0 & 1 \\ 0 & 1 & 0 & 0 & 0 & 1 \end{pmatrix}$ | 1  |
| 52. | $x^8 y^5$ | $s_3 s_3 s_3 s_3 s_2 s_4$ | $\begin{pmatrix} 0 & 0 & 0 & 1 & 1 & 0 \\ 0 & 0 & 1 & 0 & 0 & 0 \\ 0 & 1 & 0 & 0 & 1 & 0 \\ 1 & 0 & 0 & 0 & 0 & 0 \\ 0 & 0 & 0 & 0 & 1 & 1 \\ 0 & 0 & 0 & 0 & 1 & 0 \end{pmatrix}$ | -1 |
| 53. | $x^7 y$   | $s_1 s_3 s_2 s_3 s_3 s_1$ | $\begin{pmatrix} 1 & 0 & 1 & 0 & 0 & 0 \\ 1 & 1 & 1 & 0 & 0 & 1 \\ 1 & 0 & 0 & 0 & 0 & 0 \\ 0 & 0 & 1 & 0 & 1 & 1 \\ 1 & 0 & 0 & 1 & 0 & 1 \\ 0 & 0 & 1 & 0 & 0 & 1 \end{pmatrix}$ | 1  |
| 54. | $x^9 y^3$ | $s_1 s_1 s_1 s_3 s_1 s_1$ | $\begin{pmatrix} 1 & 1 & 1 & 0 & 0 & 0 \\ 0 & 0 & 1 & 1 & 1 & 1 \\ 1 & 1 & 1 & 0 & 1 & 0 \\ 1 & 0 & 0 & 0 & 1 & 1 \\ 1 & 1 & 1 & 0 & 0 & 1 \\ 0 & 1 & 0 & 0 & 1 & 1 \end{pmatrix}$ | -1 |

|     |             |                      |                                                                                                                                                                                    |    |
|-----|-------------|----------------------|------------------------------------------------------------------------------------------------------------------------------------------------------------------------------------|----|
| 55. | $x^{-2}y^2$ | $s_1s_1s_1s_4s_1s_4$ | $\begin{pmatrix} 0 & 0 & 1 & 0 & 1 & 0 \\ 1 & 1 & 1 & 1 & 0 & 0 \\ 1 & 0 & 0 & 0 & 1 & 0 \\ 1 & 1 & 1 & 0 & 1 & 0 \\ 0 & 1 & 0 & 0 & 1 & 1 \\ 1 & 1 & 1 & 0 & 0 & 0 \end{pmatrix}$ | 1  |
| 56. | $x^3y^4$    | $s_1s_3s_2s_3s_3s_3$ | $\begin{pmatrix} 0 & 0 & 1 & 0 & 1 & 0 \\ 1 & 0 & 0 & 1 & 0 & 0 \\ 0 & 0 & 1 & 0 & 0 & 0 \\ 1 & 0 & 1 & 0 & 0 & 0 \\ 1 & 1 & 1 & 0 & 0 & 0 \\ 1 & 0 & 0 & 0 & 0 & 1 \end{pmatrix}$ | -1 |
| 57. | $x^{-3}$    | $s_2s_4s_2s_3s_3s_3$ | $\begin{pmatrix} 0 & 0 & 1 & 0 & 1 & 0 \\ 1 & 0 & 0 & 1 & 0 & 0 \\ 0 & 0 & 1 & 0 & 0 & 0 \\ 1 & 1 & 1 & 0 & 0 & 0 \\ 1 & 0 & 1 & 0 & 0 & 0 \\ 1 & 0 & 0 & 0 & 0 & 1 \end{pmatrix}$ | 1  |
| 58. | $x^{-2}y^5$ | $s_2s_3s_2s_3s_3s_1$ | $\begin{pmatrix} 1 & 0 & 1 & 0 & 0 & 0 \\ 0 & 1 & 1 & 0 & 0 & 1 \\ 1 & 0 & 0 & 0 & 0 & 0 \\ 1 & 0 & 1 & 0 & 1 & 1 \\ 1 & 0 & 0 & 1 & 0 & 1 \\ 0 & 0 & 1 & 0 & 0 & 1 \end{pmatrix}$ | 1  |
| 59. | $x^3y$      | $s_1s_4s_1s_3s_1s_3$ | $\begin{pmatrix} 1 & 0 & 0 & 0 & 1 & 0 \\ 1 & 0 & 1 & 0 & 0 & 0 \\ 1 & 1 & 0 & 0 & 1 & 0 \\ 0 & 0 & 1 & 0 & 0 & 0 \\ 1 & 0 & 1 & 1 & 1 & 0 \\ 0 & 0 & 1 & 0 & 1 & 1 \end{pmatrix}$ | 1  |
| 60. | $x^{-3}y^3$ | $s_1s_3s_2s_3s_2s_4$ | $\begin{pmatrix} 1 & 0 & 0 & 1 & 1 & 0 \\ 0 & 0 & 1 & 0 & 0 & 0 \\ 1 & 0 & 1 & 0 & 1 & 0 \\ 1 & 1 & 1 & 0 & 0 & 0 \\ 1 & 0 & 0 & 0 & 1 & 1 \\ 0 & 0 & 1 & 0 & 1 & 0 \end{pmatrix}$ | 1  |
| 61. | $xy^2$      | $s_2s_3s_2s_3s_3s_3$ | $\begin{pmatrix} 1 & 0 & 1 & 0 & 1 & 0 \\ 1 & 0 & 0 & 1 & 0 & 0 \\ 0 & 0 & 1 & 0 & 0 & 0 \\ 1 & 0 & 1 & 0 & 0 & 0 \\ 0 & 1 & 1 & 0 & 0 & 0 \\ 1 & 0 & 0 & 0 & 0 & 1 \end{pmatrix}$ | -1 |
| 62. | $x^{-1}y^4$ | $s_1s_4s_4s_1s_4s_4$ | $\begin{pmatrix} 0 & 0 & 1 & 0 & 0 & 0 \\ 1 & 0 & 0 & 1 & 0 & 0 \\ 0 & 0 & 0 & 1 & 0 & 0 \\ 1 & 0 & 0 & 1 & 1 & 0 \\ 1 & 0 & 0 & 0 & 0 & 1 \\ 1 & 1 & 0 & 1 & 0 & 0 \end{pmatrix}$ | -1 |

|     |             |                           |                                                                                                                                                                                    |    |
|-----|-------------|---------------------------|------------------------------------------------------------------------------------------------------------------------------------------------------------------------------------|----|
| 63. | $x^{-2}$    | $s_1 s_1 s_4 s_2 s_2 s_3$ | $\begin{pmatrix} 1 & 0 & 0 & 1 & 1 & 0 \\ 1 & 1 & 0 & 0 & 1 & 0 \\ 0 & 1 & 0 & 1 & 1 & 0 \\ 1 & 1 & 1 & 1 & 0 & 0 \\ 0 & 0 & 0 & 1 & 1 & 0 \\ 1 & 1 & 0 & 0 & 0 & 1 \end{pmatrix}$ | -1 |
| 64. | $xy^5$      | $s_1 s_3 s_1 s_4 s_1 s_4$ | $\begin{pmatrix} 1 & 0 & 1 & 0 & 1 & 0 \\ 0 & 0 & 1 & 1 & 0 & 0 \\ 1 & 0 & 0 & 0 & 1 & 0 \\ 0 & 0 & 1 & 0 & 1 & 0 \\ 1 & 0 & 0 & 0 & 1 & 1 \\ 1 & 1 & 1 & 0 & 0 & 0 \end{pmatrix}$ | 1  |
| 65. | $x^{-1}y$   | $s_1 s_3 s_2 s_2 s_4 s_4$ | $\begin{pmatrix} 1 & 0 & 1 & 0 & 0 & 0 \\ 1 & 1 & 1 & 1 & 0 & 0 \\ 1 & 0 & 0 & 0 & 0 & 0 \\ 0 & 0 & 1 & 1 & 1 & 0 \\ 1 & 0 & 0 & 1 & 0 & 1 \\ 0 & 0 & 1 & 1 & 0 & 0 \end{pmatrix}$ | -1 |
| 66. | $x^{-2}y^3$ | $s_1 s_1 s_4 s_1 s_4 s_4$ | $\begin{pmatrix} 1 & 1 & 1 & 0 & 0 & 0 \\ 0 & 0 & 0 & 1 & 0 & 0 \\ 1 & 1 & 0 & 1 & 0 & 0 \\ 1 & 0 & 0 & 1 & 1 & 0 \\ 1 & 1 & 0 & 0 & 0 & 1 \\ 0 & 1 & 0 & 1 & 0 & 0 \end{pmatrix}$ | 1  |
| 67. | $x^4y^2$    | $s_1 s_4 s_2 s_3 s_3 s_3$ | $\begin{pmatrix} 0 & 0 & 1 & 0 & 1 & 0 \\ 1 & 0 & 0 & 1 & 0 & 0 \\ 1 & 0 & 1 & 0 & 0 & 0 \\ 1 & 1 & 1 & 0 & 0 & 0 \\ 0 & 0 & 1 & 0 & 0 & 0 \\ 1 & 0 & 0 & 0 & 0 & 1 \end{pmatrix}$ | -1 |
| 68. | $x^8y^4$    | $s_1 s_4 s_1 s_4 s_2 s_2$ | $\begin{pmatrix} 0 & 0 & 1 & 0 & 0 & 1 \\ 1 & 0 & 1 & 0 & 1 & 1 \\ 0 & 0 & 1 & 1 & 1 & 0 \\ 1 & 0 & 0 & 0 & 1 & 1 \\ 1 & 0 & 1 & 0 & 0 & 0 \\ 1 & 1 & 0 & 0 & 1 & 1 \end{pmatrix}$ | -1 |
| 69. | $x^{-1}$    | $s_3 s_2 s_4 s_2 s_3 s_3$ | $\begin{pmatrix} 0 & 1 & 0 & 0 & 1 & 0 \\ 0 & 0 & 0 & 1 & 0 & 0 \\ 0 & 1 & 1 & 1 & 0 & 0 \\ 0 & 1 & 0 & 1 & 0 & 0 \\ 1 & 1 & 0 & 0 & 0 & 0 \\ 0 & 0 & 0 & 1 & 0 & 1 \end{pmatrix}$ | 1  |
| 70. | $x^4y^5$    | $s_1 s_1 s_3 s_1 s_4 s_4$ | $\begin{pmatrix} 1 & 1 & 0 & 0 & 0 & 0 \\ 0 & 1 & 1 & 1 & 0 & 0 \\ 1 & 1 & 0 & 1 & 0 & 0 \\ 0 & 0 & 0 & 1 & 1 & 0 \\ 1 & 1 & 0 & 0 & 0 & 1 \\ 1 & 0 & 0 & 1 & 0 & 0 \end{pmatrix}$ | -1 |

|     |             |                      |                                                                                                                                                                                    |    |
|-----|-------------|----------------------|------------------------------------------------------------------------------------------------------------------------------------------------------------------------------------|----|
| 71. | $x^8y$      | $s_2s_3s_2s_4s_1s_4$ | $\begin{pmatrix} 1 & 0 & 0 & 0 & 1 & 0 \\ 0 & 0 & 1 & 1 & 0 & 0 \\ 1 & 0 & 1 & 0 & 1 & 0 \\ 0 & 1 & 1 & 0 & 1 & 0 \\ 1 & 0 & 0 & 0 & 1 & 1 \\ 1 & 0 & 1 & 0 & 0 & 0 \end{pmatrix}$ | -1 |
| 72. | $x^{-1}y^3$ | $s_1s_3s_1s_4s_4s_2$ | $\begin{pmatrix} 1 & 0 & 0 & 0 & 1 & 1 \\ 0 & 0 & 1 & 0 & 0 & 1 \\ 1 & 0 & 0 & 0 & 0 & 0 \\ 1 & 1 & 1 & 0 & 0 & 1 \\ 1 & 0 & 1 & 0 & 0 & 0 \\ 0 & 0 & 1 & 1 & 0 & 1 \end{pmatrix}$ | 1  |
| 73. | $x^7y^2$    | $s_2s_2s_4s_2s_2s_3$ | $\begin{pmatrix} 1 & 0 & 0 & 1 & 1 & 0 \\ 1 & 1 & 0 & 0 & 1 & 0 \\ 0 & 0 & 0 & 1 & 1 & 0 \\ 1 & 1 & 1 & 1 & 0 & 0 \\ 0 & 1 & 0 & 1 & 1 & 0 \\ 1 & 1 & 0 & 0 & 0 & 1 \end{pmatrix}$ | 1  |
| 74. | $x^4y^4$    | $s_1s_4s_1s_4s_4s_4$ | $\begin{pmatrix} 0 & 0 & 1 & 0 & 0 & 0 \\ 1 & 0 & 1 & 0 & 0 & 0 \\ 0 & 0 & 1 & 1 & 0 & 0 \\ 1 & 0 & 0 & 0 & 1 & 0 \\ 1 & 0 & 1 & 0 & 0 & 1 \\ 1 & 1 & 0 & 0 & 0 & 0 \end{pmatrix}$ | -1 |
| 75. | $x^7y^5$    | $s_2s_2s_4s_1s_4s_4$ | $\begin{pmatrix} 1 & 1 & 1 & 0 & 0 & 0 \\ 0 & 1 & 0 & 1 & 0 & 0 \\ 1 & 1 & 0 & 1 & 0 & 0 \\ 1 & 0 & 0 & 1 & 1 & 0 \\ 1 & 1 & 0 & 0 & 0 & 1 \\ 0 & 0 & 0 & 1 & 0 & 0 \end{pmatrix}$ | -1 |
| 76. | $x^4y$      | $s_2s_3s_1s_4s_4s_2$ | $\begin{pmatrix} 1 & 0 & 0 & 0 & 1 & 1 \\ 0 & 0 & 1 & 0 & 0 & 1 \\ 1 & 0 & 0 & 0 & 0 & 0 \\ 0 & 1 & 1 & 0 & 0 & 1 \\ 1 & 0 & 1 & 0 & 0 & 0 \\ 1 & 0 & 1 & 1 & 0 & 1 \end{pmatrix}$ | 1  |
| 77. | $x^{-3}y^2$ | $s_2s_4s_4s_4s_4s_1$ | $\begin{pmatrix} 1 & 0 & 1 & 0 & 0 & 0 \\ 1 & 0 & 0 & 1 & 0 & 1 \\ 0 & 0 & 0 & 0 & 1 & 0 \\ 1 & 0 & 0 & 0 & 0 & 1 \\ 0 & 0 & 0 & 0 & 0 & 1 \\ 1 & 1 & 0 & 0 & 0 & 1 \end{pmatrix}$ | -1 |
| 78. | $x^{-3}y^5$ | $s_1s_4s_1s_3s_2s_3$ | $\begin{pmatrix} 1 & 1 & 0 & 0 & 1 & 0 \\ 0 & 0 & 1 & 0 & 1 & 0 \\ 1 & 0 & 1 & 1 & 1 & 0 \\ 0 & 0 & 1 & 0 & 0 & 0 \\ 1 & 0 & 0 & 0 & 1 & 0 \\ 1 & 0 & 1 & 0 & 0 & 1 \end{pmatrix}$ | -1 |

## Solution for undirected graphs of diameter 7

|                               |                                                                                                                                                             |
|-------------------------------|-------------------------------------------------------------------------------------------------------------------------------------------------------------|
| Diameter                      | 7                                                                                                                                                           |
| Set size                      | 4                                                                                                                                                           |
| Group $K$                     | $\mathbb{Z}_8 \times (\mathbb{Z}_7 \rtimes \mathbb{Z}_3)$ (order 168; id 2)<br>$\langle x, y \mid x^7, y^{24}, yx^{-2}y^{-1}x, x^{-1}y^{-1}x^{-3}y \rangle$ |
| $\varphi : K \rightarrow S_7$ | $x \mapsto (1\ 2\ 4\ 3\ 6\ 5\ 7)$<br>$y \mapsto (1\ 2\ 3)(4\ 5\ 6)$                                                                                         |
| Set $S$                       | $\{s_1, s_2, s_3, s_4\} =$<br>$\{y^{-8}, y^8, x^4y, x^6y^{-1}\}$                                                                                            |
| Set $V$                       | $\{1000101, 0011001, 0010001, 0001010\}$                                                                                                                    |

| No. | Element  | Product                 | Mapping matrix $M$                                                                                                                                                                                                                      | $\det M$ |
|-----|----------|-------------------------|-----------------------------------------------------------------------------------------------------------------------------------------------------------------------------------------------------------------------------------------|----------|
| 1.  | 1        | $s_1s_3s_1s_3s_1s_4s_4$ | $\begin{pmatrix} 0 & 0 & 0 & 1 & 1 & 1 & 0 \\ 0 & 0 & 0 & 0 & 0 & 1 & 0 \\ 1 & 0 & 1 & 0 & 0 & 0 & 0 \\ 1 & 0 & 0 & 1 & 1 & 0 & 1 \\ 0 & 1 & 1 & 0 & 1 & 0 & 0 \\ 0 & 1 & 1 & 0 & 0 & 0 & 1 \\ 1 & 0 & 0 & 0 & 0 & 0 & 0 \end{pmatrix}$ | -1       |
| 2.  | $y^9$    | $s_1s_1s_3s_2s_4s_1s_3$ | $\begin{pmatrix} 0 & 0 & 0 & 0 & 0 & 1 & 0 \\ 0 & 1 & 0 & 0 & 0 & 0 & 0 \\ 1 & 0 & 0 & 0 & 0 & 0 & 1 \\ 1 & 0 & 1 & 0 & 0 & 1 & 0 \\ 0 & 0 & 1 & 1 & 1 & 1 & 0 \\ 0 & 1 & 0 & 1 & 0 & 0 & 0 \\ 1 & 1 & 0 & 1 & 1 & 0 & 1 \end{pmatrix}$ | 1        |
| 3.  | $y^{-8}$ | $s_2s_3s_1s_3s_1s_4s_4$ | $\begin{pmatrix} 0 & 0 & 0 & 1 & 1 & 1 & 0 \\ 1 & 0 & 0 & 0 & 0 & 1 & 0 \\ 0 & 0 & 1 & 0 & 0 & 0 & 0 \\ 0 & 0 & 0 & 1 & 1 & 0 & 1 \\ 0 & 1 & 1 & 0 & 1 & 0 & 0 \\ 1 & 1 & 1 & 0 & 0 & 0 & 1 \\ 1 & 0 & 0 & 0 & 0 & 0 & 0 \end{pmatrix}$ | -1       |
| 4.  | $y^{-6}$ | $s_1s_3s_3s_1s_4s_2s_3$ | $\begin{pmatrix} 0 & 0 & 1 & 1 & 0 & 1 & 0 \\ 0 & 0 & 0 & 0 & 0 & 1 & 0 \\ 1 & 0 & 1 & 1 & 1 & 0 & 1 \\ 1 & 0 & 0 & 0 & 0 & 0 & 0 \\ 0 & 1 & 0 & 0 & 1 & 0 & 0 \\ 0 & 1 & 0 & 0 & 0 & 0 & 0 \\ 1 & 0 & 0 & 1 & 0 & 1 & 1 \end{pmatrix}$ | 1        |
| 5.  | $y^{12}$ | $s_1s_3s_2s_3s_2s_3s_3$ | $\begin{pmatrix} 0 & 0 & 0 & 0 & 1 & 1 & 0 \\ 0 & 0 & 0 & 0 & 0 & 1 & 0 \\ 1 & 0 & 0 & 1 & 0 & 0 & 1 \\ 1 & 0 & 1 & 1 & 1 & 0 & 0 \\ 0 & 1 & 0 & 0 & 0 & 0 & 0 \\ 0 & 1 & 1 & 0 & 1 & 0 & 0 \\ 1 & 0 & 1 & 0 & 0 & 0 & 1 \end{pmatrix}$ | -1       |

|     |          |                               |                                                                                                                                                                                                                                         |    |
|-----|----------|-------------------------------|-----------------------------------------------------------------------------------------------------------------------------------------------------------------------------------------------------------------------------------------|----|
| 6.  | $x$      | $s_1 s_1 s_1 s_4 s_2 s_3 s_1$ | $\begin{pmatrix} 1 & 1 & 1 & 1 & 0 & 1 & 1 \\ 0 & 0 & 1 & 0 & 1 & 0 & 0 \\ 1 & 0 & 0 & 0 & 1 & 0 & 0 \\ 0 & 1 & 0 & 0 & 0 & 0 & 0 \\ 0 & 1 & 0 & 0 & 0 & 0 & 1 \\ 1 & 0 & 0 & 1 & 0 & 0 & 0 \\ 0 & 0 & 1 & 0 & 1 & 1 & 1 \end{pmatrix}$ | -1 |
| 7.  | $y$      | $s_2 s_3 s_1 s_1 s_3 s_2 s_4$ | $\begin{pmatrix} 0 & 0 & 0 & 1 & 0 & 1 & 0 \\ 1 & 0 & 0 & 1 & 0 & 0 & 0 \\ 0 & 0 & 1 & 0 & 1 & 0 & 0 \\ 0 & 0 & 0 & 0 & 1 & 1 & 1 \\ 0 & 1 & 1 & 0 & 0 & 0 & 0 \\ 1 & 1 & 1 & 1 & 0 & 1 & 1 \\ 1 & 0 & 0 & 0 & 0 & 0 & 0 \end{pmatrix}$ | 1  |
| 8.  | $y^3$    | $s_1 s_3 s_1 s_3 s_2 s_2 s_3$ | $\begin{pmatrix} 0 & 0 & 0 & 1 & 1 & 1 & 0 \\ 0 & 0 & 0 & 0 & 0 & 1 & 0 \\ 1 & 0 & 1 & 0 & 1 & 0 & 1 \\ 1 & 0 & 0 & 1 & 0 & 0 & 0 \\ 0 & 1 & 1 & 0 & 0 & 0 & 0 \\ 0 & 1 & 1 & 0 & 1 & 0 & 0 \\ 1 & 0 & 0 & 0 & 0 & 1 & 1 \end{pmatrix}$ | -1 |
| 9.  | $y^{-3}$ | $s_1 s_1 s_4 s_2 s_4 s_2 s_4$ | $\begin{pmatrix} 0 & 0 & 1 & 0 & 0 & 1 & 0 \\ 0 & 1 & 0 & 1 & 1 & 0 & 0 \\ 1 & 0 & 0 & 0 & 0 & 0 & 0 \\ 1 & 0 & 0 & 0 & 0 & 1 & 1 \\ 0 & 0 & 0 & 1 & 1 & 0 & 0 \\ 0 & 1 & 0 & 1 & 0 & 1 & 1 \\ 1 & 1 & 1 & 0 & 0 & 0 & 0 \end{pmatrix}$ | 1  |
| 10. | $xy^9$   | $s_2 s_2 s_4 s_2 s_3 s_3 s_2$ | $\begin{pmatrix} 1 & 1 & 1 & 0 & 1 & 0 & 0 \\ 1 & 0 & 0 & 0 & 0 & 1 & 0 \\ 0 & 0 & 0 & 1 & 1 & 0 & 1 \\ 0 & 1 & 1 & 0 & 0 & 0 & 1 \\ 0 & 1 & 0 & 1 & 0 & 0 & 0 \\ 0 & 0 & 0 & 1 & 0 & 0 & 0 \\ 1 & 0 & 0 & 0 & 0 & 1 & 1 \end{pmatrix}$ | 1  |
| 11. | $y^8$    | $s_1 s_3 s_3 s_2 s_4 s_2 s_4$ | $\begin{pmatrix} 0 & 0 & 0 & 0 & 0 & 1 & 0 \\ 1 & 0 & 1 & 1 & 1 & 0 & 0 \\ 0 & 0 & 1 & 0 & 0 & 0 & 0 \\ 0 & 1 & 0 & 0 & 0 & 1 & 1 \\ 0 & 1 & 0 & 1 & 1 & 0 & 0 \\ 1 & 0 & 0 & 1 & 0 & 1 & 1 \\ 1 & 0 & 0 & 0 & 0 & 0 & 0 \end{pmatrix}$ | 1  |
| 12. | $y^{10}$ | $s_2 s_3 s_3 s_2 s_3 s_1 s_4$ | $\begin{pmatrix} 0 & 0 & 1 & 0 & 0 & 0 & 0 \\ 1 & 0 & 0 & 0 & 0 & 0 & 0 \\ 0 & 0 & 1 & 1 & 0 & 0 & 0 \\ 0 & 0 & 0 & 1 & 1 & 1 & 1 \\ 0 & 1 & 0 & 0 & 0 & 1 & 0 \\ 1 & 1 & 0 & 1 & 0 & 0 & 1 \\ 1 & 0 & 0 & 0 & 1 & 1 & 0 \end{pmatrix}$ | 1  |

|     |              |                               |                                                                                                                                                                                                                                         |      |
|-----|--------------|-------------------------------|-----------------------------------------------------------------------------------------------------------------------------------------------------------------------------------------------------------------------------------------|------|
| 13. | $y^4$        | $s_2 s_4 s_1 s_4 s_2 s_4 s_4$ | $\begin{pmatrix} 0 & 0 & 1 & 0 & 1 & 1 & 0 \\ 1 & 1 & 0 & 0 & 1 & 1 & 0 \\ 0 & 0 & 1 & 1 & 0 & 0 & 0 \\ 0 & 0 & 0 & 0 & 0 & 0 & 1 \\ 0 & 0 & 0 & 1 & 0 & 0 & 0 \\ 1 & 0 & 0 & 0 & 0 & 0 & 1 \\ 1 & 1 & 1 & 0 & 1 & 0 & 0 \end{pmatrix}$ | $-1$ |
| 14. | $x^4 y^{-8}$ | $s_1 s_1 s_3 s_2 s_2 s_4 s_1$ | $\begin{pmatrix} 1 & 1 & 0 & 1 & 0 & 0 & 1 \\ 1 & 0 & 0 & 0 & 1 & 0 & 0 \\ 0 & 1 & 0 & 1 & 0 & 0 & 0 \\ 0 & 0 & 0 & 0 & 1 & 1 & 0 \\ 0 & 0 & 1 & 1 & 1 & 1 & 1 \\ 0 & 1 & 0 & 0 & 0 & 0 & 0 \\ 1 & 0 & 1 & 0 & 0 & 0 & 1 \end{pmatrix}$ | $-1$ |
| 15. | $y^6$        | $s_1 s_3 s_2 s_4 s_4 s_2 s_4$ | $\begin{pmatrix} 0 & 0 & 0 & 0 & 0 & 1 & 0 \\ 0 & 0 & 0 & 0 & 1 & 0 & 0 \\ 1 & 0 & 0 & 0 & 0 & 0 & 0 \\ 1 & 0 & 1 & 0 & 0 & 1 & 1 \\ 0 & 1 & 0 & 0 & 1 & 0 & 0 \\ 0 & 1 & 1 & 1 & 0 & 1 & 1 \\ 1 & 0 & 1 & 1 & 0 & 0 & 0 \end{pmatrix}$ | $-1$ |
| 16. | $xy^{-6}$    | $s_1 s_1 s_1 s_3 s_2 s_3 s_2$ | $\begin{pmatrix} 1 & 1 & 1 & 0 & 1 & 0 & 0 \\ 0 & 0 & 1 & 0 & 0 & 1 & 0 \\ 1 & 0 & 0 & 1 & 1 & 0 & 1 \\ 0 & 1 & 0 & 0 & 0 & 0 & 1 \\ 0 & 1 & 0 & 1 & 0 & 0 & 0 \\ 1 & 0 & 0 & 0 & 0 & 0 & 0 \\ 0 & 0 & 1 & 0 & 1 & 1 & 1 \end{pmatrix}$ | $1$  |
| 17. | $xy^{12}$    | $s_1 s_3 s_3 s_2 s_3 s_3 s_2$ | $\begin{pmatrix} 1 & 0 & 0 & 0 & 1 & 0 & 0 \\ 0 & 0 & 1 & 0 & 0 & 1 & 0 \\ 1 & 0 & 0 & 1 & 1 & 0 & 1 \\ 0 & 0 & 0 & 0 & 0 & 0 & 1 \\ 0 & 1 & 0 & 1 & 0 & 0 & 0 \\ 1 & 0 & 1 & 1 & 0 & 0 & 0 \\ 0 & 1 & 0 & 0 & 0 & 1 & 1 \end{pmatrix}$ | $1$  |
| 18. | $x^2$        | $s_1 s_1 s_4 s_2 s_3 s_1 s_1$ | $\begin{pmatrix} 0 & 0 & 0 & 1 & 0 & 0 & 1 \\ 1 & 1 & 1 & 0 & 1 & 1 & 0 \\ 0 & 1 & 0 & 1 & 0 & 0 & 0 \\ 0 & 0 & 1 & 0 & 0 & 0 & 0 \\ 1 & 0 & 0 & 0 & 0 & 0 & 1 \\ 1 & 0 & 0 & 0 & 0 & 1 & 0 \\ 0 & 1 & 0 & 1 & 1 & 1 & 1 \end{pmatrix}$ | $1$  |
| 19. | $y^{-7}$     | $s_1 s_3 s_2 s_4 s_2 s_2 s_3$ | $\begin{pmatrix} 0 & 0 & 0 & 0 & 1 & 1 & 0 \\ 1 & 0 & 0 & 0 & 0 & 1 & 0 \\ 0 & 0 & 0 & 0 & 1 & 0 & 1 \\ 0 & 1 & 0 & 0 & 0 & 0 & 0 \\ 0 & 1 & 1 & 1 & 0 & 0 & 0 \\ 1 & 0 & 1 & 0 & 1 & 0 & 0 \\ 1 & 0 & 1 & 1 & 0 & 1 & 1 \end{pmatrix}$ | $-1$ |

|     |           |                               |                                                                                                                                                                                                                                         |    |
|-----|-----------|-------------------------------|-----------------------------------------------------------------------------------------------------------------------------------------------------------------------------------------------------------------------------------------|----|
| 20. | $y^{-5}$  | $s_1 s_3 s_1 s_1 s_3 s_3$     | $\begin{pmatrix} 1 & 0 & 1 & 0 & 0 & 1 & 0 \\ 0 & 0 & 0 & 1 & 0 & 1 & 0 \\ 0 & 0 & 0 & 1 & 0 & 0 & 1 \\ 0 & 1 & 1 & 1 & 1 & 0 & 0 \\ 1 & 0 & 0 & 0 & 1 & 0 & 0 \\ 0 & 1 & 1 & 0 & 0 & 0 & 0 \\ 1 & 0 & 0 & 0 & 1 & 0 & 1 \end{pmatrix}$ | 1  |
| 21. | $y^{13}$  | $s_1 s_4 s_1 s_1 s_4 s_4$     | $\begin{pmatrix} 1 & 0 & 1 & 1 & 1 & 1 & 0 \\ 0 & 0 & 1 & 0 & 0 & 1 & 0 \\ 0 & 1 & 0 & 1 & 0 & 0 & 0 \\ 0 & 0 & 0 & 0 & 1 & 0 & 1 \\ 1 & 0 & 0 & 0 & 1 & 0 & 0 \\ 0 & 0 & 0 & 1 & 0 & 0 & 1 \\ 1 & 1 & 1 & 0 & 0 & 0 & 0 \end{pmatrix}$ | -1 |
| 22. | $x^4 y$   | $s_1 s_1 s_3 s_3 s_2 s_4 s_2$ | $\begin{pmatrix} 1 & 1 & 0 & 0 & 0 & 0 & 0 \\ 1 & 0 & 0 & 1 & 0 & 0 & 0 \\ 0 & 1 & 0 & 0 & 1 & 0 & 1 \\ 0 & 0 & 0 & 0 & 0 & 0 & 1 \\ 0 & 0 & 1 & 0 & 1 & 1 & 0 \\ 0 & 1 & 0 & 1 & 1 & 1 & 0 \\ 1 & 0 & 1 & 0 & 0 & 0 & 1 \end{pmatrix}$ | -1 |
| 23. | $y^{-9}$  | $s_1 s_1 s_3 s_1 s_4 s_1 s_4$ | $\begin{pmatrix} 0 & 0 & 0 & 0 & 1 & 0 & 0 \\ 0 & 1 & 0 & 1 & 0 & 0 & 0 \\ 1 & 0 & 0 & 0 & 0 & 0 & 0 \\ 1 & 0 & 1 & 1 & 0 & 1 & 1 \\ 0 & 0 & 1 & 1 & 1 & 1 & 0 \\ 0 & 1 & 0 & 0 & 0 & 0 & 1 \\ 1 & 1 & 0 & 0 & 0 & 1 & 0 \end{pmatrix}$ | -1 |
| 24. | $xy^3$    | $s_1 s_3 s_2 s_2 s_3 s_3 s_1$ | $\begin{pmatrix} 1 & 0 & 1 & 0 & 0 & 1 & 1 \\ 0 & 0 & 0 & 1 & 1 & 0 & 0 \\ 1 & 0 & 1 & 0 & 1 & 0 & 0 \\ 0 & 0 & 0 & 1 & 0 & 0 & 0 \\ 0 & 1 & 1 & 1 & 0 & 0 & 1 \\ 1 & 0 & 0 & 0 & 0 & 0 & 0 \\ 0 & 1 & 0 & 0 & 0 & 1 & 1 \end{pmatrix}$ | -1 |
| 25. | $xy^{-3}$ | $s_1 s_4 s_4 s_1 s_4 s_2 s_2$ | $\begin{pmatrix} 1 & 1 & 0 & 0 & 0 & 0 & 0 \\ 0 & 0 & 1 & 0 & 0 & 1 & 0 \\ 1 & 0 & 0 & 0 & 0 & 0 & 1 \\ 0 & 1 & 0 & 0 & 1 & 0 & 1 \\ 0 & 0 & 0 & 1 & 1 & 0 & 0 \\ 1 & 0 & 1 & 1 & 0 & 1 & 0 \\ 0 & 0 & 0 & 1 & 0 & 1 & 1 \end{pmatrix}$ | 1  |
| 26. | $x^2 y^9$ | $s_1 s_1 s_1 s_3 s_3 s_2 s_4$ | $\begin{pmatrix} 0 & 0 & 1 & 0 & 0 & 1 & 0 \\ 1 & 1 & 1 & 0 & 0 & 0 & 0 \\ 0 & 1 & 0 & 0 & 1 & 0 & 0 \\ 0 & 0 & 1 & 0 & 1 & 1 & 1 \\ 1 & 0 & 0 & 0 & 0 & 0 & 0 \\ 1 & 0 & 0 & 1 & 0 & 1 & 1 \\ 0 & 1 & 0 & 1 & 0 & 0 & 0 \end{pmatrix}$ | -1 |



|     |              |                               |                                                                                                                                                                                                                                         |      |
|-----|--------------|-------------------------------|-----------------------------------------------------------------------------------------------------------------------------------------------------------------------------------------------------------------------------------------|------|
| 27. | $y^2$        | $s_1 s_3 s_1 s_4 s_1 s_3 s_3$ | $\begin{pmatrix} 0 & 0 & 0 & 1 & 0 & 1 & 0 \\ 1 & 0 & 1 & 0 & 0 & 1 & 0 \\ 0 & 0 & 0 & 0 & 0 & 0 & 1 \\ 0 & 1 & 1 & 0 & 1 & 0 & 0 \\ 0 & 1 & 1 & 1 & 1 & 0 & 0 \\ 1 & 0 & 0 & 0 & 0 & 0 & 0 \\ 1 & 0 & 0 & 0 & 1 & 0 & 1 \end{pmatrix}$ | $-1$ |
| 28. | $y^{-4}$     | $s_1 s_3 s_2 s_3 s_3 s_1 s_3$ | $\begin{pmatrix} 0 & 0 & 0 & 0 & 1 & 1 & 0 \\ 1 & 0 & 0 & 1 & 0 & 0 & 0 \\ 0 & 0 & 0 & 0 & 0 & 0 & 1 \\ 0 & 1 & 0 & 0 & 1 & 1 & 0 \\ 0 & 1 & 1 & 0 & 0 & 1 & 0 \\ 1 & 0 & 1 & 1 & 0 & 0 & 0 \\ 1 & 0 & 1 & 0 & 0 & 0 & 1 \end{pmatrix}$ | $-1$ |
| 29. | $x^2 y^8$    | $s_4 s_2 s_3 s_1 s_4 s_2 s_3$ | $\begin{pmatrix} 1 & 0 & 1 & 1 & 0 & 1 & 0 \\ 0 & 0 & 0 & 0 & 0 & 1 & 0 \\ 0 & 1 & 1 & 1 & 1 & 0 & 1 \\ 1 & 0 & 0 & 0 & 0 & 0 & 0 \\ 0 & 1 & 0 & 0 & 1 & 0 & 0 \\ 0 & 1 & 0 & 0 & 0 & 0 & 0 \\ 0 & 0 & 0 & 1 & 0 & 1 & 1 \end{pmatrix}$ | $1$  |
| 30. | $y^{-2}$     | $s_4 s_1 s_4 s_1 s_3 s_1 s_4$ | $\begin{pmatrix} 1 & 0 & 0 & 0 & 0 & 0 & 0 \\ 0 & 1 & 1 & 1 & 0 & 0 & 0 \\ 0 & 1 & 0 & 1 & 0 & 0 & 0 \\ 0 & 0 & 1 & 0 & 1 & 1 & 1 \\ 0 & 0 & 0 & 1 & 0 & 1 & 0 \\ 0 & 0 & 0 & 0 & 0 & 0 & 1 \\ 1 & 1 & 0 & 0 & 1 & 1 & 0 \end{pmatrix}$ | $-1$ |
| 31. | $x^4 y^{10}$ | $s_1 s_3 s_1 s_1 s_3 s_1 s_1$ | $\begin{pmatrix} 1 & 0 & 0 & 0 & 0 & 0 & 1 \\ 1 & 0 & 1 & 0 & 1 & 1 & 0 \\ 0 & 1 & 1 & 1 & 0 & 0 & 0 \\ 0 & 0 & 0 & 1 & 0 & 0 & 0 \\ 0 & 1 & 1 & 0 & 0 & 0 & 1 \\ 0 & 0 & 0 & 1 & 0 & 1 & 0 \\ 1 & 0 & 0 & 0 & 1 & 1 & 1 \end{pmatrix}$ | $1$  |
| 32. | $x^4 y^4$    | $s_2 s_4 s_4 s_2 s_4 s_1 s_4$ | $\begin{pmatrix} 1 & 1 & 0 & 1 & 1 & 0 & 0 \\ 0 & 0 & 1 & 0 & 0 & 0 & 0 \\ 0 & 0 & 0 & 1 & 0 & 0 & 0 \\ 1 & 1 & 0 & 0 & 0 & 1 & 1 \\ 1 & 0 & 0 & 1 & 1 & 1 & 0 \\ 0 & 0 & 1 & 0 & 0 & 0 & 1 \\ 0 & 0 & 0 & 0 & 0 & 1 & 0 \end{pmatrix}$ | $1$  |
| 33. | $xy^{-8}$    | $s_2 s_2 s_3 s_2 s_2 s_4 s_2$ | $\begin{pmatrix} 0 & 0 & 0 & 1 & 0 & 0 & 0 \\ 1 & 1 & 0 & 1 & 0 & 0 & 0 \\ 1 & 0 & 0 & 0 & 1 & 0 & 1 \\ 0 & 0 & 0 & 0 & 0 & 0 & 1 \\ 0 & 1 & 0 & 0 & 1 & 1 & 0 \\ 0 & 1 & 1 & 1 & 1 & 1 & 0 \\ 1 & 0 & 1 & 0 & 0 & 0 & 1 \end{pmatrix}$ | $1$  |

|     |             |                         |                                                                                                                                                                                                                                         |    |
|-----|-------------|-------------------------|-----------------------------------------------------------------------------------------------------------------------------------------------------------------------------------------------------------------------------------------|----|
| 34. | $xy^6$      | $s_2s_2s_4s_1s_1s_4s_2$ | $\begin{pmatrix} 1 & 1 & 1 & 1 & 0 & 0 & 0 \\ 1 & 0 & 0 & 1 & 0 & 0 & 0 \\ 0 & 0 & 0 & 0 & 0 & 0 & 1 \\ 0 & 1 & 1 & 0 & 1 & 0 & 1 \\ 0 & 1 & 0 & 0 & 0 & 1 & 0 \\ 0 & 0 & 0 & 1 & 1 & 1 & 0 \\ 1 & 0 & 0 & 0 & 1 & 0 & 1 \end{pmatrix}$ | 1  |
| 35. | $x^2y^{-6}$ | $s_1s_3s_3s_2s_4s_1s_3$ | $\begin{pmatrix} 0 & 1 & 0 & 0 & 0 & 1 & 0 \\ 1 & 0 & 0 & 0 & 0 & 0 & 0 \\ 0 & 0 & 0 & 0 & 0 & 0 & 1 \\ 0 & 0 & 1 & 0 & 0 & 1 & 0 \\ 1 & 0 & 1 & 1 & 1 & 1 & 0 \\ 1 & 0 & 0 & 1 & 0 & 0 & 0 \\ 0 & 1 & 0 & 1 & 1 & 0 & 1 \end{pmatrix}$ | -1 |
| 36. | $x^2y^{12}$ | $s_1s_3s_2s_3s_3s_3s_2$ | $\begin{pmatrix} 0 & 1 & 0 & 0 & 1 & 0 & 0 \\ 1 & 0 & 1 & 0 & 0 & 1 & 0 \\ 0 & 0 & 0 & 0 & 1 & 0 & 1 \\ 0 & 0 & 0 & 0 & 0 & 0 & 1 \\ 1 & 0 & 0 & 1 & 0 & 0 & 0 \\ 1 & 0 & 1 & 1 & 0 & 0 & 0 \\ 0 & 1 & 1 & 0 & 0 & 1 & 1 \end{pmatrix}$ | -1 |
| 37. | $x^3$       | $s_2s_3s_2s_3s_2s_4s_4$ | $\begin{pmatrix} 0 & 0 & 1 & 1 & 1 & 1 & 0 \\ 1 & 1 & 1 & 0 & 1 & 1 & 0 \\ 1 & 0 & 0 & 0 & 0 & 0 & 0 \\ 1 & 0 & 1 & 0 & 0 & 0 & 1 \\ 0 & 1 & 0 & 0 & 0 & 0 & 0 \\ 0 & 0 & 0 & 1 & 0 & 0 & 1 \\ 0 & 0 & 0 & 0 & 1 & 0 & 0 \end{pmatrix}$ | -1 |
| 38. | $y^{11}$    | $s_2s_3s_1s_1s_1s_3s_3$ | $\begin{pmatrix} 0 & 0 & 1 & 0 & 0 & 1 & 0 \\ 0 & 0 & 0 & 1 & 0 & 1 & 0 \\ 1 & 0 & 0 & 1 & 0 & 0 & 1 \\ 1 & 1 & 1 & 1 & 1 & 0 & 0 \\ 0 & 0 & 0 & 0 & 1 & 0 & 0 \\ 0 & 1 & 1 & 0 & 0 & 0 & 0 \\ 1 & 0 & 0 & 0 & 1 & 0 & 1 \end{pmatrix}$ | -1 |
| 39. | $y^5$       | $s_2s_2s_4s_2s_4s_2s_4$ | $\begin{pmatrix} 0 & 1 & 1 & 0 & 0 & 1 & 0 \\ 0 & 0 & 0 & 1 & 1 & 0 & 0 \\ 1 & 0 & 0 & 0 & 0 & 0 & 0 \\ 1 & 0 & 0 & 0 & 0 & 1 & 1 \\ 0 & 1 & 0 & 1 & 1 & 0 & 0 \\ 0 & 0 & 0 & 1 & 0 & 1 & 1 \\ 1 & 1 & 1 & 0 & 0 & 0 & 0 \end{pmatrix}$ | -1 |
| 40. | $x^2y^{-7}$ | $s_4s_2s_4s_2s_3s_3s_3$ | $\begin{pmatrix} 1 & 0 & 0 & 0 & 0 & 1 & 0 \\ 0 & 0 & 0 & 0 & 0 & 1 & 0 \\ 0 & 1 & 0 & 1 & 0 & 0 & 1 \\ 1 & 0 & 0 & 1 & 1 & 0 & 0 \\ 0 & 1 & 1 & 0 & 0 & 0 & 0 \\ 0 & 1 & 1 & 0 & 1 & 0 & 0 \\ 0 & 0 & 0 & 1 & 0 & 0 & 1 \end{pmatrix}$ | -1 |

|     |              |                               |                                                                                                                                                                                                                                         |    |
|-----|--------------|-------------------------------|-----------------------------------------------------------------------------------------------------------------------------------------------------------------------------------------------------------------------------------------|----|
| 41. | $y^7$        | $s_2 s_4 s_1 s_1 s_3 s_1 s_4$ | $\begin{pmatrix} 0 & 0 & 1 & 0 & 0 & 0 & 0 \\ 1 & 1 & 0 & 1 & 0 & 0 & 0 \\ 0 & 0 & 1 & 1 & 0 & 0 & 0 \\ 0 & 0 & 0 & 0 & 1 & 1 & 1 \\ 0 & 0 & 0 & 1 & 0 & 1 & 0 \\ 1 & 0 & 0 & 0 & 0 & 0 & 1 \\ 1 & 1 & 1 & 0 & 1 & 1 & 0 \end{pmatrix}$ | -1 |
| 42. | $x^4 y^{-5}$ | $s_1 s_3 s_3 s_1 s_1 s_3 s_1$ | $\begin{pmatrix} 1 & 0 & 0 & 1 & 0 & 1 & 1 \\ 1 & 0 & 1 & 1 & 1 & 0 & 0 \\ 0 & 1 & 0 & 0 & 0 & 0 & 0 \\ 0 & 0 & 1 & 1 & 0 & 0 & 0 \\ 0 & 1 & 0 & 0 & 1 & 0 & 1 \\ 0 & 0 & 0 & 0 & 1 & 0 & 0 \\ 1 & 0 & 0 & 0 & 0 & 1 & 1 \end{pmatrix}$ | -1 |
| 43. | $x^4 y^{13}$ | $s_2 s_2 s_4 s_2 s_4 s_4 s_1$ | $\begin{pmatrix} 1 & 1 & 1 & 0 & 0 & 0 & 1 \\ 0 & 0 & 0 & 1 & 1 & 0 & 0 \\ 0 & 1 & 0 & 1 & 1 & 0 & 0 \\ 1 & 0 & 0 & 0 & 0 & 1 & 0 \\ 1 & 0 & 0 & 0 & 0 & 1 & 1 \\ 0 & 1 & 1 & 0 & 0 & 0 & 0 \\ 0 & 0 & 0 & 1 & 0 & 0 & 1 \end{pmatrix}$ | -1 |
| 44. | $xy$         | $s_2 s_4 s_4 s_1 s_3 s_3 s_3$ | $\begin{pmatrix} 0 & 0 & 0 & 1 & 0 & 1 & 0 \\ 1 & 1 & 0 & 0 & 0 & 1 & 0 \\ 1 & 1 & 0 & 0 & 0 & 0 & 1 \\ 0 & 0 & 1 & 0 & 1 & 0 & 0 \\ 0 & 0 & 1 & 1 & 0 & 0 & 0 \\ 0 & 0 & 0 & 0 & 1 & 0 & 0 \\ 1 & 0 & 0 & 1 & 0 & 0 & 1 \end{pmatrix}$ | -1 |
| 45. | $xy^{-9}$    | $s_1 s_3 s_2 s_4 s_2 s_2 s_4$ | $\begin{pmatrix} 1 & 0 & 1 & 1 & 0 & 1 & 0 \\ 0 & 0 & 0 & 0 & 1 & 0 & 0 \\ 1 & 0 & 1 & 0 & 1 & 0 & 0 \\ 0 & 0 & 0 & 0 & 1 & 1 & 1 \\ 0 & 1 & 1 & 1 & 0 & 0 & 0 \\ 1 & 0 & 0 & 0 & 0 & 1 & 1 \\ 0 & 1 & 0 & 0 & 0 & 0 & 0 \end{pmatrix}$ | 1  |
| 46. | $x^2 y^3$    | $s_1 s_4 s_4 s_1 s_4 s_4 s_4$ | $\begin{pmatrix} 0 & 0 & 0 & 1 & 0 & 1 & 0 \\ 1 & 1 & 0 & 0 & 0 & 1 & 0 \\ 0 & 1 & 0 & 0 & 1 & 0 & 0 \\ 0 & 0 & 1 & 0 & 0 & 0 & 1 \\ 1 & 0 & 1 & 1 & 0 & 0 & 0 \\ 1 & 0 & 0 & 0 & 0 & 0 & 1 \\ 0 & 0 & 0 & 1 & 1 & 0 & 0 \end{pmatrix}$ | 1  |
| 47. | $x^2 y^{-3}$ | $s_2 s_4 s_1 s_4 s_2 s_4 s_1$ | $\begin{pmatrix} 1 & 0 & 0 & 0 & 0 & 0 & 1 \\ 1 & 1 & 1 & 0 & 1 & 0 & 0 \\ 0 & 0 & 1 & 1 & 0 & 0 & 0 \\ 1 & 1 & 0 & 0 & 1 & 1 & 0 \\ 0 & 0 & 1 & 0 & 1 & 1 & 1 \\ 0 & 0 & 0 & 1 & 0 & 0 & 0 \\ 0 & 0 & 0 & 0 & 0 & 0 & 1 \end{pmatrix}$ | -1 |

|     |             |                         |                                                                                                                                                                                                                                         |    |
|-----|-------------|-------------------------|-----------------------------------------------------------------------------------------------------------------------------------------------------------------------------------------------------------------------------------------|----|
| 48. | $x^3y^9$    | $s_1s_1s_4s_1s_3s_3s_2$ | $\begin{pmatrix} 0 & 1 & 0 & 0 & 1 & 0 & 0 \\ 0 & 0 & 0 & 0 & 0 & 1 & 0 \\ 0 & 0 & 1 & 0 & 1 & 0 & 1 \\ 1 & 1 & 1 & 1 & 0 & 0 & 1 \\ 1 & 0 & 0 & 0 & 0 & 0 & 0 \\ 0 & 1 & 0 & 1 & 0 & 0 & 0 \\ 1 & 0 & 0 & 1 & 0 & 1 & 1 \end{pmatrix}$ | -1 |
| 49. | $y^{14}$    | $s_3s_2s_4s_1s_4s_4s_1$ | $\begin{pmatrix} 0 & 0 & 0 & 0 & 0 & 0 & 1 \\ 0 & 0 & 0 & 1 & 1 & 0 & 0 \\ 0 & 0 & 0 & 0 & 1 & 0 & 0 \\ 0 & 1 & 0 & 0 & 0 & 1 & 0 \\ 1 & 0 & 0 & 1 & 0 & 1 & 1 \\ 1 & 1 & 1 & 1 & 0 & 0 & 0 \\ 0 & 1 & 1 & 0 & 0 & 0 & 1 \end{pmatrix}$ | -1 |
| 50. | $x^2y^2$    | $s_3s_2s_4s_2s_2s_3s_3$ | $\begin{pmatrix} 0 & 1 & 1 & 0 & 1 & 1 & 0 \\ 0 & 0 & 0 & 1 & 0 & 1 & 0 \\ 0 & 1 & 0 & 1 & 0 & 0 & 1 \\ 0 & 0 & 0 & 1 & 1 & 0 & 0 \\ 1 & 1 & 1 & 0 & 0 & 0 & 0 \\ 0 & 0 & 0 & 0 & 1 & 0 & 0 \\ 1 & 0 & 0 & 0 & 0 & 0 & 1 \end{pmatrix}$ | 1  |
| 51. | $x^2y^{-4}$ | $s_2s_3s_1s_3s_1s_3s_3$ | $\begin{pmatrix} 1 & 0 & 0 & 0 & 0 & 1 & 0 \\ 0 & 0 & 1 & 0 & 0 & 1 & 0 \\ 1 & 1 & 1 & 0 & 0 & 0 & 1 \\ 0 & 0 & 0 & 1 & 1 & 0 & 0 \\ 0 & 1 & 1 & 0 & 1 & 0 & 0 \\ 1 & 0 & 0 & 0 & 0 & 0 & 0 \\ 0 & 0 & 0 & 1 & 1 & 0 & 1 \end{pmatrix}$ | 1  |
| 52. | $x^4y^8$    | $s_1s_4s_1s_1s_3s_1s_1$ | $\begin{pmatrix} 0 & 0 & 0 & 0 & 0 & 0 & 1 \\ 1 & 1 & 1 & 0 & 1 & 1 & 0 \\ 1 & 0 & 1 & 1 & 0 & 0 & 0 \\ 0 & 1 & 0 & 1 & 0 & 0 & 0 \\ 0 & 0 & 1 & 0 & 0 & 0 & 1 \\ 0 & 0 & 0 & 1 & 0 & 1 & 0 \\ 1 & 0 & 0 & 0 & 1 & 1 & 1 \end{pmatrix}$ | -1 |
| 53. | $x^4y^{-2}$ | $s_1s_3s_1s_4s_4s_1s_4$ | $\begin{pmatrix} 1 & 0 & 0 & 0 & 1 & 0 & 0 \\ 1 & 0 & 1 & 0 & 0 & 0 & 0 \\ 0 & 1 & 1 & 1 & 0 & 0 & 0 \\ 0 & 0 & 0 & 0 & 0 & 1 & 1 \\ 0 & 1 & 1 & 0 & 1 & 1 & 0 \\ 0 & 0 & 0 & 1 & 0 & 0 & 1 \\ 1 & 0 & 0 & 0 & 0 & 1 & 0 \end{pmatrix}$ | -1 |
| 54. | $xy^{10}$   | $s_1s_1s_1s_3s_1s_1s_3$ | $\begin{pmatrix} 1 & 0 & 0 & 1 & 1 & 1 & 0 \\ 1 & 1 & 1 & 0 & 0 & 0 & 0 \\ 0 & 0 & 1 & 0 & 1 & 0 & 1 \\ 1 & 0 & 0 & 0 & 0 & 1 & 0 \\ 0 & 1 & 0 & 0 & 0 & 1 & 0 \\ 0 & 1 & 0 & 1 & 1 & 0 & 0 \\ 0 & 0 & 1 & 0 & 0 & 0 & 1 \end{pmatrix}$ | 1  |

|     |              |                               |                                                                                                                                                                                                                                         |    |
|-----|--------------|-------------------------------|-----------------------------------------------------------------------------------------------------------------------------------------------------------------------------------------------------------------------------------------|----|
| 55. | $xy^4$       | $s_1 s_1 s_3 s_1 s_3 s_3 s_3$ | $\begin{pmatrix} 1 & 0 & 1 & 1 & 0 & 1 & 0 \\ 1 & 1 & 0 & 0 & 0 & 1 & 0 \\ 0 & 0 & 0 & 0 & 0 & 0 & 1 \\ 1 & 0 & 0 & 0 & 1 & 0 & 0 \\ 0 & 1 & 0 & 1 & 0 & 0 & 0 \\ 0 & 1 & 0 & 0 & 1 & 0 & 0 \\ 0 & 0 & 1 & 1 & 0 & 0 & 1 \end{pmatrix}$ | 1  |
| 56. | $x^5 y^{-8}$ | $s_1 s_4 s_4 s_2 s_3 s_3 s_1$ | $\begin{pmatrix} 0 & 0 & 0 & 0 & 0 & 1 & 1 \\ 1 & 0 & 0 & 1 & 1 & 0 & 0 \\ 1 & 0 & 1 & 0 & 1 & 0 & 0 \\ 1 & 1 & 0 & 1 & 0 & 0 & 0 \\ 0 & 0 & 0 & 1 & 0 & 0 & 1 \\ 0 & 0 & 1 & 0 & 0 & 0 & 0 \\ 0 & 1 & 0 & 0 & 0 & 1 & 1 \end{pmatrix}$ | 1  |
| 57. | $x^2 y^6$    | $s_1 s_1 s_1 s_4 s_1 s_1 s_4$ | $\begin{pmatrix} 0 & 0 & 1 & 0 & 0 & 0 & 0 \\ 1 & 1 & 1 & 1 & 1 & 0 & 0 \\ 0 & 1 & 0 & 0 & 1 & 0 & 0 \\ 0 & 0 & 1 & 0 & 1 & 1 & 1 \\ 1 & 0 & 0 & 1 & 0 & 1 & 0 \\ 1 & 0 & 0 & 0 & 0 & 0 & 1 \\ 0 & 1 & 0 & 0 & 0 & 1 & 0 \end{pmatrix}$ | -1 |
| 58. | $x^3 y^{-6}$ | $s_2 s_2 s_3 s_1 s_1 s_1 s_3$ | $\begin{pmatrix} 0 & 1 & 1 & 1 & 1 & 1 & 0 \\ 1 & 0 & 1 & 1 & 0 & 0 & 0 \\ 1 & 0 & 0 & 0 & 1 & 0 & 1 \\ 1 & 1 & 0 & 0 & 0 & 1 & 0 \\ 0 & 0 & 0 & 0 & 0 & 1 & 0 \\ 0 & 1 & 0 & 0 & 1 & 0 & 0 \\ 0 & 0 & 0 & 1 & 0 & 0 & 1 \end{pmatrix}$ | -1 |
| 59. | $x^3 y^{12}$ | $s_2 s_4 s_4 s_1 s_4 s_4 s_1$ | $\begin{pmatrix} 0 & 0 & 0 & 0 & 0 & 0 & 1 \\ 1 & 0 & 0 & 1 & 1 & 0 & 0 \\ 1 & 1 & 0 & 0 & 1 & 0 & 0 \\ 1 & 1 & 0 & 0 & 0 & 1 & 0 \\ 0 & 0 & 0 & 1 & 0 & 1 & 1 \\ 0 & 0 & 1 & 1 & 0 & 0 & 0 \\ 0 & 0 & 1 & 0 & 0 & 0 & 1 \end{pmatrix}$ | 1  |
| 60. | $x^4$        | $s_1 s_1 s_4 s_4 s_1 s_3 s_3$ | $\begin{pmatrix} 1 & 0 & 0 & 1 & 0 & 1 & 0 \\ 0 & 1 & 0 & 0 & 0 & 1 & 0 \\ 1 & 1 & 1 & 0 & 0 & 0 & 1 \\ 0 & 0 & 0 & 0 & 1 & 0 & 0 \\ 0 & 1 & 0 & 1 & 1 & 0 & 0 \\ 0 & 0 & 1 & 0 & 0 & 0 & 0 \\ 1 & 0 & 0 & 0 & 1 & 0 & 1 \end{pmatrix}$ | -1 |
| 61. | $y^{-1}$     | $s_1 s_3 s_1 s_4 s_2 s_2 s_4$ | $\begin{pmatrix} 0 & 0 & 0 & 1 & 0 & 1 & 0 \\ 1 & 0 & 1 & 0 & 1 & 0 & 0 \\ 0 & 0 & 0 & 0 & 1 & 0 & 0 \\ 0 & 1 & 1 & 0 & 1 & 1 & 1 \\ 0 & 1 & 1 & 1 & 0 & 0 & 0 \\ 1 & 0 & 0 & 0 & 0 & 1 & 1 \\ 1 & 0 & 0 & 0 & 0 & 0 & 0 \end{pmatrix}$ | -1 |

|     |             |                         |                                                                                                                                                                                                                                         |    |
|-----|-------------|-------------------------|-----------------------------------------------------------------------------------------------------------------------------------------------------------------------------------------------------------------------------------------|----|
| 62. | $x^2y^{11}$ | $s_2s_3s_3s_1s_1s_3s_1$ | $\begin{pmatrix} 1 & 0 & 0 & 1 & 0 & 1 & 1 \\ 0 & 0 & 1 & 1 & 1 & 0 & 0 \\ 1 & 1 & 0 & 0 & 0 & 0 & 0 \\ 0 & 0 & 1 & 1 & 0 & 0 & 0 \\ 0 & 1 & 0 & 0 & 1 & 0 & 1 \\ 1 & 0 & 0 & 0 & 1 & 0 & 0 \\ 0 & 0 & 0 & 0 & 0 & 1 & 1 \end{pmatrix}$ | 1  |
| 63. | $x^2y^5$    | $s_1s_1s_4s_2s_4s_4s_1$ | $\begin{pmatrix} 1 & 1 & 1 & 0 & 0 & 0 & 1 \\ 0 & 1 & 0 & 1 & 1 & 0 & 0 \\ 0 & 0 & 0 & 1 & 1 & 0 & 0 \\ 1 & 0 & 0 & 0 & 0 & 1 & 0 \\ 1 & 0 & 0 & 0 & 0 & 1 & 1 \\ 0 & 0 & 1 & 0 & 0 & 0 & 0 \\ 0 & 1 & 0 & 1 & 0 & 0 & 1 \end{pmatrix}$ | 1  |
| 64. | $x^4y^{-7}$ | $s_3s_3s_3s_2s_4s_2s_4$ | $\begin{pmatrix} 1 & 0 & 0 & 0 & 0 & 1 & 0 \\ 0 & 0 & 1 & 1 & 1 & 0 & 0 \\ 0 & 0 & 1 & 0 & 0 & 0 & 0 \\ 0 & 1 & 0 & 0 & 0 & 1 & 1 \\ 0 & 1 & 0 & 1 & 1 & 0 & 0 \\ 0 & 0 & 0 & 1 & 0 & 1 & 1 \\ 1 & 0 & 0 & 0 & 0 & 0 & 0 \end{pmatrix}$ | 1  |
| 65. | $x^4y^7$    | $s_1s_1s_3s_2s_4s_1s_4$ | $\begin{pmatrix} 1 & 1 & 0 & 1 & 1 & 0 & 0 \\ 1 & 0 & 0 & 0 & 0 & 0 & 0 \\ 0 & 1 & 0 & 1 & 0 & 0 & 0 \\ 0 & 0 & 0 & 0 & 0 & 1 & 1 \\ 0 & 0 & 1 & 1 & 1 & 1 & 0 \\ 0 & 1 & 0 & 0 & 0 & 0 & 1 \\ 1 & 0 & 1 & 0 & 0 & 1 & 0 \end{pmatrix}$ | 1  |
| 66. | $xy^{-5}$   | $s_1s_3s_1s_3s_3s_1s_1$ | $\begin{pmatrix} 1 & 0 & 0 & 1 & 0 & 0 & 1 \\ 1 & 0 & 0 & 0 & 1 & 1 & 0 \\ 0 & 0 & 0 & 1 & 0 & 0 & 0 \\ 1 & 0 & 1 & 0 & 0 & 0 & 0 \\ 0 & 0 & 0 & 0 & 0 & 0 & 1 \\ 0 & 1 & 1 & 0 & 0 & 1 & 0 \\ 0 & 1 & 1 & 0 & 1 & 1 & 1 \end{pmatrix}$ | -1 |
| 67. | $xy^{13}$   | $s_1s_4s_4s_2s_2s_4s_2$ | $\begin{pmatrix} 1 & 0 & 0 & 1 & 0 & 0 & 0 \\ 1 & 1 & 0 & 1 & 0 & 0 & 0 \\ 0 & 0 & 1 & 0 & 1 & 0 & 1 \\ 1 & 0 & 1 & 0 & 0 & 0 & 1 \\ 0 & 1 & 0 & 0 & 1 & 1 & 0 \\ 0 & 0 & 0 & 1 & 1 & 1 & 0 \\ 0 & 0 & 0 & 0 & 0 & 0 & 1 \end{pmatrix}$ | -1 |
| 68. | $x^5y$      | $s_1s_3s_1s_4s_2s_2s_3$ | $\begin{pmatrix} 0 & 1 & 1 & 0 & 1 & 1 & 0 \\ 1 & 0 & 0 & 0 & 0 & 1 & 0 \\ 1 & 0 & 1 & 0 & 1 & 0 & 1 \\ 1 & 0 & 0 & 0 & 0 & 0 & 0 \\ 0 & 1 & 1 & 1 & 0 & 0 & 0 \\ 0 & 0 & 0 & 0 & 1 & 0 & 0 \\ 0 & 0 & 0 & 1 & 0 & 1 & 1 \end{pmatrix}$ | 1  |

|     |             |                         |                                                                                                                                                                                                                                         |    |
|-----|-------------|-------------------------|-----------------------------------------------------------------------------------------------------------------------------------------------------------------------------------------------------------------------------------------|----|
| 69. | $x^2y^{-9}$ | $s_1s_4s_1s_1s_4s_1s_3$ | $\begin{pmatrix} 0 & 0 & 0 & 1 & 0 & 1 & 0 \\ 1 & 1 & 1 & 0 & 0 & 0 & 0 \\ 0 & 1 & 0 & 1 & 0 & 0 & 1 \\ 0 & 0 & 1 & 0 & 0 & 1 & 0 \\ 1 & 0 & 1 & 1 & 1 & 1 & 0 \\ 1 & 0 & 0 & 0 & 0 & 0 & 0 \\ 0 & 0 & 0 & 0 & 1 & 0 & 1 \end{pmatrix}$ | 1  |
| 70. | $x^3y^3$    | $s_1s_1s_3s_2s_3s_2s_3$ | $\begin{pmatrix} 0 & 1 & 0 & 1 & 1 & 1 & 0 \\ 0 & 0 & 1 & 1 & 0 & 1 & 0 \\ 0 & 0 & 0 & 0 & 0 & 0 & 1 \\ 1 & 1 & 0 & 1 & 0 & 0 & 0 \\ 1 & 0 & 1 & 0 & 0 & 0 & 0 \\ 0 & 1 & 0 & 0 & 1 & 0 & 0 \\ 1 & 0 & 0 & 0 & 0 & 1 & 1 \end{pmatrix}$ | 1  |
| 71. | $x^3y^{-3}$ | $s_3s_2s_4s_1s_4s_4s_4$ | $\begin{pmatrix} 1 & 0 & 0 & 1 & 0 & 1 & 0 \\ 0 & 1 & 0 & 0 & 0 & 1 & 0 \\ 0 & 0 & 0 & 0 & 1 & 0 & 0 \\ 0 & 1 & 1 & 0 & 0 & 0 & 1 \\ 1 & 1 & 1 & 1 & 0 & 0 & 0 \\ 0 & 0 & 0 & 0 & 0 & 0 & 1 \\ 0 & 0 & 0 & 1 & 1 & 0 & 0 \end{pmatrix}$ | -1 |
| 72. | $x^4y^9$    | $s_3s_3s_1s_3s_1s_4s_4$ | $\begin{pmatrix} 0 & 0 & 0 & 1 & 1 & 1 & 0 \\ 1 & 0 & 0 & 0 & 0 & 1 & 0 \\ 0 & 0 & 1 & 0 & 0 & 0 & 0 \\ 0 & 0 & 0 & 1 & 1 & 0 & 1 \\ 0 & 1 & 1 & 0 & 1 & 0 & 0 \\ 0 & 1 & 1 & 0 & 0 & 0 & 1 \\ 1 & 0 & 0 & 0 & 0 & 0 & 0 \end{pmatrix}$ | -1 |
| 73. | $x^2y^{14}$ | $s_1s_1s_1s_4s_2s_4s_2$ | $\begin{pmatrix} 1 & 1 & 1 & 1 & 0 & 0 & 0 \\ 0 & 1 & 0 & 0 & 0 & 0 & 0 \\ 0 & 0 & 1 & 0 & 1 & 0 & 1 \\ 1 & 0 & 0 & 1 & 0 & 0 & 1 \\ 1 & 0 & 0 & 0 & 1 & 1 & 0 \\ 0 & 0 & 1 & 0 & 1 & 1 & 0 \\ 0 & 1 & 0 & 0 & 0 & 0 & 1 \end{pmatrix}$ | 1  |
| 74. | $x^4y^2$    | $s_1s_3s_3s_1s_3s_1s_4$ | $\begin{pmatrix} 0 & 1 & 0 & 0 & 0 & 0 & 0 \\ 1 & 0 & 0 & 1 & 0 & 0 & 0 \\ 1 & 0 & 1 & 1 & 0 & 0 & 0 \\ 0 & 0 & 0 & 0 & 1 & 1 & 1 \\ 0 & 0 & 1 & 1 & 0 & 1 & 0 \\ 0 & 1 & 0 & 0 & 0 & 0 & 1 \\ 1 & 0 & 0 & 0 & 1 & 1 & 0 \end{pmatrix}$ | -1 |
| 75. | $x^4y^{-4}$ | $s_1s_4s_1s_4s_4s_1s_4$ | $\begin{pmatrix} 0 & 0 & 0 & 0 & 1 & 0 & 0 \\ 1 & 1 & 1 & 0 & 0 & 0 & 0 \\ 1 & 0 & 1 & 1 & 0 & 0 & 0 \\ 0 & 1 & 0 & 0 & 0 & 1 & 1 \\ 0 & 0 & 1 & 0 & 1 & 1 & 0 \\ 0 & 0 & 0 & 1 & 0 & 0 & 1 \\ 1 & 0 & 0 & 0 & 0 & 1 & 0 \end{pmatrix}$ | -1 |

|     |             |                         |                                                                                                                                                                                                                                         |    |
|-----|-------------|-------------------------|-----------------------------------------------------------------------------------------------------------------------------------------------------------------------------------------------------------------------------------------|----|
| 76. | $x^6y^8$    | $s_1s_1s_4s_1s_3s_1s_1$ | $\begin{pmatrix} 1 & 0 & 0 & 0 & 0 & 0 & 1 \\ 0 & 1 & 0 & 0 & 1 & 1 & 0 \\ 0 & 1 & 0 & 1 & 0 & 0 & 0 \\ 1 & 1 & 1 & 1 & 0 & 0 & 0 \\ 0 & 0 & 0 & 0 & 0 & 0 & 1 \\ 1 & 0 & 0 & 1 & 0 & 1 & 0 \\ 0 & 0 & 1 & 0 & 1 & 1 & 1 \end{pmatrix}$ | 1  |
| 77. | $xy^{-2}$   | $s_1s_1s_3s_1s_4s_4s_4$ | $\begin{pmatrix} 1 & 0 & 1 & 1 & 0 & 1 & 0 \\ 1 & 1 & 0 & 0 & 0 & 1 & 0 \\ 0 & 0 & 0 & 0 & 1 & 0 & 0 \\ 1 & 0 & 0 & 0 & 0 & 0 & 1 \\ 0 & 1 & 0 & 1 & 0 & 0 & 0 \\ 0 & 1 & 0 & 0 & 0 & 0 & 1 \\ 0 & 0 & 1 & 1 & 1 & 0 & 0 \end{pmatrix}$ | -1 |
| 78. | $x^5y^{10}$ | $s_1s_1s_3s_1s_1s_1s_3$ | $\begin{pmatrix} 0 & 0 & 1 & 1 & 1 & 1 & 0 \\ 1 & 0 & 1 & 1 & 0 & 0 & 0 \\ 1 & 0 & 0 & 0 & 1 & 0 & 1 \\ 1 & 1 & 0 & 0 & 0 & 1 & 0 \\ 0 & 1 & 0 & 0 & 0 & 1 & 0 \\ 0 & 0 & 0 & 0 & 1 & 0 & 0 \\ 0 & 1 & 0 & 1 & 0 & 0 & 1 \end{pmatrix}$ | 1  |
| 79. | $x^5y^4$    | $s_1s_3s_1s_3s_3s_1s_3$ | $\begin{pmatrix} 0 & 1 & 1 & 0 & 1 & 1 & 0 \\ 1 & 0 & 0 & 1 & 0 & 0 & 0 \\ 1 & 0 & 1 & 0 & 0 & 0 & 1 \\ 1 & 0 & 0 & 0 & 1 & 1 & 0 \\ 0 & 1 & 1 & 0 & 0 & 1 & 0 \\ 0 & 0 & 0 & 1 & 0 & 0 & 0 \\ 0 & 0 & 0 & 0 & 0 & 0 & 1 \end{pmatrix}$ | -1 |
| 80. | $x^2y^{-8}$ | $s_1s_1s_1s_3s_2s_2s_4$ | $\begin{pmatrix} 0 & 1 & 0 & 0 & 0 & 1 & 0 \\ 0 & 0 & 1 & 0 & 1 & 0 & 0 \\ 1 & 1 & 1 & 0 & 1 & 0 & 0 \\ 1 & 0 & 0 & 1 & 1 & 1 & 1 \\ 0 & 0 & 1 & 0 & 0 & 0 & 0 \\ 1 & 0 & 0 & 0 & 0 & 1 & 1 \\ 0 & 1 & 0 & 1 & 0 & 0 & 0 \end{pmatrix}$ | -1 |
| 81. | $x^3y^6$    | $s_1s_1s_4s_2s_2s_4s_2$ | $\begin{pmatrix} 0 & 1 & 0 & 1 & 0 & 0 & 0 \\ 0 & 0 & 0 & 1 & 0 & 0 & 0 \\ 0 & 0 & 1 & 0 & 1 & 0 & 1 \\ 1 & 1 & 1 & 0 & 0 & 0 & 1 \\ 1 & 0 & 0 & 0 & 1 & 1 & 0 \\ 0 & 1 & 0 & 1 & 1 & 1 & 0 \\ 1 & 0 & 0 & 0 & 0 & 0 & 1 \end{pmatrix}$ | 1  |
| 82. | $x^4y^{-6}$ | $s_1s_3s_1s_1s_3s_2s_2$ | $\begin{pmatrix} 1 & 0 & 1 & 0 & 1 & 0 & 0 \\ 0 & 1 & 1 & 1 & 0 & 1 & 0 \\ 1 & 0 & 0 & 0 & 0 & 0 & 1 \\ 0 & 1 & 1 & 0 & 0 & 0 & 1 \\ 0 & 0 & 0 & 1 & 0 & 0 & 0 \\ 0 & 0 & 0 & 1 & 0 & 1 & 0 \\ 1 & 0 & 0 & 0 & 1 & 1 & 1 \end{pmatrix}$ | -1 |



|     |             |                         |                                                                                                                                                                                                                                         |    |
|-----|-------------|-------------------------|-----------------------------------------------------------------------------------------------------------------------------------------------------------------------------------------------------------------------------------------|----|
| 83. | $x^4y^{12}$ | $s_1s_4s_4s_1s_4s_2s_4$ | $\begin{pmatrix} 1 & 0 & 1 & 1 & 0 & 1 & 0 \\ 0 & 0 & 0 & 1 & 1 & 0 & 0 \\ 1 & 1 & 0 & 0 & 0 & 0 & 0 \\ 0 & 0 & 0 & 1 & 0 & 1 & 1 \\ 0 & 1 & 0 & 0 & 1 & 0 & 0 \\ 0 & 0 & 1 & 0 & 0 & 1 & 1 \\ 1 & 0 & 0 & 0 & 0 & 0 & 0 \end{pmatrix}$ | -1 |
| 84. | $x^5$       | $s_2s_2s_4s_1s_3s_2s_2$ | $\begin{pmatrix} 0 & 0 & 0 & 0 & 1 & 0 & 0 \\ 0 & 0 & 0 & 1 & 0 & 1 & 0 \\ 1 & 0 & 0 & 0 & 0 & 0 & 1 \\ 0 & 1 & 0 & 0 & 0 & 0 & 1 \\ 1 & 0 & 0 & 1 & 0 & 0 & 0 \\ 1 & 1 & 1 & 1 & 0 & 1 & 0 \\ 0 & 1 & 1 & 0 & 1 & 1 & 1 \end{pmatrix}$ | -1 |
| 85. | $x^2y^{-1}$ | $s_1s_1s_4s_4s_2s_3s_2$ | $\begin{pmatrix} 1 & 1 & 1 & 0 & 1 & 0 & 0 \\ 0 & 1 & 0 & 1 & 0 & 1 & 0 \\ 0 & 0 & 0 & 0 & 1 & 0 & 1 \\ 1 & 0 & 0 & 1 & 0 & 0 & 1 \\ 1 & 0 & 0 & 0 & 0 & 0 & 0 \\ 0 & 0 & 1 & 0 & 0 & 0 & 0 \\ 0 & 1 & 0 & 0 & 1 & 1 & 1 \end{pmatrix}$ | 1  |
| 86. | $x^4y^{11}$ | $s_1s_3s_3s_1s_1s_3s_2$ | $\begin{pmatrix} 0 & 1 & 0 & 0 & 0 & 0 & 0 \\ 1 & 0 & 0 & 1 & 0 & 1 & 0 \\ 1 & 0 & 1 & 1 & 1 & 0 & 1 \\ 0 & 0 & 0 & 0 & 1 & 0 & 1 \\ 0 & 0 & 1 & 1 & 0 & 0 & 0 \\ 0 & 1 & 0 & 0 & 1 & 0 & 0 \\ 1 & 0 & 0 & 0 & 0 & 1 & 1 \end{pmatrix}$ | 1  |
| 87. | $x^4y^5$    | $s_1s_4s_1s_4s_2s_4s_1$ | $\begin{pmatrix} 0 & 0 & 0 & 0 & 0 & 0 & 1 \\ 1 & 1 & 1 & 0 & 1 & 0 & 0 \\ 1 & 0 & 1 & 1 & 0 & 0 & 0 \\ 0 & 1 & 0 & 0 & 1 & 1 & 0 \\ 0 & 0 & 1 & 0 & 1 & 1 & 1 \\ 0 & 0 & 0 & 1 & 0 & 0 & 0 \\ 1 & 0 & 0 & 0 & 0 & 0 & 1 \end{pmatrix}$ | 1  |
| 88. | $x^6y^{-7}$ | $s_1s_1s_3s_1s_4s_1s_3$ | $\begin{pmatrix} 1 & 0 & 1 & 1 & 0 & 1 & 0 \\ 0 & 1 & 0 & 0 & 0 & 0 & 0 \\ 0 & 1 & 0 & 1 & 0 & 0 & 1 \\ 1 & 1 & 0 & 0 & 0 & 1 & 0 \\ 0 & 0 & 1 & 1 & 1 & 1 & 0 \\ 1 & 0 & 0 & 0 & 0 & 0 & 0 \\ 0 & 0 & 0 & 0 & 1 & 0 & 1 \end{pmatrix}$ | -1 |
| 89. | $xy^7$      | $s_1s_1s_1s_3s_2s_4s_4$ | $\begin{pmatrix} 1 & 0 & 0 & 1 & 1 & 1 & 0 \\ 1 & 1 & 1 & 0 & 1 & 1 & 0 \\ 0 & 0 & 1 & 0 & 0 & 0 & 0 \\ 1 & 0 & 0 & 0 & 0 & 0 & 1 \\ 0 & 1 & 0 & 0 & 0 & 0 & 0 \\ 0 & 1 & 0 & 1 & 0 & 0 & 1 \\ 0 & 0 & 1 & 0 & 1 & 0 & 0 \end{pmatrix}$ | 1  |

|     |             |                         |                                                                                                                                                                                                                                         |    |
|-----|-------------|-------------------------|-----------------------------------------------------------------------------------------------------------------------------------------------------------------------------------------------------------------------------------------|----|
| 90. | $x^5y^{-5}$ | $s_1s_3s_1s_1s_3s_3s_1$ | $\begin{pmatrix} 0 & 1 & 1 & 0 & 0 & 1 & 1 \\ 1 & 0 & 0 & 0 & 1 & 0 & 0 \\ 1 & 0 & 1 & 0 & 1 & 0 & 0 \\ 1 & 0 & 0 & 0 & 0 & 0 & 0 \\ 0 & 1 & 1 & 1 & 0 & 0 & 1 \\ 0 & 0 & 0 & 1 & 0 & 0 & 0 \\ 0 & 0 & 0 & 1 & 0 & 1 & 1 \end{pmatrix}$ | -1 |
| 91. | $x^5y^{13}$ | $s_1s_4s_2s_2s_4s_4s_2$ | $\begin{pmatrix} 0 & 0 & 0 & 1 & 1 & 0 & 0 \\ 1 & 0 & 1 & 0 & 0 & 0 & 0 \\ 1 & 0 & 1 & 1 & 1 & 0 & 1 \\ 1 & 1 & 0 & 0 & 0 & 0 & 1 \\ 0 & 0 & 1 & 0 & 0 & 1 & 0 \\ 0 & 0 & 0 & 0 & 0 & 1 & 0 \\ 0 & 1 & 0 & 1 & 0 & 0 & 1 \end{pmatrix}$ | -1 |
| 92. | $x^2y$      | $s_1s_4s_4s_2s_3s_3s_3$ | $\begin{pmatrix} 0 & 1 & 0 & 0 & 0 & 1 & 0 \\ 0 & 0 & 0 & 0 & 0 & 1 & 0 \\ 1 & 1 & 0 & 1 & 0 & 0 & 1 \\ 1 & 0 & 0 & 1 & 1 & 0 & 0 \\ 0 & 0 & 1 & 0 & 0 & 0 & 0 \\ 1 & 0 & 1 & 0 & 1 & 0 & 0 \\ 0 & 0 & 0 & 1 & 0 & 0 & 1 \end{pmatrix}$ | 1  |
| 93. | $x^3y^{-9}$ | $s_3s_3s_2s_4s_2s_4s_4$ | $\begin{pmatrix} 1 & 0 & 0 & 0 & 1 & 1 & 0 \\ 0 & 0 & 1 & 0 & 1 & 1 & 0 \\ 0 & 1 & 1 & 1 & 0 & 0 & 0 \\ 0 & 0 & 0 & 0 & 0 & 0 & 1 \\ 1 & 0 & 1 & 1 & 0 & 0 & 0 \\ 0 & 1 & 0 & 0 & 0 & 0 & 1 \\ 0 & 0 & 0 & 0 & 1 & 0 & 0 \end{pmatrix}$ | 1  |
| 94. | $x^4y^3$    | $s_3s_3s_3s_2s_3s_1s_4$ | $\begin{pmatrix} 0 & 0 & 1 & 0 & 0 & 0 & 0 \\ 1 & 0 & 0 & 0 & 0 & 0 & 0 \\ 0 & 0 & 1 & 1 & 0 & 0 & 0 \\ 0 & 0 & 0 & 1 & 1 & 1 & 1 \\ 0 & 1 & 0 & 0 & 0 & 1 & 0 \\ 0 & 1 & 0 & 1 & 0 & 0 & 1 \\ 1 & 0 & 0 & 0 & 1 & 1 & 0 \end{pmatrix}$ | 1  |
| 95. | $x^4y^{-3}$ | $s_1s_1s_4s_4s_2s_2s_4$ | $\begin{pmatrix} 1 & 0 & 0 & 1 & 0 & 1 & 0 \\ 0 & 1 & 0 & 0 & 1 & 0 & 0 \\ 1 & 1 & 1 & 0 & 1 & 0 & 0 \\ 0 & 0 & 0 & 0 & 1 & 1 & 1 \\ 0 & 1 & 0 & 1 & 0 & 0 & 0 \\ 0 & 0 & 1 & 0 & 0 & 1 & 1 \\ 1 & 0 & 0 & 0 & 0 & 0 & 0 \end{pmatrix}$ | -1 |
| 96. | $x^5y^9$    | $s_1s_1s_3s_1s_4s_2s_3$ | $\begin{pmatrix} 1 & 0 & 1 & 1 & 0 & 1 & 0 \\ 1 & 0 & 0 & 0 & 0 & 1 & 0 \\ 0 & 0 & 1 & 1 & 1 & 0 & 1 \\ 0 & 1 & 0 & 0 & 0 & 0 & 0 \\ 0 & 0 & 0 & 0 & 1 & 0 & 0 \\ 1 & 1 & 0 & 0 & 0 & 0 & 0 \\ 0 & 1 & 0 & 1 & 0 & 1 & 1 \end{pmatrix}$ | -1 |

|      |             |                         |                                                                                                                                                                                                                                         |    |
|------|-------------|-------------------------|-----------------------------------------------------------------------------------------------------------------------------------------------------------------------------------------------------------------------------------------|----|
| 97.  | $x^4y^{14}$ | $s_1s_1s_1s_4s_4s_2s_2$ | $\begin{pmatrix} 0 & 1 & 0 & 0 & 0 & 0 & 0 \\ 1 & 1 & 1 & 1 & 0 & 1 & 0 \\ 1 & 0 & 0 & 1 & 0 & 0 & 1 \\ 0 & 1 & 0 & 0 & 1 & 0 & 1 \\ 0 & 0 & 1 & 0 & 1 & 0 & 0 \\ 0 & 0 & 1 & 0 & 0 & 1 & 0 \\ 1 & 0 & 0 & 0 & 0 & 1 & 1 \end{pmatrix}$ | -1 |
| 98.  | $x^6y^2$    | $s_3s_1s_3s_1s_3s_1s_4$ | $\begin{pmatrix} 1 & 1 & 0 & 0 & 0 & 0 & 0 \\ 1 & 1 & 0 & 1 & 0 & 0 & 0 \\ 0 & 0 & 1 & 1 & 0 & 0 & 0 \\ 0 & 0 & 0 & 0 & 1 & 1 & 1 \\ 0 & 0 & 1 & 1 & 0 & 1 & 0 \\ 0 & 0 & 0 & 0 & 0 & 0 & 1 \\ 0 & 1 & 0 & 0 & 1 & 1 & 0 \end{pmatrix}$ | 1  |
| 99.  | $x^6y^{-4}$ | $s_1s_3s_3s_2s_3s_1s_3$ | $\begin{pmatrix} 1 & 0 & 0 & 1 & 1 & 1 & 0 \\ 0 & 1 & 0 & 1 & 0 & 0 & 0 \\ 0 & 0 & 0 & 0 & 0 & 0 & 1 \\ 1 & 0 & 0 & 0 & 1 & 1 & 0 \\ 0 & 1 & 0 & 0 & 0 & 1 & 0 \\ 1 & 0 & 1 & 1 & 0 & 0 & 0 \\ 0 & 0 & 1 & 0 & 0 & 0 & 1 \end{pmatrix}$ | 1  |
| 100. | $xy^8$      | $s_1s_1s_1s_4s_1s_1s_3$ | $\begin{pmatrix} 0 & 0 & 1 & 0 & 1 & 1 & 0 \\ 1 & 0 & 0 & 0 & 0 & 0 & 0 \\ 1 & 1 & 1 & 1 & 1 & 0 & 1 \\ 0 & 1 & 0 & 0 & 0 & 1 & 0 \\ 1 & 0 & 0 & 1 & 0 & 1 & 0 \\ 0 & 1 & 0 & 0 & 1 & 0 & 0 \\ 0 & 0 & 1 & 0 & 0 & 0 & 1 \end{pmatrix}$ | 1  |
| 101. | $x^5y^{-2}$ | $s_1s_3s_1s_4s_1s_4s_4$ | $\begin{pmatrix} 0 & 1 & 1 & 0 & 1 & 1 & 0 \\ 1 & 0 & 0 & 0 & 0 & 1 & 0 \\ 1 & 0 & 1 & 0 & 0 & 0 & 0 \\ 1 & 0 & 0 & 0 & 1 & 0 & 1 \\ 0 & 1 & 1 & 1 & 1 & 0 & 0 \\ 0 & 0 & 0 & 0 & 0 & 0 & 1 \\ 0 & 0 & 0 & 1 & 0 & 0 & 0 \end{pmatrix}$ | -1 |
| 102. | $x^2y^{10}$ | $s_1s_3s_3s_2s_3s_2s_4$ | $\begin{pmatrix} 0 & 0 & 0 & 0 & 0 & 1 & 0 \\ 0 & 1 & 0 & 0 & 0 & 0 & 0 \\ 1 & 0 & 0 & 0 & 1 & 0 & 0 \\ 1 & 0 & 0 & 1 & 1 & 1 & 1 \\ 0 & 0 & 1 & 0 & 0 & 0 & 0 \\ 1 & 0 & 1 & 1 & 0 & 1 & 1 \\ 0 & 1 & 0 & 1 & 0 & 0 & 0 \end{pmatrix}$ | -1 |
| 103. | $x^2y^4$    | $s_1s_3s_1s_1s_3s_3s_3$ | $\begin{pmatrix} 0 & 0 & 0 & 1 & 0 & 1 & 0 \\ 0 & 1 & 1 & 0 & 0 & 1 & 0 \\ 1 & 0 & 0 & 0 & 0 & 0 & 1 \\ 1 & 0 & 0 & 0 & 1 & 0 & 0 \\ 0 & 0 & 0 & 1 & 0 & 0 & 0 \\ 1 & 0 & 1 & 0 & 1 & 0 & 0 \\ 0 & 1 & 1 & 1 & 0 & 0 & 1 \end{pmatrix}$ | -1 |

|      |             |                         |                                                                                                                                                                                                                                         |    |
|------|-------------|-------------------------|-----------------------------------------------------------------------------------------------------------------------------------------------------------------------------------------------------------------------------------------|----|
| 104. | $x^6y^{-8}$ | $s_1s_1s_4s_4s_2s_3s_3$ | $\begin{pmatrix} 0 & 1 & 0 & 0 & 1 & 1 & 0 \\ 0 & 1 & 0 & 1 & 0 & 1 & 0 \\ 1 & 0 & 0 & 0 & 0 & 0 & 1 \\ 0 & 0 & 0 & 0 & 1 & 0 & 0 \\ 1 & 0 & 0 & 1 & 0 & 0 & 0 \\ 1 & 1 & 1 & 0 & 1 & 0 & 0 \\ 0 & 0 & 1 & 0 & 0 & 0 & 1 \end{pmatrix}$ | -1 |
| 105. | $x^4y^6$    | $s_1s_1s_4s_1s_1s_4s_1$ | $\begin{pmatrix} 1 & 0 & 0 & 1 & 0 & 0 & 1 \\ 0 & 1 & 0 & 0 & 0 & 0 & 0 \\ 1 & 1 & 1 & 1 & 0 & 0 & 0 \\ 0 & 0 & 0 & 0 & 0 & 1 & 0 \\ 0 & 1 & 0 & 1 & 1 & 1 & 1 \\ 0 & 0 & 1 & 0 & 1 & 0 & 0 \\ 1 & 0 & 0 & 0 & 1 & 0 & 1 \end{pmatrix}$ | -1 |
| 106. | $x^5y^{-6}$ | $s_1s_3s_3s_3s_1s_4s_2$ | $\begin{pmatrix} 1 & 0 & 0 & 0 & 0 & 0 & 0 \\ 1 & 0 & 1 & 0 & 0 & 0 & 0 \\ 0 & 1 & 0 & 0 & 0 & 0 & 1 \\ 0 & 1 & 0 & 0 & 1 & 0 & 1 \\ 0 & 0 & 1 & 0 & 0 & 1 & 0 \\ 1 & 0 & 0 & 1 & 1 & 1 & 0 \\ 0 & 0 & 0 & 1 & 1 & 0 & 1 \end{pmatrix}$ | -1 |
| 107. | $x^5y^{12}$ | $s_1s_4s_4s_4s_1s_4s_2$ | $\begin{pmatrix} 1 & 0 & 0 & 0 & 0 & 0 & 0 \\ 1 & 0 & 1 & 0 & 0 & 0 & 0 \\ 0 & 0 & 0 & 1 & 0 & 0 & 1 \\ 0 & 0 & 0 & 1 & 1 & 0 & 1 \\ 0 & 0 & 1 & 0 & 0 & 1 & 0 \\ 1 & 1 & 0 & 0 & 1 & 1 & 0 \\ 0 & 1 & 0 & 0 & 1 & 0 & 1 \end{pmatrix}$ | 1  |
| 108. | $x^6$       | $s_2s_4s_1s_3s_1s_1s_1$ | $\begin{pmatrix} 0 & 0 & 1 & 0 & 0 & 0 & 1 \\ 0 & 0 & 0 & 0 & 0 & 1 & 0 \\ 0 & 0 & 0 & 1 & 1 & 0 & 0 \\ 0 & 0 & 1 & 0 & 1 & 0 & 0 \\ 1 & 1 & 1 & 0 & 0 & 0 & 1 \\ 1 & 0 & 0 & 0 & 0 & 1 & 0 \\ 1 & 1 & 0 & 1 & 1 & 1 & 1 \end{pmatrix}$ | -1 |
| 109. | $x^4y^{-1}$ | $s_2s_4s_1s_3s_2s_4s_1$ | $\begin{pmatrix} 0 & 0 & 0 & 1 & 0 & 0 & 1 \\ 1 & 1 & 1 & 0 & 1 & 0 & 0 \\ 0 & 0 & 1 & 0 & 0 & 0 & 0 \\ 0 & 0 & 1 & 0 & 1 & 1 & 0 \\ 1 & 1 & 0 & 1 & 1 & 1 & 1 \\ 1 & 0 & 0 & 0 & 0 & 0 & 0 \\ 0 & 0 & 0 & 0 & 0 & 0 & 1 \end{pmatrix}$ | -1 |
| 110. | $x^6y^{11}$ | $s_1s_1s_3s_2s_3s_3s_1$ | $\begin{pmatrix} 1 & 0 & 1 & 0 & 0 & 1 & 1 \\ 0 & 1 & 0 & 1 & 1 & 0 & 0 \\ 0 & 1 & 0 & 0 & 1 & 0 & 0 \\ 1 & 1 & 0 & 1 & 0 & 0 & 0 \\ 0 & 0 & 1 & 1 & 0 & 0 & 1 \\ 1 & 0 & 0 & 0 & 0 & 0 & 0 \\ 0 & 0 & 0 & 0 & 0 & 1 & 1 \end{pmatrix}$ | -1 |

|      |             |                         |                                                                                                                                                                                                                                         |    |
|------|-------------|-------------------------|-----------------------------------------------------------------------------------------------------------------------------------------------------------------------------------------------------------------------------------------|----|
| 111. | $x^6y^5$    | $s_1s_4s_2s_4s_1s_4s_1$ | $\begin{pmatrix} 1 & 0 & 1 & 0 & 0 & 0 & 1 \\ 0 & 0 & 1 & 1 & 0 & 0 & 0 \\ 0 & 1 & 0 & 0 & 0 & 0 & 0 \\ 1 & 1 & 0 & 0 & 0 & 1 & 0 \\ 0 & 0 & 0 & 0 & 1 & 1 & 1 \\ 1 & 0 & 1 & 1 & 1 & 0 & 0 \\ 0 & 0 & 0 & 0 & 1 & 0 & 1 \end{pmatrix}$ | 1  |
| 112. | $xy^{-7}$   | $s_1s_1s_4s_1s_3s_1s_3$ | $\begin{pmatrix} 0 & 0 & 1 & 0 & 1 & 1 & 0 \\ 1 & 0 & 0 & 0 & 0 & 0 & 0 \\ 1 & 1 & 1 & 1 & 0 & 0 & 1 \\ 0 & 1 & 0 & 0 & 1 & 1 & 0 \\ 1 & 0 & 0 & 1 & 0 & 1 & 0 \\ 0 & 1 & 0 & 1 & 0 & 0 & 0 \\ 0 & 0 & 0 & 0 & 0 & 0 & 1 \end{pmatrix}$ | 1  |
| 113. | $x^5y^7$    | $s_2s_2s_4s_2s_4s_2s_3$ | $\begin{pmatrix} 1 & 0 & 0 & 0 & 0 & 1 & 0 \\ 0 & 0 & 0 & 1 & 0 & 1 & 0 \\ 0 & 0 & 0 & 1 & 1 & 0 & 1 \\ 1 & 1 & 1 & 0 & 0 & 0 & 0 \\ 0 & 1 & 0 & 1 & 1 & 0 & 0 \\ 1 & 0 & 0 & 0 & 0 & 0 & 0 \\ 0 & 1 & 1 & 0 & 0 & 1 & 1 \end{pmatrix}$ | 1  |
| 114. | $x^2y^{-5}$ | $s_1s_1s_1s_3s_1s_3s_3$ | $\begin{pmatrix} 0 & 1 & 0 & 0 & 0 & 1 & 0 \\ 0 & 0 & 1 & 0 & 0 & 1 & 0 \\ 1 & 1 & 1 & 0 & 0 & 0 & 1 \\ 1 & 0 & 0 & 1 & 1 & 0 & 0 \\ 0 & 0 & 1 & 0 & 1 & 0 & 0 \\ 1 & 0 & 0 & 0 & 0 & 0 & 0 \\ 0 & 1 & 0 & 1 & 1 & 0 & 1 \end{pmatrix}$ | 1  |
| 115. | $x^2y^{13}$ | $s_2s_4s_1s_4s_2s_4s_2$ | $\begin{pmatrix} 0 & 0 & 1 & 1 & 0 & 0 & 0 \\ 1 & 0 & 0 & 0 & 0 & 0 & 0 \\ 1 & 1 & 1 & 0 & 1 & 0 & 1 \\ 0 & 0 & 0 & 1 & 0 & 0 & 1 \\ 1 & 1 & 0 & 0 & 1 & 1 & 0 \\ 0 & 0 & 1 & 0 & 1 & 1 & 0 \\ 0 & 0 & 0 & 0 & 0 & 0 & 1 \end{pmatrix}$ | -1 |
| 116. | $x^6y$      | $s_1s_3s_2s_4s_2s_3s_1$ | $\begin{pmatrix} 0 & 1 & 1 & 1 & 0 & 1 & 1 \\ 0 & 0 & 0 & 0 & 1 & 0 & 0 \\ 1 & 0 & 1 & 0 & 1 & 0 & 0 \\ 0 & 1 & 0 & 0 & 0 & 0 & 0 \\ 1 & 0 & 0 & 0 & 0 & 0 & 1 \\ 1 & 0 & 1 & 1 & 0 & 0 & 0 \\ 0 & 0 & 0 & 0 & 1 & 1 & 1 \end{pmatrix}$ | -1 |
| 117. | $x^4y^{-9}$ | $s_1s_4s_4s_2s_3s_2s_2$ | $\begin{pmatrix} 1 & 0 & 1 & 0 & 1 & 0 & 0 \\ 0 & 0 & 0 & 1 & 0 & 1 & 0 \\ 1 & 1 & 0 & 1 & 0 & 0 & 1 \\ 0 & 0 & 0 & 0 & 0 & 0 & 1 \\ 0 & 1 & 0 & 0 & 0 & 0 & 0 \\ 0 & 0 & 1 & 0 & 0 & 1 & 0 \\ 1 & 0 & 0 & 1 & 1 & 1 & 1 \end{pmatrix}$ | 1  |

|      |             |                         |                                                                                                                                                                                                                                         |    |
|------|-------------|-------------------------|-----------------------------------------------------------------------------------------------------------------------------------------------------------------------------------------------------------------------------------------|----|
| 118. | $x^5y^3$    | $s_2s_2s_3s_3s_1s_3s_1$ | $\begin{pmatrix} 0 & 0 & 0 & 0 & 0 & 1 & 1 \\ 0 & 0 & 0 & 1 & 1 & 0 & 0 \\ 1 & 0 & 1 & 0 & 0 & 0 & 0 \\ 0 & 1 & 1 & 0 & 0 & 0 & 0 \\ 1 & 0 & 0 & 1 & 1 & 0 & 1 \\ 1 & 1 & 0 & 0 & 1 & 0 & 0 \\ 0 & 1 & 0 & 0 & 0 & 1 & 1 \end{pmatrix}$ | 1  |
| 119. | $x^5y^{-3}$ | $s_1s_4s_2s_2s_4s_4s_1$ | $\begin{pmatrix} 1 & 0 & 1 & 0 & 0 & 0 & 1 \\ 1 & 0 & 1 & 1 & 1 & 0 & 0 \\ 0 & 0 & 0 & 1 & 1 & 0 & 0 \\ 0 & 0 & 1 & 0 & 0 & 1 & 0 \\ 0 & 0 & 0 & 0 & 0 & 1 & 1 \\ 1 & 1 & 0 & 0 & 0 & 0 & 0 \\ 0 & 1 & 0 & 1 & 0 & 0 & 1 \end{pmatrix}$ | 1  |
| 120. | $x^6y^9$    | $s_1s_4s_2s_3s_1s_3s_1$ | $\begin{pmatrix} 0 & 1 & 0 & 0 & 0 & 1 & 1 \\ 1 & 0 & 1 & 1 & 1 & 0 & 0 \\ 0 & 0 & 1 & 0 & 0 & 0 & 0 \\ 1 & 0 & 1 & 0 & 0 & 0 & 0 \\ 1 & 1 & 0 & 1 & 1 & 0 & 1 \\ 0 & 0 & 0 & 0 & 1 & 0 & 0 \\ 0 & 0 & 0 & 0 & 0 & 1 & 1 \end{pmatrix}$ | 1  |
| 121. | $x^6y^{14}$ | $s_2s_2s_4s_2s_2s_4s_2$ | $\begin{pmatrix} 0 & 0 & 0 & 1 & 0 & 0 & 0 \\ 0 & 1 & 0 & 1 & 0 & 0 & 0 \\ 0 & 1 & 1 & 0 & 1 & 0 & 1 \\ 1 & 1 & 1 & 0 & 0 & 0 & 1 \\ 1 & 0 & 0 & 0 & 1 & 1 & 0 \\ 0 & 0 & 0 & 1 & 1 & 1 & 0 \\ 1 & 0 & 0 & 0 & 0 & 0 & 1 \end{pmatrix}$ | -1 |
| 122. | $xy^2$      | $s_1s_1s_1s_3s_2s_3s_1$ | $\begin{pmatrix} 0 & 0 & 1 & 0 & 0 & 1 & 1 \\ 1 & 0 & 0 & 1 & 1 & 0 & 0 \\ 1 & 1 & 1 & 0 & 1 & 0 & 0 \\ 0 & 1 & 0 & 1 & 0 & 0 & 0 \\ 1 & 0 & 0 & 0 & 0 & 0 & 1 \\ 0 & 1 & 0 & 0 & 0 & 0 & 0 \\ 0 & 0 & 1 & 0 & 1 & 1 & 1 \end{pmatrix}$ | -1 |
| 123. | $xy^{-4}$   | $s_1s_1s_3s_2s_3s_3s_3$ | $\begin{pmatrix} 0 & 0 & 0 & 0 & 0 & 1 & 0 \\ 1 & 0 & 1 & 0 & 0 & 1 & 0 \\ 1 & 1 & 0 & 1 & 0 & 0 & 1 \\ 0 & 1 & 0 & 1 & 1 & 0 & 0 \\ 1 & 0 & 0 & 0 & 0 & 0 & 0 \\ 0 & 1 & 0 & 0 & 1 & 0 & 0 \\ 0 & 0 & 1 & 1 & 0 & 0 & 1 \end{pmatrix}$ | -1 |
| 124. | $x^3y^8$    | $s_1s_1s_1s_4s_1s_3s_1$ | $\begin{pmatrix} 0 & 0 & 1 & 0 & 0 & 1 & 1 \\ 0 & 0 & 1 & 0 & 1 & 0 & 0 \\ 0 & 1 & 0 & 0 & 0 & 0 & 0 \\ 1 & 0 & 0 & 0 & 0 & 0 & 0 \\ 0 & 1 & 0 & 0 & 1 & 0 & 1 \\ 1 & 1 & 1 & 1 & 1 & 0 & 0 \\ 1 & 0 & 0 & 1 & 0 & 1 & 1 \end{pmatrix}$ | 1  |

|      |             |                         |                                                                                                                                                                                                                                         |    |
|------|-------------|-------------------------|-----------------------------------------------------------------------------------------------------------------------------------------------------------------------------------------------------------------------------------------|----|
| 125. | $x^2y^{-2}$ | $s_1s_3s_1s_1s_4s_4s_4$ | $\begin{pmatrix} 0 & 0 & 0 & 1 & 0 & 1 & 0 \\ 0 & 1 & 1 & 0 & 0 & 1 & 0 \\ 1 & 0 & 0 & 0 & 1 & 0 & 0 \\ 1 & 0 & 0 & 0 & 0 & 0 & 1 \\ 0 & 0 & 0 & 1 & 0 & 0 & 0 \\ 1 & 0 & 1 & 0 & 0 & 0 & 1 \\ 0 & 1 & 1 & 1 & 1 & 0 & 0 \end{pmatrix}$ | 1  |
| 126. | $x^6y^{10}$ | $s_1s_3s_1s_3s_1s_1s_1$ | $\begin{pmatrix} 0 & 1 & 1 & 0 & 0 & 0 & 1 \\ 0 & 0 & 0 & 0 & 0 & 1 & 0 \\ 1 & 0 & 0 & 1 & 1 & 0 & 0 \\ 0 & 1 & 1 & 0 & 1 & 0 & 0 \\ 1 & 0 & 1 & 0 & 0 & 0 & 1 \\ 1 & 0 & 0 & 0 & 0 & 1 & 0 \\ 0 & 0 & 0 & 1 & 1 & 1 & 1 \end{pmatrix}$ | 1  |
| 127. | $x^6y^4$    | $s_1s_3s_3s_1s_3s_3s_1$ | $\begin{pmatrix} 0 & 1 & 0 & 0 & 0 & 1 & 1 \\ 0 & 0 & 0 & 0 & 1 & 0 & 0 \\ 1 & 0 & 0 & 0 & 1 & 0 & 0 \\ 0 & 1 & 0 & 0 & 0 & 0 & 0 \\ 1 & 0 & 1 & 1 & 0 & 0 & 1 \\ 1 & 0 & 0 & 1 & 0 & 0 & 0 \\ 0 & 0 & 1 & 1 & 0 & 1 & 1 \end{pmatrix}$ | 1  |
| 128. | $x^3y^{-8}$ | $s_1s_1s_1s_4s_2s_2s_3$ | $\begin{pmatrix} 0 & 0 & 1 & 0 & 1 & 1 & 0 \\ 0 & 1 & 0 & 0 & 0 & 1 & 0 \\ 0 & 0 & 1 & 0 & 1 & 0 & 1 \\ 0 & 1 & 0 & 0 & 0 & 0 & 0 \\ 1 & 1 & 1 & 1 & 0 & 0 & 0 \\ 1 & 0 & 0 & 0 & 1 & 0 & 0 \\ 1 & 0 & 0 & 1 & 0 & 1 & 1 \end{pmatrix}$ | 1  |
| 129. | $x^5y^6$    | $s_4s_1s_3s_2s_4s_2s_4$ | $\begin{pmatrix} 0 & 0 & 0 & 0 & 0 & 1 & 0 \\ 1 & 0 & 1 & 1 & 1 & 0 & 0 \\ 0 & 0 & 1 & 0 & 0 & 0 & 0 \\ 0 & 0 & 0 & 0 & 0 & 1 & 1 \\ 0 & 1 & 0 & 1 & 1 & 0 & 0 \\ 1 & 1 & 0 & 1 & 0 & 1 & 1 \\ 0 & 1 & 0 & 0 & 0 & 0 & 0 \end{pmatrix}$ | 1  |
| 130. | $x^6y^{-6}$ | $s_1s_3s_2s_2s_3s_1s_1$ | $\begin{pmatrix} 0 & 0 & 0 & 1 & 0 & 0 & 1 \\ 1 & 0 & 1 & 0 & 1 & 1 & 0 \\ 0 & 1 & 1 & 1 & 0 & 0 & 0 \\ 1 & 0 & 0 & 0 & 0 & 0 & 0 \\ 1 & 0 & 1 & 0 & 0 & 0 & 1 \\ 0 & 1 & 0 & 0 & 0 & 1 & 0 \\ 0 & 0 & 0 & 1 & 1 & 1 & 1 \end{pmatrix}$ | -1 |
| 131. | $x^6y^{12}$ | $s_1s_3s_2s_3s_3s_2s_3$ | $\begin{pmatrix} 0 & 0 & 0 & 0 & 1 & 1 & 0 \\ 1 & 0 & 1 & 1 & 0 & 1 & 0 \\ 0 & 1 & 1 & 0 & 0 & 0 & 1 \\ 1 & 0 & 0 & 1 & 0 & 0 & 0 \\ 1 & 0 & 1 & 0 & 0 & 0 & 0 \\ 0 & 1 & 0 & 0 & 1 & 0 & 0 \\ 0 & 0 & 0 & 0 & 0 & 1 & 1 \end{pmatrix}$ | 1  |

|      |             |                         |                                                                                                                                                                                                                                         |    |
|------|-------------|-------------------------|-----------------------------------------------------------------------------------------------------------------------------------------------------------------------------------------------------------------------------------------|----|
| 132. | $x^6y^{-1}$ | $s_1s_3s_1s_4s_4s_2s_2$ | $\begin{pmatrix} 1 & 0 & 0 & 0 & 0 & 0 & 0 \\ 0 & 1 & 1 & 1 & 0 & 1 & 0 \\ 0 & 0 & 0 & 1 & 0 & 0 & 1 \\ 1 & 0 & 0 & 0 & 1 & 0 & 1 \\ 0 & 1 & 1 & 0 & 1 & 0 & 0 \\ 1 & 0 & 1 & 0 & 0 & 1 & 0 \\ 0 & 0 & 0 & 0 & 0 & 1 & 1 \end{pmatrix}$ | 1  |
| 133. | $xy^{11}$   | $s_1s_3s_2s_3s_1s_3s_1$ | $\begin{pmatrix} 0 & 0 & 0 & 0 & 0 & 1 & 1 \\ 1 & 0 & 1 & 1 & 1 & 0 & 0 \\ 1 & 0 & 1 & 0 & 0 & 0 & 0 \\ 0 & 1 & 1 & 0 & 0 & 0 & 0 \\ 1 & 0 & 0 & 1 & 1 & 0 & 1 \\ 0 & 0 & 0 & 0 & 1 & 0 & 0 \\ 0 & 1 & 0 & 0 & 0 & 1 & 1 \end{pmatrix}$ | 1  |
| 134. | $xy^5$      | $s_2s_2s_4s_4s_2s_2s_4$ | $\begin{pmatrix} 1 & 0 & 0 & 1 & 0 & 1 & 0 \\ 0 & 0 & 0 & 0 & 1 & 0 & 0 \\ 1 & 1 & 1 & 0 & 1 & 0 & 0 \\ 0 & 1 & 0 & 0 & 1 & 1 & 1 \\ 0 & 0 & 0 & 1 & 0 & 0 & 0 \\ 0 & 1 & 1 & 0 & 0 & 1 & 1 \\ 1 & 0 & 0 & 0 & 0 & 0 & 0 \end{pmatrix}$ | 1  |
| 135. | $x^3y^{-7}$ | $s_2s_2s_3s_2s_3s_1s_4$ | $\begin{pmatrix} 1 & 0 & 1 & 0 & 0 & 0 & 0 \\ 1 & 0 & 0 & 0 & 0 & 0 & 0 \\ 0 & 1 & 1 & 1 & 0 & 0 & 0 \\ 0 & 0 & 0 & 1 & 1 & 1 & 1 \\ 0 & 1 & 0 & 0 & 0 & 1 & 0 \\ 1 & 1 & 0 & 1 & 0 & 0 & 1 \\ 0 & 0 & 0 & 0 & 1 & 1 & 0 \end{pmatrix}$ | 1  |
| 136. | $x^2y^7$    | $s_1s_4s_2s_3s_1s_1s_4$ | $\begin{pmatrix} 0 & 1 & 0 & 0 & 0 & 0 & 0 \\ 0 & 0 & 0 & 0 & 1 & 0 & 0 \\ 1 & 1 & 0 & 1 & 1 & 0 & 0 \\ 1 & 0 & 1 & 1 & 1 & 1 & 1 \\ 0 & 0 & 0 & 0 & 0 & 1 & 0 \\ 1 & 0 & 1 & 0 & 0 & 0 & 1 \\ 0 & 0 & 1 & 0 & 0 & 1 & 0 \end{pmatrix}$ | -1 |
| 137. | $x^6y^{-5}$ | $s_1s_1s_3s_3s_1s_3s_1$ | $\begin{pmatrix} 0 & 1 & 0 & 0 & 0 & 1 & 1 \\ 0 & 1 & 0 & 1 & 1 & 0 & 0 \\ 1 & 0 & 1 & 0 & 0 & 0 & 0 \\ 0 & 0 & 1 & 0 & 0 & 0 & 0 \\ 1 & 0 & 0 & 1 & 1 & 0 & 1 \\ 1 & 1 & 0 & 0 & 1 & 0 & 0 \\ 0 & 0 & 0 & 0 & 0 & 1 & 1 \end{pmatrix}$ | -1 |
| 138. | $x^6y^{13}$ | $s_2s_2s_4s_2s_4s_1s_4$ | $\begin{pmatrix} 0 & 1 & 0 & 1 & 1 & 0 & 0 \\ 0 & 1 & 1 & 0 & 0 & 0 & 0 \\ 0 & 0 & 0 & 1 & 0 & 0 & 0 \\ 1 & 0 & 0 & 0 & 0 & 1 & 1 \\ 0 & 0 & 0 & 1 & 1 & 1 & 0 \\ 1 & 1 & 1 & 0 & 0 & 0 & 1 \\ 1 & 0 & 0 & 0 & 0 & 1 & 0 \end{pmatrix}$ | -1 |



|      |             |                         |                                                                                                                                                                                                                                         |    |
|------|-------------|-------------------------|-----------------------------------------------------------------------------------------------------------------------------------------------------------------------------------------------------------------------------------------|----|
| 139. | $x^3y$      | $s_1s_1s_3s_3s_2s_2s_4$ | $\begin{pmatrix} 0 & 0 & 0 & 0 & 0 & 1 & 0 \\ 0 & 1 & 0 & 0 & 1 & 0 & 0 \\ 0 & 0 & 1 & 0 & 1 & 0 & 0 \\ 0 & 1 & 0 & 1 & 1 & 1 & 1 \\ 1 & 1 & 0 & 0 & 0 & 0 & 0 \\ 1 & 0 & 1 & 0 & 0 & 1 & 1 \\ 1 & 0 & 0 & 1 & 0 & 0 & 0 \end{pmatrix}$ | -1 |
| 140. | $x^5y^{-9}$ | $s_1s_1s_1s_3s_1s_4s_4$ | $\begin{pmatrix} 1 & 0 & 0 & 1 & 1 & 1 & 0 \\ 1 & 0 & 0 & 0 & 0 & 1 & 0 \\ 0 & 0 & 1 & 0 & 0 & 0 & 0 \\ 0 & 1 & 0 & 1 & 1 & 0 & 1 \\ 0 & 0 & 1 & 0 & 1 & 0 & 0 \\ 1 & 1 & 1 & 0 & 0 & 0 & 1 \\ 0 & 1 & 0 & 0 & 0 & 0 & 0 \end{pmatrix}$ | 1  |
| 141. | $x^6y^3$    | $s_1s_1s_3s_2s_3s_3s_2$ | $\begin{pmatrix} 0 & 1 & 0 & 0 & 1 & 0 & 0 \\ 1 & 0 & 1 & 0 & 0 & 1 & 0 \\ 0 & 1 & 0 & 1 & 1 & 0 & 1 \\ 1 & 0 & 0 & 0 & 0 & 0 & 1 \\ 1 & 1 & 0 & 1 & 0 & 0 & 0 \\ 0 & 0 & 1 & 1 & 0 & 0 & 0 \\ 0 & 0 & 0 & 0 & 0 & 1 & 1 \end{pmatrix}$ | -1 |
| 142. | $x^6y^{-3}$ | $s_1s_1s_4s_2s_2s_4s_4$ | $\begin{pmatrix} 0 & 1 & 0 & 1 & 1 & 1 & 0 \\ 1 & 0 & 0 & 0 & 1 & 1 & 0 \\ 0 & 1 & 0 & 1 & 0 & 0 & 0 \\ 1 & 0 & 0 & 0 & 0 & 0 & 1 \\ 1 & 1 & 1 & 0 & 0 & 0 & 0 \\ 0 & 0 & 0 & 1 & 0 & 0 & 1 \\ 0 & 0 & 1 & 0 & 1 & 0 & 0 \end{pmatrix}$ | 1  |
| 143. | $xy^{14}$   | $s_1s_1s_3s_2s_4s_4s_4$ | $\begin{pmatrix} 0 & 0 & 0 & 0 & 0 & 1 & 0 \\ 1 & 0 & 1 & 0 & 0 & 1 & 0 \\ 1 & 1 & 0 & 1 & 1 & 0 & 0 \\ 0 & 1 & 0 & 1 & 0 & 0 & 1 \\ 1 & 0 & 0 & 0 & 0 & 0 & 0 \\ 0 & 1 & 0 & 0 & 0 & 0 & 1 \\ 0 & 0 & 1 & 1 & 1 & 0 & 0 \end{pmatrix}$ | 1  |
| 144. | $x^3y^2$    | $s_1s_3s_1s_1s_1s_3s_2$ | $\begin{pmatrix} 0 & 1 & 1 & 0 & 0 & 0 & 0 \\ 0 & 0 & 0 & 1 & 0 & 1 & 0 \\ 0 & 1 & 1 & 1 & 1 & 0 & 1 \\ 1 & 0 & 0 & 0 & 1 & 0 & 1 \\ 0 & 0 & 0 & 1 & 0 & 0 & 0 \\ 1 & 0 & 0 & 0 & 1 & 0 & 0 \\ 1 & 0 & 1 & 0 & 0 & 1 & 1 \end{pmatrix}$ | -1 |
| 145. | $x^3y^{-4}$ | $s_1s_4s_1s_4s_4s_4s_1$ | $\begin{pmatrix} 0 & 0 & 0 & 1 & 0 & 0 & 1 \\ 0 & 0 & 1 & 0 & 1 & 0 & 0 \\ 0 & 0 & 0 & 0 & 1 & 0 & 0 \\ 1 & 0 & 0 & 0 & 0 & 1 & 0 \\ 0 & 1 & 0 & 0 & 0 & 1 & 1 \\ 1 & 1 & 1 & 0 & 0 & 0 & 0 \\ 1 & 0 & 1 & 1 & 0 & 0 & 1 \end{pmatrix}$ | 1  |

|      |             |                         |                                                                                                                                                                                                                                         |    |
|------|-------------|-------------------------|-----------------------------------------------------------------------------------------------------------------------------------------------------------------------------------------------------------------------------------------|----|
| 146. | $x^5y^8$    | $s_1s_3s_1s_1s_4s_1s_1$ | $\begin{pmatrix} 1 & 0 & 1 & 0 & 0 & 0 & 1 \\ 0 & 1 & 1 & 0 & 0 & 1 & 0 \\ 1 & 0 & 0 & 0 & 0 & 0 & 0 \\ 0 & 0 & 0 & 1 & 0 & 0 & 0 \\ 1 & 0 & 0 & 0 & 1 & 0 & 1 \\ 0 & 1 & 1 & 1 & 1 & 1 & 0 \\ 0 & 0 & 0 & 1 & 0 & 1 & 1 \end{pmatrix}$ | -1 |
| 147. | $x^6y^{-2}$ | $s_2s_4s_2s_4s_4s_2s_3$ | $\begin{pmatrix} 0 & 0 & 1 & 0 & 0 & 1 & 0 \\ 0 & 0 & 1 & 1 & 0 & 1 & 0 \\ 0 & 0 & 0 & 0 & 1 & 0 & 1 \\ 1 & 0 & 1 & 1 & 0 & 0 & 0 \\ 0 & 0 & 0 & 0 & 1 & 0 & 0 \\ 1 & 1 & 0 & 0 & 0 & 0 & 0 \\ 1 & 1 & 0 & 0 & 0 & 1 & 1 \end{pmatrix}$ | -1 |
| 148. | $x^3y^{10}$ | $s_1s_3s_1s_1s_1s_3s_1$ | $\begin{pmatrix} 0 & 0 & 0 & 1 & 0 & 1 & 1 \\ 0 & 1 & 1 & 1 & 1 & 0 & 0 \\ 0 & 1 & 1 & 0 & 0 & 0 & 0 \\ 0 & 0 & 0 & 1 & 0 & 0 & 0 \\ 1 & 0 & 0 & 0 & 1 & 0 & 1 \\ 1 & 0 & 0 & 0 & 1 & 0 & 0 \\ 1 & 0 & 1 & 0 & 0 & 1 & 1 \end{pmatrix}$ | 1  |
| 149. | $x^3y^4$    | $s_1s_4s_2s_2s_4s_4s_4$ | $\begin{pmatrix} 0 & 0 & 0 & 0 & 0 & 1 & 0 \\ 0 & 0 & 1 & 0 & 0 & 1 & 0 \\ 0 & 0 & 0 & 1 & 1 & 0 & 0 \\ 0 & 1 & 0 & 1 & 0 & 0 & 1 \\ 1 & 1 & 0 & 0 & 0 & 0 & 0 \\ 1 & 0 & 1 & 0 & 0 & 0 & 1 \\ 1 & 0 & 1 & 1 & 1 & 0 & 0 \end{pmatrix}$ | 1  |
| 150. | $x^6y^6$    | $s_1s_4s_1s_4s_1s_1s_1$ | $\begin{pmatrix} 0 & 1 & 0 & 0 & 0 & 0 & 1 \\ 1 & 0 & 0 & 0 & 0 & 1 & 0 \\ 0 & 0 & 0 & 0 & 1 & 0 & 0 \\ 1 & 0 & 1 & 1 & 1 & 0 & 0 \\ 1 & 1 & 1 & 0 & 0 & 0 & 1 \\ 0 & 0 & 0 & 1 & 0 & 1 & 0 \\ 0 & 0 & 1 & 0 & 1 & 1 & 1 \end{pmatrix}$ | 1  |
| 151. | $xy^{-1}$   | $s_1s_4s_2s_2s_4s_1s_3$ | $\begin{pmatrix} 0 & 0 & 0 & 0 & 0 & 1 & 0 \\ 1 & 0 & 1 & 0 & 0 & 0 & 0 \\ 1 & 1 & 0 & 0 & 0 & 0 & 1 \\ 0 & 0 & 1 & 0 & 0 & 1 & 0 \\ 1 & 0 & 1 & 1 & 1 & 1 & 0 \\ 0 & 1 & 0 & 1 & 0 & 0 & 0 \\ 0 & 0 & 0 & 1 & 1 & 0 & 1 \end{pmatrix}$ | 1  |
| 152. | $x^3y^{11}$ | $s_1s_3s_1s_3s_2s_3s_1$ | $\begin{pmatrix} 0 & 1 & 1 & 0 & 0 & 1 & 1 \\ 0 & 0 & 0 & 1 & 1 & 0 & 0 \\ 0 & 1 & 1 & 0 & 1 & 0 & 0 \\ 1 & 0 & 0 & 1 & 0 & 0 & 0 \\ 0 & 0 & 0 & 0 & 0 & 0 & 1 \\ 1 & 0 & 0 & 0 & 0 & 0 & 0 \\ 1 & 0 & 1 & 0 & 1 & 1 & 1 \end{pmatrix}$ | 1  |

|      |             |                         |                                                                                                                                                                                                                                         |    |
|------|-------------|-------------------------|-----------------------------------------------------------------------------------------------------------------------------------------------------------------------------------------------------------------------------------------|----|
| 153. | $x^3y^5$    | $s_1s_1s_1s_4s_4s_2s_4$ | $\begin{pmatrix} 0 & 0 & 1 & 0 & 0 & 1 & 0 \\ 0 & 0 & 1 & 0 & 1 & 0 & 0 \\ 0 & 1 & 0 & 0 & 0 & 0 & 0 \\ 1 & 0 & 0 & 0 & 0 & 1 & 1 \\ 0 & 1 & 0 & 0 & 1 & 0 & 0 \\ 1 & 1 & 1 & 1 & 0 & 1 & 1 \\ 1 & 0 & 0 & 1 & 0 & 0 & 0 \end{pmatrix}$ | 1  |
| 154. | $x^5y^{-7}$ | $s_1s_1s_1s_4s_1s_3s_3$ | $\begin{pmatrix} 1 & 0 & 0 & 1 & 0 & 1 & 0 \\ 0 & 0 & 1 & 0 & 0 & 1 & 0 \\ 1 & 0 & 0 & 0 & 0 & 0 & 1 \\ 0 & 0 & 1 & 0 & 1 & 0 & 0 \\ 1 & 1 & 1 & 1 & 1 & 0 & 0 \\ 0 & 1 & 0 & 0 & 0 & 0 & 0 \\ 0 & 1 & 0 & 0 & 1 & 0 & 1 \end{pmatrix}$ | 1  |
| 155. | $x^6y^7$    | $s_4s_4s_4s_1s_3s_1s_3$ | $\begin{pmatrix} 0 & 0 & 1 & 0 & 1 & 1 & 0 \\ 0 & 1 & 0 & 0 & 0 & 0 & 0 \\ 0 & 0 & 1 & 1 & 0 & 0 & 1 \\ 0 & 0 & 0 & 0 & 1 & 1 & 0 \\ 1 & 0 & 0 & 1 & 0 & 1 & 0 \\ 1 & 0 & 0 & 1 & 0 & 0 & 0 \\ 0 & 1 & 0 & 0 & 0 & 0 & 1 \end{pmatrix}$ | 1  |
| 156. | $x^3y^{-5}$ | $s_2s_2s_3s_1s_3s_2s_3$ | $\begin{pmatrix} 1 & 0 & 0 & 0 & 1 & 1 & 0 \\ 0 & 1 & 1 & 1 & 0 & 1 & 0 \\ 1 & 0 & 1 & 1 & 0 & 0 & 1 \\ 0 & 1 & 0 & 0 & 0 & 0 & 0 \\ 1 & 1 & 0 & 0 & 0 & 0 & 0 \\ 0 & 0 & 0 & 0 & 1 & 0 & 0 \\ 0 & 0 & 0 & 1 & 0 & 1 & 1 \end{pmatrix}$ | -1 |
| 157. | $x^3y^{13}$ | $s_2s_4s_2s_4s_1s_4s_2$ | $\begin{pmatrix} 1 & 1 & 0 & 0 & 0 & 0 & 0 \\ 0 & 0 & 1 & 0 & 0 & 0 & 0 \\ 1 & 0 & 1 & 1 & 0 & 0 & 1 \\ 0 & 0 & 1 & 1 & 1 & 0 & 1 \\ 1 & 1 & 0 & 0 & 0 & 1 & 0 \\ 0 & 0 & 0 & 0 & 1 & 1 & 0 \\ 0 & 0 & 0 & 0 & 1 & 0 & 1 \end{pmatrix}$ | -1 |
| 158. | $x^6y^{-9}$ | $s_1s_4s_4s_1s_3s_1s_1$ | $\begin{pmatrix} 0 & 1 & 0 & 0 & 0 & 0 & 1 \\ 1 & 0 & 0 & 0 & 1 & 1 & 0 \\ 0 & 0 & 0 & 1 & 0 & 0 & 0 \\ 1 & 0 & 1 & 1 & 0 & 0 & 0 \\ 1 & 1 & 0 & 0 & 0 & 0 & 1 \\ 0 & 0 & 0 & 1 & 0 & 1 & 0 \\ 0 & 0 & 1 & 0 & 1 & 1 & 1 \end{pmatrix}$ | -1 |
| 159. | $x^3y^{14}$ | $s_3s_1s_4s_1s_4s_4s_2$ | $\begin{pmatrix} 0 & 0 & 0 & 0 & 1 & 0 & 0 \\ 0 & 1 & 0 & 0 & 0 & 0 & 0 \\ 1 & 1 & 0 & 1 & 1 & 0 & 1 \\ 1 & 1 & 1 & 1 & 0 & 0 & 1 \\ 0 & 0 & 0 & 0 & 0 & 1 & 0 \\ 0 & 0 & 0 & 1 & 0 & 1 & 0 \\ 0 & 0 & 1 & 0 & 0 & 0 & 1 \end{pmatrix}$ | 1  |

|      |             |                         |                                                                                                                                                                                                                                         |    |
|------|-------------|-------------------------|-----------------------------------------------------------------------------------------------------------------------------------------------------------------------------------------------------------------------------------------|----|
| 160. | $x^5y^2$    | $s_1s_3s_3s_3s_1s_4s_1$ | $\begin{pmatrix} 1 & 0 & 1 & 0 & 0 & 0 & 1 \\ 0 & 1 & 0 & 0 & 0 & 0 & 0 \\ 1 & 0 & 0 & 0 & 0 & 0 & 0 \\ 0 & 0 & 1 & 0 & 0 & 1 & 0 \\ 1 & 0 & 0 & 1 & 1 & 1 & 1 \\ 0 & 1 & 0 & 0 & 1 & 0 & 0 \\ 0 & 0 & 0 & 1 & 1 & 0 & 1 \end{pmatrix}$ | 1  |
| 161. | $x^5y^{-4}$ | $s_1s_3s_1s_3s_2s_3s_3$ | $\begin{pmatrix} 1 & 0 & 1 & 0 & 1 & 1 & 0 \\ 0 & 1 & 1 & 0 & 0 & 1 & 0 \\ 1 & 0 & 0 & 1 & 0 & 0 & 1 \\ 0 & 0 & 0 & 1 & 1 & 0 & 0 \\ 1 & 0 & 0 & 0 & 0 & 0 & 0 \\ 0 & 1 & 1 & 0 & 1 & 0 & 0 \\ 0 & 0 & 0 & 0 & 0 & 0 & 1 \end{pmatrix}$ | 1  |
| 162. | $x^3y^{-2}$ | $s_2s_4s_1s_4s_1s_1s_1$ | $\begin{pmatrix} 1 & 1 & 0 & 0 & 0 & 0 & 1 \\ 0 & 0 & 0 & 0 & 0 & 1 & 0 \\ 1 & 0 & 0 & 0 & 1 & 0 & 0 \\ 0 & 0 & 1 & 1 & 1 & 0 & 0 \\ 1 & 1 & 1 & 0 & 0 & 0 & 1 \\ 0 & 0 & 0 & 1 & 0 & 1 & 0 \\ 0 & 0 & 1 & 0 & 1 & 1 & 1 \end{pmatrix}$ | -1 |
| 163. | $x^3y^{-1}$ | $s_4s_2s_4s_2s_3s_1s_1$ | $\begin{pmatrix} 0 & 1 & 0 & 1 & 0 & 0 & 1 \\ 0 & 1 & 1 & 0 & 1 & 1 & 0 \\ 0 & 0 & 0 & 1 & 0 & 0 & 0 \\ 0 & 1 & 1 & 0 & 0 & 0 & 0 \\ 0 & 0 & 0 & 0 & 0 & 0 & 1 \\ 1 & 0 & 0 & 0 & 0 & 1 & 0 \\ 1 & 0 & 0 & 1 & 1 & 1 & 1 \end{pmatrix}$ | 1  |
| 164. | $x^5y^{11}$ | $s_1s_3s_1s_1s_3s_3s_2$ | $\begin{pmatrix} 1 & 0 & 1 & 0 & 1 & 0 & 0 \\ 0 & 1 & 1 & 0 & 0 & 1 & 0 \\ 1 & 0 & 0 & 0 & 1 & 0 & 1 \\ 0 & 0 & 0 & 1 & 0 & 0 & 1 \\ 1 & 0 & 0 & 0 & 0 & 0 & 0 \\ 0 & 1 & 1 & 1 & 0 & 0 & 0 \\ 0 & 0 & 0 & 1 & 0 & 1 & 1 \end{pmatrix}$ | 1  |
| 165. | $x^5y^5$    | $s_1s_4s_4s_2s_4s_1s_1$ | $\begin{pmatrix} 1 & 0 & 1 & 0 & 0 & 0 & 1 \\ 0 & 0 & 0 & 0 & 0 & 1 & 0 \\ 1 & 0 & 0 & 1 & 0 & 0 & 0 \\ 0 & 0 & 1 & 0 & 0 & 0 & 0 \\ 1 & 1 & 0 & 1 & 1 & 0 & 1 \\ 0 & 0 & 0 & 1 & 1 & 1 & 0 \\ 0 & 1 & 0 & 0 & 0 & 1 & 1 \end{pmatrix}$ | -1 |
| 166. | $x^3y^7$    | $s_1s_1s_3s_1s_4s_4s_2$ | $\begin{pmatrix} 0 & 0 & 0 & 0 & 1 & 0 & 0 \\ 0 & 1 & 0 & 0 & 0 & 0 & 0 \\ 0 & 0 & 1 & 1 & 1 & 0 & 1 \\ 0 & 1 & 0 & 1 & 0 & 0 & 1 \\ 1 & 1 & 0 & 0 & 0 & 1 & 0 \\ 1 & 0 & 1 & 1 & 0 & 1 & 0 \\ 1 & 0 & 0 & 0 & 0 & 0 & 1 \end{pmatrix}$ | 1  |

$$167. \quad x^5 y^{14} \quad s_1 s_4 s_4 s_1 s_3 s_2 s_4 \quad \begin{pmatrix} 1 & 0 & 1 & 1 & 0 & 1 & 0 \\ 0 & 0 & 0 & 1 & 0 & 0 & 0 \\ 1 & 0 & 0 & 0 & 1 & 0 & 0 \\ 0 & 0 & 1 & 0 & 1 & 1 & 1 \\ 1 & 1 & 0 & 0 & 0 & 0 & 0 \\ 0 & 0 & 0 & 1 & 0 & 1 & 1 \\ 0 & 1 & 0 & 0 & 0 & 0 & 0 \end{pmatrix} \quad 1$$

$$168. \quad x^5 y^{-1} \quad s_2 s_3 s_1 s_1 s_4 s_2 s_4 \quad \begin{pmatrix} 0 & 0 & 0 & 1 & 0 & 1 & 0 \\ 1 & 1 & 1 & 1 & 1 & 0 & 0 \\ 0 & 1 & 1 & 0 & 0 & 0 & 0 \\ 1 & 0 & 0 & 1 & 0 & 1 & 1 \\ 1 & 0 & 0 & 0 & 1 & 0 & 0 \\ 0 & 0 & 0 & 0 & 0 & 1 & 1 \\ 0 & 0 & 1 & 0 & 0 & 0 & 0 \end{pmatrix} \quad -1$$

## Solution for directed graphs of diameter 3

|                               |                                                                                                          |
|-------------------------------|----------------------------------------------------------------------------------------------------------|
| Diameter                      | 3                                                                                                        |
| Set size                      | 4                                                                                                        |
| Group $K$                     | $\mathbb{Z}_2 \times S_4$ (order 48; id 48)<br>$\langle x, y \mid x^4, y^6, (yx)^2, (y^{-2}x)^2 \rangle$ |
| $\varphi : K \rightarrow S_3$ | $x \mapsto (2\ 3)$<br>$y \mapsto (1\ 2\ 3)$                                                              |
| Set $S$                       | $\{s_1, s_2, s_3, s_4\} =$<br>$\{x^2yx^3y, y^4, x^3, x^2y\}$                                             |
| Set $V$                       | $\{110, 010, 110, 010\}$                                                                                 |

| No. | Element      | Product     | Mapping matrix $M$                                                  | $\det M$ |
|-----|--------------|-------------|---------------------------------------------------------------------|----------|
| 1.  | 1            | $s_2s_2s_2$ | $\begin{pmatrix} 1 & 0 & 0 \\ 0 & 0 & 1 \\ 0 & 1 & 0 \end{pmatrix}$ | -1       |
| 2.  | $x^2yx^3y$   | $s_2s_1s_2$ | $\begin{pmatrix} 1 & 0 & 0 \\ 0 & 1 & 1 \\ 0 & 1 & 0 \end{pmatrix}$ | -1       |
| 3.  | $y^3$        | $s_4s_4s_4$ | $\begin{pmatrix} 1 & 0 & 0 \\ 0 & 0 & 1 \\ 0 & 1 & 0 \end{pmatrix}$ | -1       |
| 4.  | $y^4$        | $s_1s_1s_2$ | $\begin{pmatrix} 1 & 0 & 0 \\ 1 & 1 & 1 \\ 0 & 1 & 0 \end{pmatrix}$ | -1       |
| 5.  | $xyx^3y$     | $s_4s_4s_2$ | $\begin{pmatrix} 1 & 0 & 0 \\ 0 & 0 & 1 \\ 0 & 1 & 0 \end{pmatrix}$ | -1       |
| 6.  | $(x^3y)^2$   | $s_4s_2s_4$ | $\begin{pmatrix} 1 & 0 & 0 \\ 0 & 0 & 1 \\ 0 & 1 & 0 \end{pmatrix}$ | -1       |
| 7.  | $x(x^2y)^2y$ | $s_4s_3s_2$ | $\begin{pmatrix} 1 & 0 & 0 \\ 0 & 1 & 1 \\ 0 & 1 & 0 \end{pmatrix}$ | -1       |
| 8.  | $x^2y^2x$    | $s_2s_2s_1$ | $\begin{pmatrix} 0 & 0 & 1 \\ 1 & 0 & 1 \\ 0 & 1 & 0 \end{pmatrix}$ | 1        |
| 9.  | $x$          | $s_4s_3s_4$ | $\begin{pmatrix} 1 & 0 & 0 \\ 0 & 1 & 1 \\ 0 & 1 & 0 \end{pmatrix}$ | -1       |
| 10. | $x^3$        | $s_4s_1s_4$ | $\begin{pmatrix} 1 & 0 & 0 \\ 0 & 1 & 1 \\ 0 & 1 & 0 \end{pmatrix}$ | -1       |
| 11. | $y$          | $s_3s_3s_4$ | $\begin{pmatrix} 1 & 0 & 0 \\ 1 & 1 & 1 \\ 0 & 1 & 0 \end{pmatrix}$ | -1       |
| 12. | $(x^2y)^2y$  | $s_2s_2s_4$ | $\begin{pmatrix} 1 & 0 & 0 \\ 0 & 0 & 1 \\ 0 & 1 & 0 \end{pmatrix}$ | -1       |

|     |             |             |                                                                     |    |
|-----|-------------|-------------|---------------------------------------------------------------------|----|
| 13. | $yx^2y^2$   | $s_2s_4s_2$ | $\begin{pmatrix} 1 & 0 & 0 \\ 0 & 0 & 1 \\ 0 & 1 & 0 \end{pmatrix}$ | -1 |
| 14. | $y^2$       | $s_1s_2s_1$ | $\begin{pmatrix} 0 & 0 & 1 \\ 1 & 0 & 1 \\ 1 & 1 & 0 \end{pmatrix}$ | 1  |
| 15. | $x^2y^4$    | $s_2s_3s_1$ | $\begin{pmatrix} 0 & 1 & 1 \\ 1 & 0 & 1 \\ 0 & 1 & 0 \end{pmatrix}$ | 1  |
| 16. | $xy^2x$     | $s_2s_1s_3$ | $\begin{pmatrix} 0 & 1 & 1 \\ 1 & 0 & 1 \\ 0 & 1 & 0 \end{pmatrix}$ | 1  |
| 17. | $x^2$       | $s_2s_4s_4$ | $\begin{pmatrix} 1 & 0 & 0 \\ 0 & 0 & 1 \\ 0 & 1 & 0 \end{pmatrix}$ | -1 |
| 18. | $x^3yx^2$   | $s_2s_4s_3$ | $\begin{pmatrix} 0 & 0 & 1 \\ 1 & 0 & 1 \\ 0 & 1 & 0 \end{pmatrix}$ | 1  |
| 19. | $xy^3$      | $s_2s_1s_4$ | $\begin{pmatrix} 1 & 0 & 0 \\ 0 & 1 & 1 \\ 0 & 1 & 0 \end{pmatrix}$ | -1 |
| 20. | $x^3y^3$    | $s_2s_3s_4$ | $\begin{pmatrix} 1 & 0 & 0 \\ 0 & 1 & 1 \\ 0 & 1 & 0 \end{pmatrix}$ | -1 |
| 21. | $x(x^2y)^2$ | $s_1s_2s_2$ | $\begin{pmatrix} 1 & 0 & 0 \\ 0 & 0 & 1 \\ 1 & 1 & 0 \end{pmatrix}$ | -1 |
| 22. | $y^2x$      | $s_4s_4s_3$ | $\begin{pmatrix} 0 & 0 & 1 \\ 1 & 0 & 1 \\ 0 & 1 & 0 \end{pmatrix}$ | 1  |
| 23. | $xy^4$      | $s_2s_2s_3$ | $\begin{pmatrix} 0 & 0 & 1 \\ 1 & 0 & 1 \\ 0 & 1 & 0 \end{pmatrix}$ | 1  |
| 24. | $yx^3y$     | $s_2s_3s_2$ | $\begin{pmatrix} 1 & 0 & 0 \\ 0 & 1 & 1 \\ 0 & 1 & 0 \end{pmatrix}$ | -1 |
| 25. | $xyx$       | $s_1s_4s_3$ | $\begin{pmatrix} 0 & 0 & 1 \\ 1 & 0 & 1 \\ 1 & 1 & 0 \end{pmatrix}$ | 1  |
| 26. | $x^2y$      | $s_1s_1s_4$ | $\begin{pmatrix} 1 & 0 & 0 \\ 1 & 1 & 1 \\ 0 & 1 & 0 \end{pmatrix}$ | -1 |
| 27. | $x^2yx^2$   | $s_1s_3s_4$ | $\begin{pmatrix} 1 & 0 & 0 \\ 1 & 1 & 1 \\ 0 & 1 & 0 \end{pmatrix}$ | -1 |
| 28. | $x^2y^3$    | $s_4s_2s_2$ | $\begin{pmatrix} 1 & 0 & 0 \\ 0 & 0 & 1 \\ 0 & 1 & 0 \end{pmatrix}$ | -1 |

|     |            |             |                                                                     |    |
|-----|------------|-------------|---------------------------------------------------------------------|----|
| 29. | $yx^2y$    | $s_3s_2s_3$ | $\begin{pmatrix} 0 & 0 & 1 \\ 1 & 0 & 1 \\ 1 & 1 & 0 \end{pmatrix}$ | 1  |
| 30. | $x^2y^2$   | $s_1s_2s_3$ | $\begin{pmatrix} 0 & 0 & 1 \\ 1 & 0 & 1 \\ 1 & 1 & 0 \end{pmatrix}$ | 1  |
| 31. | $x^3y^2x$  | $s_1s_3s_2$ | $\begin{pmatrix} 1 & 0 & 0 \\ 1 & 1 & 1 \\ 0 & 1 & 0 \end{pmatrix}$ | -1 |
| 32. | $x^2yx^3$  | $s_3s_2s_4$ | $\begin{pmatrix} 1 & 0 & 0 \\ 0 & 0 & 1 \\ 1 & 1 & 0 \end{pmatrix}$ | -1 |
| 33. | $xyx^2$    | $s_4s_2s_1$ | $\begin{pmatrix} 0 & 0 & 1 \\ 1 & 0 & 1 \\ 0 & 1 & 0 \end{pmatrix}$ | 1  |
| 34. | $xy$       | $s_2s_4s_1$ | $\begin{pmatrix} 0 & 0 & 1 \\ 1 & 0 & 1 \\ 0 & 1 & 0 \end{pmatrix}$ | 1  |
| 35. | $xyx^2y^2$ | $s_4s_1s_2$ | $\begin{pmatrix} 1 & 0 & 0 \\ 0 & 1 & 1 \\ 0 & 1 & 0 \end{pmatrix}$ | -1 |
| 36. | $x^3y^2$   | $s_3s_2s_2$ | $\begin{pmatrix} 1 & 0 & 0 \\ 0 & 0 & 1 \\ 1 & 1 & 0 \end{pmatrix}$ | -1 |
| 37. | $xyx^2y$   | $s_3s_4s_4$ | $\begin{pmatrix} 1 & 0 & 0 \\ 0 & 0 & 1 \\ 1 & 1 & 0 \end{pmatrix}$ | -1 |
| 38. | $x^3y^4$   | $s_4s_4s_1$ | $\begin{pmatrix} 0 & 0 & 1 \\ 1 & 0 & 1 \\ 0 & 1 & 0 \end{pmatrix}$ | 1  |
| 39. | $x^3yx^3$  | $s_3s_4s_1$ | $\begin{pmatrix} 0 & 0 & 1 \\ 1 & 0 & 1 \\ 1 & 1 & 0 \end{pmatrix}$ | 1  |
| 40. | $x^3yx$    | $s_1s_4s_1$ | $\begin{pmatrix} 0 & 0 & 1 \\ 1 & 0 & 1 \\ 1 & 1 & 0 \end{pmatrix}$ | 1  |
| 41. | $yx^2$     | $s_3s_1s_4$ | $\begin{pmatrix} 1 & 0 & 0 \\ 1 & 1 & 1 \\ 0 & 1 & 0 \end{pmatrix}$ | -1 |
| 42. | $(x^2y)^2$ | $s_3s_2s_1$ | $\begin{pmatrix} 0 & 0 & 1 \\ 1 & 0 & 1 \\ 1 & 1 & 0 \end{pmatrix}$ | 1  |
| 43. | $yx$       | $s_1s_2s_4$ | $\begin{pmatrix} 1 & 0 & 0 \\ 0 & 0 & 1 \\ 1 & 1 & 0 \end{pmatrix}$ | -1 |
| 44. | $yx^3$     | $s_1s_4s_2$ | $\begin{pmatrix} 1 & 0 & 0 \\ 0 & 0 & 1 \\ 1 & 1 & 0 \end{pmatrix}$ | -1 |



|     |         |             |                                                                     |    |
|-----|---------|-------------|---------------------------------------------------------------------|----|
| 45. | $x^3y$  | $s_4s_2s_3$ | $\begin{pmatrix} 0 & 0 & 1 \\ 1 & 0 & 1 \\ 0 & 1 & 0 \end{pmatrix}$ | 1  |
| 46. | $xy^2$  | $s_1s_4s_4$ | $\begin{pmatrix} 1 & 0 & 0 \\ 0 & 0 & 1 \\ 1 & 1 & 0 \end{pmatrix}$ | -1 |
| 47. | $xyx^3$ | $s_3s_4s_3$ | $\begin{pmatrix} 0 & 0 & 1 \\ 1 & 0 & 1 \\ 1 & 1 & 0 \end{pmatrix}$ | 1  |
| 48. | $x^2yx$ | $s_3s_4s_2$ | $\begin{pmatrix} 1 & 0 & 0 \\ 0 & 0 & 1 \\ 1 & 1 & 0 \end{pmatrix}$ | -1 |

## Solution for directed graphs of diameter 4

|                               |                                                                                                           |
|-------------------------------|-----------------------------------------------------------------------------------------------------------|
| Diameter                      | 4                                                                                                         |
| Set size                      | 3                                                                                                         |
| Group $K$                     | $\mathbb{Z}_3 \times A_4$ (order 36; id 11)                                                               |
|                               | $\langle x, y \mid x^3, y^6, (y^{-1}x^{-1})^3, y^{-2}xy^2x^{-1}, (yx^{-1})^3, (xyx^{-1}x^{-1})^2 \rangle$ |
| $\varphi : K \rightarrow S_4$ | $x \mapsto (2\ 3\ 4)$<br>$y \mapsto (1\ 2)(3\ 4)$                                                         |
| Set $S$                       | $\{s_1, s_2, s_3\} =$<br>$\{x, x^2y^3, xy\}$                                                              |
| Set $V$                       | $\{0010, 0110, 1011\}$                                                                                    |

| No. | Element    | Product        | Mapping matrix $M$                                                                               | $\det M$ |
|-----|------------|----------------|--------------------------------------------------------------------------------------------------|----------|
| 1.  | 1          | $s_1s_2s_1s_2$ | $\begin{pmatrix} 0 & 1 & 1 & 0 \\ 1 & 0 & 0 & 1 \\ 0 & 0 & 0 & 1 \\ 0 & 1 & 0 & 0 \end{pmatrix}$ | -1       |
| 2.  | $x$        | $s_3s_3s_3s_1$ | $\begin{pmatrix} 0 & 1 & 1 & 0 \\ 1 & 0 & 1 & 0 \\ 1 & 1 & 0 & 1 \\ 1 & 1 & 1 & 0 \end{pmatrix}$ | -1       |
| 3.  | $y^4$      | $s_1s_3s_2s_2$ | $\begin{pmatrix} 0 & 0 & 1 & 0 \\ 1 & 1 & 0 & 1 \\ 0 & 1 & 1 & 1 \\ 0 & 1 & 0 & 0 \end{pmatrix}$ | -1       |
| 4.  | $y^3$      | $s_2s_2s_1s_1$ | $\begin{pmatrix} 1 & 0 & 0 & 0 \\ 1 & 1 & 0 & 0 \\ 0 & 0 & 0 & 1 \\ 0 & 1 & 1 & 0 \end{pmatrix}$ | -1       |
| 5.  | $x(xy)^2y$ | $s_1s_1s_2s_2$ | $\begin{pmatrix} 0 & 0 & 1 & 0 \\ 0 & 1 & 0 & 1 \\ 0 & 0 & 1 & 1 \\ 1 & 0 & 0 & 0 \end{pmatrix}$ | 1        |
| 6.  | $x^2$      | $s_3s_3s_2s_3$ | $\begin{pmatrix} 0 & 1 & 0 & 1 \\ 1 & 1 & 0 & 0 \\ 1 & 0 & 1 & 1 \\ 1 & 1 & 1 & 1 \end{pmatrix}$ | 1        |
| 7.  | $xy^4$     | $s_2s_2s_3s_2$ | $\begin{pmatrix} 1 & 1 & 1 & 0 \\ 0 & 0 & 1 & 1 \\ 1 & 0 & 0 & 1 \\ 0 & 1 & 1 & 0 \end{pmatrix}$ | 1        |
| 8.  | $xy^3$     | $s_2s_1s_2s_2$ | $\begin{pmatrix} 0 & 0 & 1 & 0 \\ 1 & 1 & 0 & 1 \\ 0 & 0 & 1 & 1 \\ 1 & 0 & 0 & 0 \end{pmatrix}$ | 1        |
| 9.  | $xyx^2$    | $s_3s_1s_3s_3$ | $\begin{pmatrix} 1 & 0 & 1 & 1 \\ 1 & 0 & 1 & 0 \\ 0 & 1 & 1 & 1 \\ 1 & 0 & 0 & 1 \end{pmatrix}$ | 1        |

|     |               |                   |                                                                                                  |    |
|-----|---------------|-------------------|--------------------------------------------------------------------------------------------------|----|
| 10. | $y^2$         | $s_2 s_3 s_2 s_3$ | $\begin{pmatrix} 1 & 1 & 0 & 1 \\ 1 & 1 & 0 & 0 \\ 0 & 0 & 1 & 1 \\ 0 & 1 & 1 & 1 \end{pmatrix}$ | 1  |
| 11. | $y$           | $s_3 s_1 s_2 s_2$ | $\begin{pmatrix} 1 & 0 & 1 & 0 \\ 0 & 1 & 0 & 1 \\ 1 & 0 & 1 & 1 \\ 1 & 0 & 0 & 0 \end{pmatrix}$ | 1  |
| 12. | $x^2 y x$     | $s_1 s_2 s_2 s_3$ | $\begin{pmatrix} 0 & 0 & 0 & 1 \\ 0 & 1 & 0 & 0 \\ 0 & 1 & 1 & 1 \\ 1 & 0 & 1 & 1 \end{pmatrix}$ | -1 |
| 13. | $x y x^2 y^2$ | $s_2 s_1 s_1 s_2$ | $\begin{pmatrix} 0 & 0 & 1 & 0 \\ 0 & 0 & 0 & 1 \\ 1 & 0 & 0 & 1 \\ 1 & 1 & 0 & 0 \end{pmatrix}$ | 1  |
| 14. | $x^2 y^4$     | $s_3 s_1 s_2 s_1$ | $\begin{pmatrix} 0 & 1 & 0 & 0 \\ 1 & 0 & 0 & 0 \\ 1 & 0 & 1 & 1 \\ 1 & 0 & 1 & 0 \end{pmatrix}$ | 1  |
| 15. | $x^2 y^3$     | $s_1 s_1 s_1 s_2$ | $\begin{pmatrix} 0 & 0 & 1 & 0 \\ 0 & 0 & 0 & 1 \\ 1 & 0 & 0 & 1 \\ 0 & 1 & 0 & 0 \end{pmatrix}$ | 1  |
| 16. | $(x y)^2 y$   | $s_1 s_1 s_2 s_1$ | $\begin{pmatrix} 0 & 1 & 0 & 0 \\ 1 & 0 & 0 & 0 \\ 0 & 0 & 1 & 1 \\ 0 & 0 & 1 & 0 \end{pmatrix}$ | 1  |
| 17. | $x y^2$       | $s_3 s_1 s_1 s_3$ | $\begin{pmatrix} 0 & 1 & 0 & 1 \\ 1 & 0 & 0 & 0 \\ 1 & 0 & 1 & 1 \\ 1 & 0 & 0 & 1 \end{pmatrix}$ | -1 |
| 18. | $x y$         | $s_3 s_1 s_1 s_1$ | $\begin{pmatrix} 1 & 0 & 0 & 0 \\ 0 & 1 & 0 & 0 \\ 1 & 0 & 0 & 1 \\ 1 & 0 & 1 & 0 \end{pmatrix}$ | -1 |
| 19. | $y x$         | $s_1 s_1 s_3 s_1$ | $\begin{pmatrix} 1 & 0 & 1 & 0 \\ 0 & 0 & 1 & 0 \\ 0 & 0 & 0 & 1 \\ 0 & 1 & 1 & 0 \end{pmatrix}$ | 1  |
| 20. | $(x^2 y)^2 y$ | $s_2 s_2 s_1 s_2$ | $\begin{pmatrix} 0 & 1 & 1 & 0 \\ 1 & 0 & 0 & 1 \\ 0 & 0 & 0 & 1 \\ 1 & 1 & 0 & 0 \end{pmatrix}$ | -1 |
| 21. | $(x y)^2 x$   | $s_2 s_3 s_3 s_2$ | $\begin{pmatrix} 1 & 1 & 1 & 0 \\ 1 & 1 & 1 & 1 \\ 0 & 1 & 0 & 1 \\ 0 & 0 & 1 & 0 \end{pmatrix}$ | 1  |

|     |            |                |                                                                                                  |    |
|-----|------------|----------------|--------------------------------------------------------------------------------------------------|----|
| 22. | $xyx^2y$   | $s_2s_2s_3s_3$ | $\begin{pmatrix} 0 & 1 & 1 & 1 \\ 0 & 0 & 1 & 0 \\ 1 & 1 & 1 & 1 \\ 1 & 0 & 0 & 1 \end{pmatrix}$ | 1  |
| 23. | $xyx^2$    | $s_2s_2s_3s_1$ | $\begin{pmatrix} 0 & 0 & 1 & 0 \\ 0 & 1 & 1 & 0 \\ 1 & 0 & 0 & 1 \\ 1 & 1 & 1 & 0 \end{pmatrix}$ | 1  |
| 24. | $x^2y^2$   | $s_3s_1s_3s_2$ | $\begin{pmatrix} 0 & 1 & 1 & 0 \\ 1 & 0 & 1 & 1 \\ 1 & 0 & 0 & 1 \\ 1 & 0 & 1 & 0 \end{pmatrix}$ | -1 |
| 25. | $x^2y$     | $s_3s_2s_1s_1$ | $\begin{pmatrix} 1 & 0 & 0 & 0 \\ 0 & 1 & 0 & 0 \\ 1 & 0 & 0 & 1 \\ 1 & 1 & 1 & 0 \end{pmatrix}$ | -1 |
| 26. | $xyx$      | $s_1s_1s_3s_2$ | $\begin{pmatrix} 0 & 1 & 1 & 0 \\ 1 & 0 & 1 & 1 \\ 0 & 0 & 0 & 1 \\ 0 & 0 & 1 & 0 \end{pmatrix}$ | 1  |
| 27. | $yx^2y^2$  | $s_1s_2s_1s_1$ | $\begin{pmatrix} 1 & 0 & 0 & 0 \\ 0 & 1 & 0 & 0 \\ 0 & 0 & 0 & 1 \\ 0 & 1 & 1 & 0 \end{pmatrix}$ | -1 |
| 28. | $x(xy)^2x$ | $s_1s_3s_3s_1$ | $\begin{pmatrix} 0 & 1 & 1 & 0 \\ 0 & 0 & 1 & 0 \\ 0 & 1 & 0 & 1 \\ 1 & 1 & 1 & 0 \end{pmatrix}$ | -1 |
| 29. | $(x^2y)^2$ | $s_1s_3s_1s_3$ | $\begin{pmatrix} 1 & 1 & 0 & 1 \\ 0 & 1 & 0 & 0 \\ 0 & 0 & 1 & 1 \\ 0 & 1 & 0 & 1 \end{pmatrix}$ | 1  |
| 30. | $x^2yx^2$  | $s_1s_3s_1s_1$ | $\begin{pmatrix} 0 & 1 & 0 & 0 \\ 1 & 1 & 0 & 0 \\ 0 & 1 & 0 & 1 \\ 0 & 0 & 1 & 0 \end{pmatrix}$ | 1  |
| 31. | $x(xy)^2$  | $s_3s_3s_2s_2$ | $\begin{pmatrix} 1 & 0 & 1 & 0 \\ 1 & 1 & 0 & 1 \\ 1 & 1 & 1 & 1 \\ 0 & 1 & 0 & 0 \end{pmatrix}$ | -1 |
| 32. | $(yx)^2$   | $s_3s_3s_2s_1$ | $\begin{pmatrix} 1 & 1 & 0 & 0 \\ 0 & 1 & 0 & 0 \\ 1 & 1 & 1 & 1 \\ 1 & 0 & 1 & 0 \end{pmatrix}$ | -1 |
| 33. | $yx^2y$    | $s_1s_3s_2s_3$ | $\begin{pmatrix} 0 & 1 & 0 & 1 \\ 1 & 1 & 0 & 0 \\ 0 & 0 & 1 & 1 \\ 0 & 1 & 1 & 1 \end{pmatrix}$ | 1  |

|     |          |                |                                                                                                  |      |
|-----|----------|----------------|--------------------------------------------------------------------------------------------------|------|
| 34. | $yx^2$   | $s_1s_3s_2s_1$ | $\begin{pmatrix} 1 & 1 & 0 & 0 \\ 0 & 1 & 0 & 0 \\ 0 & 1 & 1 & 1 \\ 0 & 0 & 1 & 0 \end{pmatrix}$ | $-1$ |
| 35. | $xyx$    | $s_1s_1s_3s_3$ | $\begin{pmatrix} 0 & 0 & 1 & 1 \\ 1 & 0 & 1 & 0 \\ 0 & 1 & 1 & 1 \\ 0 & 0 & 0 & 1 \end{pmatrix}$ | $1$  |
| 36. | $(xy)^2$ | $s_3s_2s_3s_1$ | $\begin{pmatrix} 1 & 0 & 1 & 0 \\ 1 & 1 & 1 & 0 \\ 1 & 0 & 0 & 1 \\ 0 & 1 & 1 & 0 \end{pmatrix}$ | $-1$ |

## Solution for directed graphs of diameter 5

|                               |                                                                                                          |
|-------------------------------|----------------------------------------------------------------------------------------------------------|
| Diameter                      | 5                                                                                                        |
| Set size                      | 3                                                                                                        |
| Group $K$                     | $S_5$ (order 120; id 34)<br>$\langle x, y \mid x^5, y^2, (yx)^4, (yx^{-1}yx)^3, (x^2yx^{-2}y)^2 \rangle$ |
| $\varphi : K \rightarrow S_5$ | $x \mapsto (1\ 2\ 3\ 5\ 4)$<br>$y \mapsto (2\ 3)$                                                        |
| Set $S$                       | $\{s_1, s_2, s_3\} =$<br>$\{(yx)^2x^2y, yx(xy)^2, x^2(xy)^2x^2\}$                                        |
| Set $V$                       | $\{11000, 10100, 10000\}$                                                                                |

| No. | Element      | Product           | Mapping matrix $M$                                                                                                                    | $\det M$ |
|-----|--------------|-------------------|---------------------------------------------------------------------------------------------------------------------------------------|----------|
| 1.  | 1            | $s_3s_3s_3s_3s_3$ | $\begin{pmatrix} 0 & 0 & 0 & 0 & 1 \\ 0 & 0 & 0 & 1 & 0 \\ 0 & 0 & 1 & 0 & 0 \\ 0 & 1 & 0 & 0 & 0 \\ 1 & 0 & 0 & 0 & 0 \end{pmatrix}$ | 1        |
| 2.  | $x^3yx^2$    | $s_3s_1s_3s_3s_3$ | $\begin{pmatrix} 0 & 0 & 0 & 0 & 1 \\ 0 & 0 & 0 & 1 & 0 \\ 0 & 0 & 1 & 0 & 0 \\ 1 & 1 & 0 & 0 & 0 \\ 0 & 1 & 0 & 0 & 0 \end{pmatrix}$ | -1       |
| 3.  | $(x^2y)^3$   | $s_3s_3s_1s_3s_3$ | $\begin{pmatrix} 0 & 0 & 0 & 0 & 1 \\ 0 & 0 & 0 & 1 & 0 \\ 0 & 1 & 1 & 0 & 0 \\ 0 & 0 & 1 & 0 & 0 \\ 1 & 0 & 0 & 0 & 0 \end{pmatrix}$ | -1       |
| 4.  | $(yx)^2x^2$  | $s_3s_1s_1s_3s_3$ | $\begin{pmatrix} 0 & 0 & 0 & 0 & 1 \\ 0 & 0 & 0 & 1 & 0 \\ 1 & 1 & 1 & 0 & 0 \\ 0 & 0 & 1 & 0 & 0 \\ 0 & 1 & 0 & 0 & 0 \end{pmatrix}$ | 1        |
| 5.  | $x^2(xy)^2x$ | $s_3s_1s_2s_3s_3$ | $\begin{pmatrix} 0 & 0 & 0 & 0 & 1 \\ 0 & 0 & 0 & 1 & 0 \\ 0 & 1 & 1 & 0 & 0 \\ 1 & 1 & 0 & 0 & 0 \\ 0 & 0 & 1 & 0 & 0 \end{pmatrix}$ | 1        |
| 6.  | $x^4yx$      | $s_3s_3s_2s_3s_3$ | $\begin{pmatrix} 0 & 0 & 0 & 0 & 1 \\ 0 & 0 & 0 & 1 & 0 \\ 1 & 0 & 1 & 0 & 0 \\ 0 & 1 & 0 & 0 & 0 \\ 0 & 0 & 1 & 0 & 0 \end{pmatrix}$ | -1       |
| 7.  | $y$          | $s_3s_3s_3s_1s_3$ | $\begin{pmatrix} 0 & 0 & 0 & 0 & 1 \\ 0 & 0 & 1 & 1 & 0 \\ 0 & 0 & 0 & 1 & 0 \\ 0 & 1 & 0 & 0 & 0 \\ 1 & 0 & 0 & 0 & 0 \end{pmatrix}$ | -1       |

|     |                 |                   |                                                                                                                                       |    |
|-----|-----------------|-------------------|---------------------------------------------------------------------------------------------------------------------------------------|----|
| 8.  | $x(x^2y)^2$     | $s_3s_1s_3s_1s_3$ | $\begin{pmatrix} 0 & 0 & 0 & 0 & 1 \\ 0 & 0 & 1 & 1 & 0 \\ 0 & 0 & 0 & 1 & 0 \\ 1 & 1 & 0 & 0 & 0 \\ 0 & 1 & 0 & 0 & 0 \end{pmatrix}$ | 1  |
| 9.  | $(x^2y)^2x^2$   | $s_3s_3s_1s_1s_3$ | $\begin{pmatrix} 0 & 0 & 0 & 0 & 1 \\ 0 & 1 & 1 & 1 & 0 \\ 0 & 0 & 0 & 1 & 0 \\ 0 & 0 & 1 & 0 & 0 \\ 1 & 0 & 0 & 0 & 0 \end{pmatrix}$ | 1  |
| 10. | $(yx)^2x^2y$    | $s_2s_1s_1s_3s_3$ | $\begin{pmatrix} 0 & 0 & 0 & 0 & 1 \\ 1 & 0 & 0 & 1 & 0 \\ 1 & 1 & 1 & 0 & 0 \\ 0 & 0 & 1 & 0 & 0 \\ 0 & 1 & 0 & 0 & 0 \end{pmatrix}$ | 1  |
| 11. | $x^2yx^4$       | $s_2s_3s_2s_2s_3$ | $\begin{pmatrix} 0 & 0 & 0 & 0 & 1 \\ 0 & 1 & 0 & 1 & 0 \\ 1 & 0 & 1 & 0 & 0 \\ 1 & 0 & 0 & 1 & 0 \\ 0 & 0 & 1 & 0 & 0 \end{pmatrix}$ | 1  |
| 12. | $x^3(xy)^2$     | $s_2s_3s_2s_3s_3$ | $\begin{pmatrix} 0 & 0 & 0 & 0 & 1 \\ 1 & 0 & 0 & 1 & 0 \\ 1 & 0 & 1 & 0 & 0 \\ 0 & 1 & 0 & 0 & 0 \\ 0 & 0 & 1 & 0 & 0 \end{pmatrix}$ | -1 |
| 13. | $(xyx)^2$       | $s_3s_3s_1s_2s_3$ | $\begin{pmatrix} 0 & 0 & 0 & 0 & 1 \\ 0 & 0 & 1 & 1 & 0 \\ 0 & 1 & 1 & 0 & 0 \\ 0 & 0 & 0 & 1 & 0 \\ 1 & 0 & 0 & 0 & 0 \end{pmatrix}$ | 1  |
| 14. | $xyx^3$         | $s_2s_1s_3s_1s_3$ | $\begin{pmatrix} 0 & 0 & 0 & 0 & 1 \\ 0 & 0 & 1 & 1 & 0 \\ 1 & 0 & 0 & 1 & 0 \\ 1 & 1 & 0 & 0 & 0 \\ 0 & 1 & 0 & 0 & 0 \end{pmatrix}$ | 1  |
| 15. | $(xyx)^2y$      | $s_3s_3s_3s_2s_3$ | $\begin{pmatrix} 0 & 0 & 0 & 0 & 1 \\ 0 & 1 & 0 & 1 & 0 \\ 0 & 0 & 1 & 0 & 0 \\ 0 & 0 & 0 & 1 & 0 \\ 1 & 0 & 0 & 0 & 0 \end{pmatrix}$ | -1 |
| 16. | $xyx^3y$        | $s_2s_1s_3s_3s_3$ | $\begin{pmatrix} 0 & 0 & 0 & 0 & 1 \\ 1 & 0 & 0 & 1 & 0 \\ 0 & 0 & 1 & 0 & 0 \\ 1 & 1 & 0 & 0 & 0 \\ 0 & 1 & 0 & 0 & 0 \end{pmatrix}$ | -1 |
| 17. | $x^2(x^2y)^3xy$ | $s_3s_3s_2s_2s_3$ | $\begin{pmatrix} 0 & 0 & 0 & 0 & 1 \\ 0 & 1 & 0 & 1 & 0 \\ 1 & 0 & 1 & 0 & 0 \\ 0 & 0 & 0 & 1 & 0 \\ 0 & 0 & 1 & 0 & 0 \end{pmatrix}$ | 1  |

|     |                |                   |                                                                                                                                       |    |
|-----|----------------|-------------------|---------------------------------------------------------------------------------------------------------------------------------------|----|
| 18. | $x^2(x^2y)^3x$ | $s_2s_1s_2s_3s_3$ | $\begin{pmatrix} 0 & 0 & 0 & 0 & 1 \\ 1 & 0 & 0 & 1 & 0 \\ 0 & 1 & 1 & 0 & 0 \\ 1 & 1 & 0 & 0 & 0 \\ 0 & 0 & 1 & 0 & 0 \end{pmatrix}$ | 1  |
| 19. | $(x^2yx)^2y$   | $s_2s_3s_1s_2s_3$ | $\begin{pmatrix} 0 & 0 & 0 & 0 & 1 \\ 0 & 0 & 1 & 1 & 0 \\ 0 & 1 & 1 & 0 & 0 \\ 1 & 0 & 0 & 1 & 0 \\ 1 & 0 & 0 & 0 & 0 \end{pmatrix}$ | 1  |
| 20. | $(xy)^2x^2$    | $s_2s_3s_3s_1s_3$ | $\begin{pmatrix} 0 & 0 & 0 & 0 & 1 \\ 0 & 0 & 1 & 1 & 0 \\ 1 & 0 & 0 & 1 & 0 \\ 0 & 1 & 0 & 0 & 0 \\ 1 & 0 & 0 & 0 & 0 \end{pmatrix}$ | -1 |
| 21. | $(x^2yx)^2$    | $s_2s_3s_3s_2s_3$ | $\begin{pmatrix} 0 & 0 & 0 & 0 & 1 \\ 0 & 1 & 0 & 1 & 0 \\ 0 & 0 & 1 & 0 & 0 \\ 1 & 0 & 0 & 1 & 0 \\ 1 & 0 & 0 & 0 & 0 \end{pmatrix}$ | -1 |
| 22. | $(xy)^2x^2y$   | $s_2s_3s_3s_3s_3$ | $\begin{pmatrix} 0 & 0 & 0 & 0 & 1 \\ 1 & 0 & 0 & 1 & 0 \\ 0 & 0 & 1 & 0 & 0 \\ 0 & 1 & 0 & 0 & 0 \\ 1 & 0 & 0 & 0 & 0 \end{pmatrix}$ | 1  |
| 23. | $(x^2y)^2xyx$  | $s_2s_3s_1s_1s_3$ | $\begin{pmatrix} 0 & 0 & 0 & 0 & 1 \\ 0 & 1 & 1 & 1 & 0 \\ 1 & 0 & 0 & 1 & 0 \\ 0 & 0 & 1 & 0 & 0 \\ 1 & 0 & 0 & 0 & 0 \end{pmatrix}$ | 1  |
| 24. | $x(xy)^2x^4$   | $s_2s_3s_1s_3s_3$ | $\begin{pmatrix} 0 & 0 & 0 & 0 & 1 \\ 1 & 0 & 0 & 1 & 0 \\ 0 & 1 & 1 & 0 & 0 \\ 0 & 0 & 1 & 0 & 0 \\ 1 & 0 & 0 & 0 & 0 \end{pmatrix}$ | -1 |
| 25. | $xyx^4$        | $s_3s_3s_3s_3s_1$ | $\begin{pmatrix} 0 & 0 & 0 & 1 & 1 \\ 0 & 0 & 0 & 0 & 1 \\ 0 & 0 & 1 & 0 & 0 \\ 0 & 1 & 0 & 0 & 0 \\ 1 & 0 & 0 & 0 & 0 \end{pmatrix}$ | -1 |
| 26. | $(xyx)^2x$     | $s_3s_1s_3s_3s_1$ | $\begin{pmatrix} 0 & 0 & 0 & 1 & 1 \\ 0 & 0 & 0 & 0 & 1 \\ 0 & 0 & 1 & 0 & 0 \\ 1 & 1 & 0 & 0 & 0 \\ 0 & 1 & 0 & 0 & 0 \end{pmatrix}$ | 1  |
| 27. | $x(x^2y)^3xy$  | $s_3s_3s_1s_3s_1$ | $\begin{pmatrix} 0 & 0 & 0 & 1 & 1 \\ 0 & 0 & 0 & 0 & 1 \\ 0 & 1 & 1 & 0 & 0 \\ 0 & 0 & 1 & 0 & 0 \\ 1 & 0 & 0 & 0 & 0 \end{pmatrix}$ | 1  |



|     |                 |                   |                                                                                                                                       |    |
|-----|-----------------|-------------------|---------------------------------------------------------------------------------------------------------------------------------------|----|
| 28. | $yx(xy)^2$      | $s_3s_1s_1s_3s_1$ | $\begin{pmatrix} 0 & 0 & 0 & 1 & 1 \\ 0 & 0 & 0 & 0 & 1 \\ 1 & 1 & 1 & 0 & 0 \\ 0 & 0 & 1 & 0 & 0 \\ 0 & 1 & 0 & 0 & 0 \end{pmatrix}$ | -1 |
| 29. | $(xyx)^2yx$     | $s_3s_1s_2s_3s_1$ | $\begin{pmatrix} 0 & 0 & 0 & 1 & 1 \\ 0 & 0 & 0 & 0 & 1 \\ 0 & 1 & 1 & 0 & 0 \\ 1 & 1 & 0 & 0 & 0 \\ 0 & 0 & 1 & 0 & 0 \end{pmatrix}$ | -1 |
| 30. | $xyx^3yx$       | $s_3s_3s_2s_3s_1$ | $\begin{pmatrix} 0 & 0 & 0 & 1 & 1 \\ 0 & 0 & 0 & 0 & 1 \\ 1 & 0 & 1 & 0 & 0 \\ 0 & 1 & 0 & 0 & 0 \\ 0 & 0 & 1 & 0 & 0 \end{pmatrix}$ | 1  |
| 31. | $(yx)^2x^3$     | $s_3s_3s_3s_1s_1$ | $\begin{pmatrix} 0 & 0 & 1 & 1 & 1 \\ 0 & 0 & 0 & 0 & 1 \\ 0 & 0 & 0 & 1 & 0 \\ 0 & 1 & 0 & 0 & 0 \\ 1 & 0 & 0 & 0 & 0 \end{pmatrix}$ | 1  |
| 32. | $(x^2y)^3x$     | $s_3s_1s_3s_1s_1$ | $\begin{pmatrix} 0 & 0 & 1 & 1 & 1 \\ 0 & 0 & 0 & 0 & 1 \\ 0 & 0 & 0 & 1 & 0 \\ 1 & 1 & 0 & 0 & 0 \\ 0 & 1 & 0 & 0 & 0 \end{pmatrix}$ | -1 |
| 33. | $x^4yx^2$       | $s_3s_2s_1s_1s_3$ | $\begin{pmatrix} 0 & 1 & 0 & 0 & 1 \\ 0 & 1 & 1 & 1 & 0 \\ 0 & 0 & 0 & 1 & 0 \\ 0 & 0 & 1 & 0 & 0 \\ 1 & 0 & 0 & 0 & 0 \end{pmatrix}$ | 1  |
| 34. | $x^2(xy)^2x^2$  | $s_1s_1s_1s_1s_3$ | $\begin{pmatrix} 1 & 0 & 0 & 0 & 1 \\ 1 & 1 & 1 & 1 & 0 \\ 0 & 0 & 0 & 1 & 0 \\ 0 & 0 & 1 & 0 & 0 \\ 0 & 1 & 0 & 0 & 0 \end{pmatrix}$ | -1 |
| 35. | $x$             | $s_1s_2s_2s_1s_3$ | $\begin{pmatrix} 0 & 1 & 0 & 0 & 1 \\ 1 & 0 & 1 & 1 & 0 \\ 0 & 0 & 0 & 1 & 0 \\ 1 & 1 & 0 & 0 & 0 \\ 0 & 0 & 1 & 0 & 0 \end{pmatrix}$ | 1  |
| 36. | $x^3yx^3$       | $s_1s_3s_2s_1s_3$ | $\begin{pmatrix} 1 & 0 & 0 & 0 & 1 \\ 1 & 0 & 1 & 1 & 0 \\ 0 & 0 & 0 & 1 & 0 \\ 0 & 1 & 0 & 0 & 0 \\ 0 & 0 & 1 & 0 & 0 \end{pmatrix}$ | 1  |
| 37. | $x^3(xy)^2x^2y$ | $s_3s_2s_3s_2s_2$ | $\begin{pmatrix} 0 & 0 & 1 & 0 & 1 \\ 0 & 1 & 0 & 1 & 0 \\ 0 & 1 & 0 & 0 & 1 \\ 0 & 0 & 0 & 1 & 0 \\ 1 & 0 & 0 & 0 & 0 \end{pmatrix}$ | 1  |

|     |                   |                       |                                                                                                                                       |    |
|-----|-------------------|-----------------------|---------------------------------------------------------------------------------------------------------------------------------------|----|
| 38. | $x(xy)^2$         | $s_1 s_1 s_3 s_2 s_2$ | $\begin{pmatrix} 0 & 0 & 1 & 0 & 1 \\ 1 & 1 & 0 & 1 & 0 \\ 1 & 0 & 0 & 0 & 1 \\ 0 & 0 & 0 & 1 & 0 \\ 0 & 1 & 0 & 0 & 0 \end{pmatrix}$ | -1 |
| 39. | $(xy)^2 x^3$      | $s_3 s_2 s_3 s_2 s_3$ | $\begin{pmatrix} 0 & 1 & 0 & 0 & 1 \\ 0 & 1 & 0 & 1 & 0 \\ 0 & 0 & 1 & 0 & 0 \\ 0 & 0 & 0 & 1 & 0 \\ 1 & 0 & 0 & 0 & 0 \end{pmatrix}$ | -1 |
| 40. | $x(x^3 y)^2 xy$   | $s_1 s_1 s_3 s_2 s_3$ | $\begin{pmatrix} 1 & 0 & 0 & 0 & 1 \\ 1 & 1 & 0 & 1 & 0 \\ 0 & 0 & 1 & 0 & 0 \\ 0 & 0 & 0 & 1 & 0 \\ 0 & 1 & 0 & 0 & 0 \end{pmatrix}$ | 1  |
| 41. | $x(x^2 y)^3$      | $s_3 s_2 s_2 s_2 s_3$ | $\begin{pmatrix} 0 & 1 & 0 & 0 & 1 \\ 0 & 1 & 0 & 1 & 0 \\ 1 & 0 & 1 & 0 & 0 \\ 0 & 0 & 0 & 1 & 0 \\ 0 & 0 & 1 & 0 & 0 \end{pmatrix}$ | 1  |
| 42. | $yx^2 y$          | $s_1 s_1 s_2 s_2 s_3$ | $\begin{pmatrix} 1 & 0 & 0 & 0 & 1 \\ 1 & 1 & 0 & 1 & 0 \\ 0 & 1 & 1 & 0 & 0 \\ 0 & 0 & 0 & 1 & 0 \\ 0 & 0 & 1 & 0 & 0 \end{pmatrix}$ | -1 |
| 43. | $x(x^3 y)^2$      | $s_2 s_2 s_3 s_2 s_2$ | $\begin{pmatrix} 0 & 0 & 1 & 0 & 1 \\ 0 & 1 & 0 & 1 & 0 \\ 0 & 1 & 0 & 0 & 1 \\ 1 & 0 & 0 & 1 & 0 \\ 1 & 0 & 0 & 0 & 0 \end{pmatrix}$ | 1  |
| 44. | $x^2(xy)^2 x^3 y$ | $s_2 s_3 s_3 s_1 s_1$ | $\begin{pmatrix} 0 & 0 & 1 & 1 & 1 \\ 0 & 0 & 0 & 0 & 1 \\ 1 & 0 & 0 & 1 & 0 \\ 0 & 1 & 0 & 0 & 0 \\ 1 & 0 & 0 & 0 & 0 \end{pmatrix}$ | 1  |
| 45. | $yx$              | $s_2 s_2 s_3 s_2 s_3$ | $\begin{pmatrix} 0 & 1 & 0 & 0 & 1 \\ 0 & 1 & 0 & 1 & 0 \\ 0 & 0 & 1 & 0 & 0 \\ 1 & 0 & 0 & 1 & 0 \\ 1 & 0 & 0 & 0 & 0 \end{pmatrix}$ | -1 |
| 46. | $x(x^2 y)^2 x$    | $s_2 s_3 s_3 s_3 s_1$ | $\begin{pmatrix} 1 & 0 & 0 & 1 & 1 \\ 0 & 0 & 0 & 0 & 1 \\ 0 & 0 & 1 & 0 & 0 \\ 0 & 1 & 0 & 0 & 0 \\ 1 & 0 & 0 & 0 & 0 \end{pmatrix}$ | -1 |
| 47. | $x^3(xy)^2 x$     | $s_2 s_2 s_1 s_1 s_3$ | $\begin{pmatrix} 0 & 1 & 0 & 0 & 1 \\ 0 & 1 & 1 & 1 & 0 \\ 1 & 0 & 0 & 1 & 0 \\ 0 & 0 & 1 & 0 & 0 \\ 1 & 0 & 0 & 0 & 0 \end{pmatrix}$ | 1  |

|     |               |                   |                                                                                                                                       |    |
|-----|---------------|-------------------|---------------------------------------------------------------------------------------------------------------------------------------|----|
| 48. | $x^2y$        | $s_2s_3s_1s_3s_1$ | $\begin{pmatrix} 1 & 0 & 0 & 1 & 1 \\ 0 & 0 & 0 & 0 & 1 \\ 0 & 1 & 1 & 0 & 0 \\ 0 & 0 & 1 & 0 & 0 \\ 1 & 0 & 0 & 0 & 0 \end{pmatrix}$ | 1  |
| 49. | $x(xy)^2x$    | $s_3s_3s_3s_1s_2$ | $\begin{pmatrix} 0 & 0 & 0 & 1 & 1 \\ 0 & 0 & 1 & 1 & 0 \\ 0 & 0 & 0 & 0 & 1 \\ 0 & 1 & 0 & 0 & 0 \\ 1 & 0 & 0 & 0 & 0 \end{pmatrix}$ | 1  |
| 50. | $(xyx)^2xy$   | $s_3s_1s_3s_1s_2$ | $\begin{pmatrix} 0 & 0 & 0 & 1 & 1 \\ 0 & 0 & 1 & 1 & 0 \\ 0 & 0 & 0 & 0 & 1 \\ 1 & 1 & 0 & 0 & 0 \\ 0 & 1 & 0 & 0 & 0 \end{pmatrix}$ | -1 |
| 51. | $x(x^2y)^3x$  | $s_3s_2s_1s_3s_1$ | $\begin{pmatrix} 0 & 0 & 0 & 1 & 1 \\ 0 & 1 & 0 & 0 & 1 \\ 0 & 1 & 1 & 0 & 0 \\ 0 & 0 & 1 & 0 & 0 \\ 1 & 0 & 0 & 0 & 0 \end{pmatrix}$ | 1  |
| 52. | $yx^2yx$      | $s_1s_1s_1s_3s_1$ | $\begin{pmatrix} 0 & 0 & 0 & 1 & 1 \\ 1 & 0 & 0 & 0 & 1 \\ 1 & 1 & 1 & 0 & 0 \\ 0 & 0 & 1 & 0 & 0 \\ 0 & 1 & 0 & 0 & 0 \end{pmatrix}$ | -1 |
| 53. | $(xy)^2x^4$   | $s_1s_2s_2s_3s_1$ | $\begin{pmatrix} 0 & 0 & 0 & 1 & 1 \\ 0 & 1 & 0 & 0 & 1 \\ 1 & 0 & 1 & 0 & 0 \\ 1 & 1 & 0 & 0 & 0 \\ 0 & 0 & 1 & 0 & 0 \end{pmatrix}$ | 1  |
| 54. | $xyx^2(xy)^2$ | $s_1s_3s_2s_3s_1$ | $\begin{pmatrix} 0 & 0 & 0 & 1 & 1 \\ 1 & 0 & 0 & 0 & 1 \\ 1 & 0 & 1 & 0 & 0 \\ 0 & 1 & 0 & 0 & 0 \\ 0 & 0 & 1 & 0 & 0 \end{pmatrix}$ | 1  |
| 55. | $yx(xy)^2x$   | $s_3s_3s_3s_3s_2$ | $\begin{pmatrix} 0 & 0 & 1 & 0 & 1 \\ 0 & 0 & 0 & 1 & 0 \\ 0 & 0 & 0 & 0 & 1 \\ 0 & 1 & 0 & 0 & 0 \\ 1 & 0 & 0 & 0 & 0 \end{pmatrix}$ | -1 |
| 56. | $(x^2y)^3xy$  | $s_3s_1s_3s_3s_2$ | $\begin{pmatrix} 0 & 0 & 1 & 0 & 1 \\ 0 & 0 & 0 & 1 & 0 \\ 0 & 0 & 0 & 0 & 1 \\ 1 & 1 & 0 & 0 & 0 \\ 0 & 1 & 0 & 0 & 0 \end{pmatrix}$ | 1  |
| 57. | $x^2(x^2y)^2$ | $s_3s_2s_1s_3s_3$ | $\begin{pmatrix} 0 & 1 & 0 & 0 & 1 \\ 0 & 0 & 0 & 1 & 0 \\ 0 & 1 & 1 & 0 & 0 \\ 0 & 0 & 1 & 0 & 0 \\ 1 & 0 & 0 & 0 & 0 \end{pmatrix}$ | -1 |

|     |                 |                   |                                                                                                                                       |    |
|-----|-----------------|-------------------|---------------------------------------------------------------------------------------------------------------------------------------|----|
| 58. | $x^2(xy)^2x^2y$ | $s_1s_1s_1s_3s_3$ | $\begin{pmatrix} 1 & 0 & 0 & 0 & 1 \\ 0 & 0 & 0 & 1 & 0 \\ 1 & 1 & 1 & 0 & 0 \\ 0 & 0 & 1 & 0 & 0 \\ 0 & 1 & 0 & 0 & 0 \end{pmatrix}$ | 1  |
| 59. | $xy$            | $s_1s_2s_2s_3s_3$ | $\begin{pmatrix} 0 & 1 & 0 & 0 & 1 \\ 0 & 0 & 0 & 1 & 0 \\ 1 & 0 & 1 & 0 & 0 \\ 1 & 1 & 0 & 0 & 0 \\ 0 & 0 & 1 & 0 & 0 \end{pmatrix}$ | -1 |
| 60. | $(x^3y)^2$      | $s_1s_3s_2s_3s_3$ | $\begin{pmatrix} 1 & 0 & 0 & 0 & 1 \\ 0 & 0 & 0 & 1 & 0 \\ 1 & 0 & 1 & 0 & 0 \\ 0 & 1 & 0 & 0 & 0 \\ 0 & 0 & 1 & 0 & 0 \end{pmatrix}$ | -1 |
| 61. | $x^3(xy)^2x^2$  | $s_3s_3s_3s_2s_2$ | $\begin{pmatrix} 0 & 0 & 1 & 0 & 1 \\ 0 & 1 & 0 & 1 & 0 \\ 0 & 0 & 0 & 0 & 1 \\ 0 & 0 & 0 & 1 & 0 \\ 1 & 0 & 0 & 0 & 0 \end{pmatrix}$ | 1  |
| 62. | $x^2yx$         | $s_2s_1s_3s_3s_2$ | $\begin{pmatrix} 0 & 0 & 1 & 0 & 1 \\ 1 & 0 & 0 & 1 & 0 \\ 0 & 0 & 0 & 0 & 1 \\ 1 & 1 & 0 & 0 & 0 \\ 0 & 1 & 0 & 0 & 0 \end{pmatrix}$ | 1  |
| 63. | $(xy)^2x^3y$    | $s_3s_2s_1s_2s_3$ | $\begin{pmatrix} 0 & 1 & 0 & 0 & 1 \\ 0 & 0 & 1 & 1 & 0 \\ 0 & 1 & 1 & 0 & 0 \\ 0 & 0 & 0 & 1 & 0 \\ 1 & 0 & 0 & 0 & 0 \end{pmatrix}$ | 1  |
| 64. | $x(x^3y)^2x$    | $s_1s_1s_1s_2s_3$ | $\begin{pmatrix} 1 & 0 & 0 & 0 & 1 \\ 0 & 0 & 1 & 1 & 0 \\ 1 & 1 & 1 & 0 & 0 \\ 0 & 0 & 0 & 1 & 0 \\ 0 & 1 & 0 & 0 & 0 \end{pmatrix}$ | -1 |
| 65. | $x(x^2y)^2x^2$  | $s_1s_2s_2s_2s_3$ | $\begin{pmatrix} 0 & 1 & 0 & 0 & 1 \\ 1 & 1 & 0 & 1 & 0 \\ 1 & 0 & 1 & 0 & 0 \\ 0 & 0 & 0 & 1 & 0 \\ 0 & 0 & 1 & 0 & 0 \end{pmatrix}$ | 1  |
| 66. | $yx^2$          | $s_1s_3s_2s_2s_3$ | $\begin{pmatrix} 1 & 0 & 0 & 0 & 1 \\ 0 & 1 & 0 & 1 & 0 \\ 1 & 0 & 1 & 0 & 0 \\ 0 & 0 & 0 & 1 & 0 \\ 0 & 0 & 1 & 0 & 0 \end{pmatrix}$ | 1  |
| 67. | $x^4yx^3$       | $s_2s_3s_3s_2s_2$ | $\begin{pmatrix} 0 & 0 & 1 & 0 & 1 \\ 0 & 1 & 0 & 1 & 0 \\ 0 & 0 & 0 & 0 & 1 \\ 1 & 0 & 0 & 1 & 0 \\ 1 & 0 & 0 & 0 & 0 \end{pmatrix}$ | 1  |

|     |                |                   |                                                                                                                                       |    |
|-----|----------------|-------------------|---------------------------------------------------------------------------------------------------------------------------------------|----|
| 68. | $x^2(xy)^2x^3$ | $s_2s_3s_3s_3s_2$ | $\begin{pmatrix} 0 & 0 & 1 & 0 & 1 \\ 1 & 0 & 0 & 1 & 0 \\ 0 & 0 & 0 & 0 & 1 \\ 0 & 1 & 0 & 0 & 0 \\ 1 & 0 & 0 & 0 & 0 \end{pmatrix}$ | -1 |
| 69. | $yxy$          | $s_2s_2s_1s_2s_3$ | $\begin{pmatrix} 0 & 1 & 0 & 0 & 1 \\ 0 & 0 & 1 & 1 & 0 \\ 0 & 1 & 1 & 0 & 0 \\ 1 & 0 & 0 & 1 & 0 \\ 1 & 0 & 0 & 0 & 0 \end{pmatrix}$ | 1  |
| 70. | $x(x^2y)^2xy$  | $s_2s_3s_3s_1s_2$ | $\begin{pmatrix} 1 & 0 & 0 & 1 & 1 \\ 0 & 0 & 1 & 1 & 0 \\ 0 & 0 & 0 & 0 & 1 \\ 0 & 1 & 0 & 0 & 0 \\ 1 & 0 & 0 & 0 & 0 \end{pmatrix}$ | 1  |
| 71. | $x^3yx^4$      | $s_2s_2s_1s_3s_3$ | $\begin{pmatrix} 0 & 1 & 0 & 0 & 1 \\ 1 & 0 & 0 & 1 & 0 \\ 0 & 1 & 1 & 0 & 0 \\ 0 & 0 & 1 & 0 & 0 \\ 1 & 0 & 0 & 0 & 0 \end{pmatrix}$ | -1 |
| 72. | $x^2$          | $s_2s_2s_1s_3s_1$ | $\begin{pmatrix} 1 & 0 & 0 & 1 & 1 \\ 0 & 1 & 0 & 0 & 1 \\ 0 & 1 & 1 & 0 & 0 \\ 0 & 0 & 1 & 0 & 0 \\ 1 & 0 & 0 & 0 & 0 \end{pmatrix}$ | 1  |
| 73. | $x^3yx$        | $s_3s_2s_3s_1s_2$ | $\begin{pmatrix} 0 & 0 & 0 & 1 & 1 \\ 0 & 0 & 1 & 1 & 0 \\ 0 & 1 & 0 & 0 & 1 \\ 0 & 1 & 0 & 0 & 0 \\ 1 & 0 & 0 & 0 & 0 \end{pmatrix}$ | 1  |
| 74. | $x^4$          | $s_1s_1s_3s_1s_2$ | $\begin{pmatrix} 0 & 0 & 0 & 1 & 1 \\ 0 & 0 & 1 & 1 & 0 \\ 1 & 0 & 0 & 0 & 1 \\ 1 & 1 & 0 & 0 & 0 \\ 0 & 1 & 0 & 0 & 0 \end{pmatrix}$ | -1 |
| 75. | $x^2(xy)^2$    | $s_3s_2s_3s_3s_1$ | $\begin{pmatrix} 0 & 0 & 0 & 1 & 1 \\ 0 & 1 & 0 & 0 & 1 \\ 0 & 0 & 1 & 0 & 0 \\ 0 & 1 & 0 & 0 & 0 \\ 1 & 0 & 0 & 0 & 0 \end{pmatrix}$ | -1 |
| 76. | $x^4y$         | $s_1s_1s_3s_3s_1$ | $\begin{pmatrix} 0 & 0 & 0 & 1 & 1 \\ 1 & 0 & 0 & 0 & 1 \\ 0 & 0 & 1 & 0 & 0 \\ 1 & 1 & 0 & 0 & 0 \\ 0 & 1 & 0 & 0 & 0 \end{pmatrix}$ | 1  |
| 77. | $(yx)^2xy$     | $s_3s_2s_2s_3s_1$ | $\begin{pmatrix} 0 & 0 & 0 & 1 & 1 \\ 0 & 1 & 0 & 0 & 1 \\ 1 & 0 & 1 & 0 & 0 \\ 0 & 1 & 0 & 0 & 0 \\ 0 & 0 & 1 & 0 & 0 \end{pmatrix}$ | 1  |

|     |                |                   |                                                                                                                                       |    |
|-----|----------------|-------------------|---------------------------------------------------------------------------------------------------------------------------------------|----|
| 78. | $(yx)^2x$      | $s_1s_1s_2s_3s_1$ | $\begin{pmatrix} 0 & 0 & 0 & 1 & 1 \\ 1 & 0 & 0 & 0 & 1 \\ 0 & 1 & 1 & 0 & 0 \\ 1 & 1 & 0 & 0 & 0 \\ 0 & 0 & 1 & 0 & 0 \end{pmatrix}$ | -1 |
| 79. | $yx^3yx$       | $s_3s_2s_3s_3s_2$ | $\begin{pmatrix} 0 & 0 & 1 & 0 & 1 \\ 0 & 0 & 0 & 1 & 0 \\ 0 & 1 & 0 & 0 & 1 \\ 0 & 1 & 0 & 0 & 0 \\ 1 & 0 & 0 & 0 & 0 \end{pmatrix}$ | -1 |
| 80. | $yx^4$         | $s_1s_1s_3s_3s_2$ | $\begin{pmatrix} 0 & 0 & 1 & 0 & 1 \\ 0 & 0 & 0 & 1 & 0 \\ 1 & 0 & 0 & 0 & 1 \\ 1 & 1 & 0 & 0 & 0 \\ 0 & 1 & 0 & 0 & 0 \end{pmatrix}$ | 1  |
| 81. | $x^2yx^3$      | $s_3s_2s_3s_3s_3$ | $\begin{pmatrix} 0 & 1 & 0 & 0 & 1 \\ 0 & 0 & 0 & 1 & 0 \\ 0 & 0 & 1 & 0 & 0 \\ 0 & 1 & 0 & 0 & 0 \\ 1 & 0 & 0 & 0 & 0 \end{pmatrix}$ | 1  |
| 82. | $x^3(xy)^2x^4$ | $s_1s_1s_3s_3s_3$ | $\begin{pmatrix} 1 & 0 & 0 & 0 & 1 \\ 0 & 0 & 0 & 1 & 0 \\ 0 & 0 & 1 & 0 & 0 \\ 1 & 1 & 0 & 0 & 0 \\ 0 & 1 & 0 & 0 & 0 \end{pmatrix}$ | -1 |
| 83. | $(x^2y)^2x$    | $s_3s_2s_2s_3s_3$ | $\begin{pmatrix} 0 & 1 & 0 & 0 & 1 \\ 0 & 0 & 0 & 1 & 0 \\ 1 & 0 & 1 & 0 & 0 \\ 0 & 1 & 0 & 0 & 0 \\ 0 & 0 & 1 & 0 & 0 \end{pmatrix}$ | -1 |
| 84. | $x(xy)^2x^3y$  | $s_1s_1s_2s_3s_3$ | $\begin{pmatrix} 1 & 0 & 0 & 0 & 1 \\ 0 & 0 & 0 & 1 & 0 \\ 0 & 1 & 1 & 0 & 0 \\ 1 & 1 & 0 & 0 & 0 \\ 0 & 0 & 1 & 0 & 0 \end{pmatrix}$ | 1  |
| 85. | $yx^2(xy)^2$   | $s_3s_2s_3s_1s_1$ | $\begin{pmatrix} 0 & 0 & 1 & 1 & 1 \\ 0 & 1 & 0 & 0 & 1 \\ 0 & 0 & 0 & 1 & 0 \\ 0 & 1 & 0 & 0 & 0 \\ 1 & 0 & 0 & 0 & 0 \end{pmatrix}$ | 1  |
| 86. | $(xy)^2x$      | $s_1s_1s_3s_1s_1$ | $\begin{pmatrix} 0 & 0 & 1 & 1 & 1 \\ 1 & 0 & 0 & 0 & 1 \\ 0 & 0 & 0 & 1 & 0 \\ 1 & 1 & 0 & 0 & 0 \\ 0 & 1 & 0 & 0 & 0 \end{pmatrix}$ | -1 |
| 87. | $x^2yx^3y$     | $s_3s_2s_3s_1s_3$ | $\begin{pmatrix} 0 & 1 & 0 & 0 & 1 \\ 0 & 0 & 1 & 1 & 0 \\ 0 & 0 & 0 & 1 & 0 \\ 0 & 1 & 0 & 0 & 0 \\ 1 & 0 & 0 & 0 & 0 \end{pmatrix}$ | -1 |

|     |                  |                   |                                                                                                                                       |    |
|-----|------------------|-------------------|---------------------------------------------------------------------------------------------------------------------------------------|----|
| 88. | $x^2(x^2y)^2xyx$ | $s_1s_1s_3s_1s_3$ | $\begin{pmatrix} 1 & 0 & 0 & 0 & 1 \\ 0 & 0 & 1 & 1 & 0 \\ 0 & 0 & 0 & 1 & 0 \\ 1 & 1 & 0 & 0 & 0 \\ 0 & 1 & 0 & 0 & 0 \end{pmatrix}$ | 1  |
| 89. | $(x^2y)^2xy$     | $s_2s_2s_2s_3s_3$ | $\begin{pmatrix} 0 & 1 & 0 & 0 & 1 \\ 1 & 0 & 0 & 1 & 0 \\ 1 & 0 & 1 & 0 & 0 \\ 0 & 1 & 0 & 0 & 0 \\ 0 & 0 & 1 & 0 & 0 \end{pmatrix}$ | -1 |
| 90. | $x(xy)^2x^3$     | $s_1s_1s_2s_1s_3$ | $\begin{pmatrix} 1 & 0 & 0 & 0 & 1 \\ 0 & 1 & 1 & 1 & 0 \\ 0 & 0 & 0 & 1 & 0 \\ 1 & 1 & 0 & 0 & 0 \\ 0 & 0 & 1 & 0 & 0 \end{pmatrix}$ | -1 |
| 91. | $xyx^2y$         | $s_2s_2s_3s_1s_1$ | $\begin{pmatrix} 0 & 0 & 1 & 1 & 1 \\ 0 & 1 & 0 & 0 & 1 \\ 1 & 0 & 0 & 1 & 0 \\ 0 & 1 & 0 & 0 & 0 \\ 1 & 0 & 0 & 0 & 0 \end{pmatrix}$ | 1  |
| 92. | $xyx^2$          | $s_2s_2s_3s_3s_2$ | $\begin{pmatrix} 0 & 0 & 1 & 0 & 1 \\ 1 & 0 & 0 & 1 & 0 \\ 0 & 1 & 0 & 0 & 1 \\ 0 & 1 & 0 & 0 & 0 \\ 1 & 0 & 0 & 0 & 0 \end{pmatrix}$ | -1 |
| 93. | $(yx^2)^2yx$     | $s_2s_2s_3s_1s_3$ | $\begin{pmatrix} 0 & 1 & 0 & 0 & 1 \\ 0 & 0 & 1 & 1 & 0 \\ 1 & 0 & 0 & 1 & 0 \\ 0 & 1 & 0 & 0 & 0 \\ 1 & 0 & 0 & 0 & 0 \end{pmatrix}$ | -1 |
| 94. | $x^2(x^2y)^2x^2$ | $s_2s_2s_3s_1s_2$ | $\begin{pmatrix} 1 & 0 & 0 & 1 & 1 \\ 0 & 0 & 1 & 1 & 0 \\ 0 & 1 & 0 & 0 & 1 \\ 0 & 1 & 0 & 0 & 0 \\ 1 & 0 & 0 & 0 & 0 \end{pmatrix}$ | 1  |
| 95. | $(yx^2)^2yxy$    | $s_2s_2s_3s_3s_3$ | $\begin{pmatrix} 0 & 1 & 0 & 0 & 1 \\ 1 & 0 & 0 & 1 & 0 \\ 0 & 0 & 1 & 0 & 0 \\ 0 & 1 & 0 & 0 & 0 \\ 1 & 0 & 0 & 0 & 0 \end{pmatrix}$ | 1  |
| 96. | $x^2(x^2y)^3$    | $s_2s_2s_3s_3s_1$ | $\begin{pmatrix} 1 & 0 & 0 & 1 & 1 \\ 0 & 1 & 0 & 0 & 1 \\ 0 & 0 & 1 & 0 & 0 \\ 0 & 1 & 0 & 0 & 0 \\ 1 & 0 & 0 & 0 & 0 \end{pmatrix}$ | -1 |
| 97. | $x^3(xy)^2x^3$   | $s_1s_2s_3s_1s_2$ | $\begin{pmatrix} 0 & 0 & 0 & 1 & 1 \\ 0 & 0 & 1 & 1 & 0 \\ 0 & 1 & 0 & 0 & 1 \\ 1 & 1 & 0 & 0 & 0 \\ 1 & 0 & 0 & 0 & 0 \end{pmatrix}$ | 1  |

|      |                 |                   |                                                                                                                                       |    |
|------|-----------------|-------------------|---------------------------------------------------------------------------------------------------------------------------------------|----|
| 98.  | $x^2yx^2$       | $s_1s_3s_3s_1s_2$ | $\begin{pmatrix} 0 & 0 & 0 & 1 & 1 \\ 0 & 0 & 1 & 1 & 0 \\ 1 & 0 & 0 & 0 & 1 \\ 0 & 1 & 0 & 0 & 0 \\ 1 & 0 & 0 & 0 & 0 \end{pmatrix}$ | 1  |
| 99.  | $x^3(xy)^2x^3y$ | $s_1s_2s_3s_3s_1$ | $\begin{pmatrix} 0 & 0 & 0 & 1 & 1 \\ 0 & 1 & 0 & 0 & 1 \\ 0 & 0 & 1 & 0 & 0 \\ 1 & 1 & 0 & 0 & 0 \\ 1 & 0 & 0 & 0 & 0 \end{pmatrix}$ | -1 |
| 100. | $(x^2y)^2$      | $s_1s_3s_3s_3s_1$ | $\begin{pmatrix} 0 & 0 & 0 & 1 & 1 \\ 1 & 0 & 0 & 0 & 1 \\ 0 & 0 & 1 & 0 & 0 \\ 0 & 1 & 0 & 0 & 0 \\ 1 & 0 & 0 & 0 & 0 \end{pmatrix}$ | -1 |
| 101. | $yx^3y$         | $s_1s_2s_1s_3s_1$ | $\begin{pmatrix} 0 & 0 & 0 & 1 & 1 \\ 0 & 1 & 0 & 0 & 1 \\ 1 & 1 & 1 & 0 & 0 \\ 0 & 0 & 1 & 0 & 0 \\ 1 & 0 & 0 & 0 & 0 \end{pmatrix}$ | 1  |
| 102. | $yx^3$          | $s_1s_3s_1s_3s_1$ | $\begin{pmatrix} 0 & 0 & 0 & 1 & 1 \\ 1 & 0 & 0 & 0 & 1 \\ 0 & 1 & 1 & 0 & 0 \\ 0 & 0 & 1 & 0 & 0 \\ 1 & 0 & 0 & 0 & 0 \end{pmatrix}$ | 1  |
| 103. | $x^2(x^2y)^2xy$ | $s_1s_2s_3s_3s_2$ | $\begin{pmatrix} 0 & 0 & 1 & 0 & 1 \\ 0 & 0 & 0 & 1 & 0 \\ 0 & 1 & 0 & 0 & 1 \\ 1 & 1 & 0 & 0 & 0 \\ 1 & 0 & 0 & 0 & 0 \end{pmatrix}$ | -1 |
| 104. | $(yx^2)^2$      | $s_1s_3s_3s_3s_2$ | $\begin{pmatrix} 0 & 0 & 1 & 0 & 1 \\ 0 & 0 & 0 & 1 & 0 \\ 1 & 0 & 0 & 0 & 1 \\ 0 & 1 & 0 & 0 & 0 \\ 1 & 0 & 0 & 0 & 0 \end{pmatrix}$ | -1 |
| 105. | $x(xy)^2x^2$    | $s_1s_2s_3s_3s_3$ | $\begin{pmatrix} 0 & 1 & 0 & 0 & 1 \\ 0 & 0 & 0 & 1 & 0 \\ 0 & 0 & 1 & 0 & 0 \\ 1 & 1 & 0 & 0 & 0 \\ 1 & 0 & 0 & 0 & 0 \end{pmatrix}$ | 1  |
| 106. | $(xyx)^3$       | $s_1s_3s_3s_3s_3$ | $\begin{pmatrix} 1 & 0 & 0 & 0 & 1 \\ 0 & 0 & 0 & 1 & 0 \\ 0 & 0 & 1 & 0 & 0 \\ 0 & 1 & 0 & 0 & 0 \\ 1 & 0 & 0 & 0 & 0 \end{pmatrix}$ | 1  |
| 107. | $(x^3y)^2xy$    | $s_1s_2s_1s_3s_3$ | $\begin{pmatrix} 0 & 1 & 0 & 0 & 1 \\ 0 & 0 & 0 & 1 & 0 \\ 1 & 1 & 1 & 0 & 0 \\ 0 & 0 & 1 & 0 & 0 \\ 1 & 0 & 0 & 0 & 0 \end{pmatrix}$ | -1 |



|      |                |                       |                                                                                                                                       |    |
|------|----------------|-----------------------|---------------------------------------------------------------------------------------------------------------------------------------|----|
| 108. | $(xy)^2$       | $s_1 s_3 s_1 s_3 s_3$ | $\begin{pmatrix} 1 & 0 & 0 & 0 & 1 \\ 0 & 0 & 0 & 1 & 0 \\ 0 & 1 & 1 & 0 & 0 \\ 0 & 0 & 1 & 0 & 0 \\ 1 & 0 & 0 & 0 & 0 \end{pmatrix}$ | -1 |
| 109. | $x^2(x^2y)^2x$ | $s_1 s_2 s_3 s_1 s_1$ | $\begin{pmatrix} 0 & 0 & 1 & 1 & 1 \\ 0 & 1 & 0 & 0 & 1 \\ 0 & 0 & 0 & 1 & 0 \\ 1 & 1 & 0 & 0 & 0 \\ 1 & 0 & 0 & 0 & 0 \end{pmatrix}$ | 1  |
| 110. | $(yx^2)^2y$    | $s_1 s_3 s_3 s_1 s_1$ | $\begin{pmatrix} 0 & 0 & 1 & 1 & 1 \\ 1 & 0 & 0 & 0 & 1 \\ 0 & 0 & 0 & 1 & 0 \\ 0 & 1 & 0 & 0 & 0 \\ 1 & 0 & 0 & 0 & 0 \end{pmatrix}$ | 1  |
| 111. | $x(xy)^2x^2y$  | $s_1 s_2 s_3 s_1 s_3$ | $\begin{pmatrix} 0 & 1 & 0 & 0 & 1 \\ 0 & 0 & 1 & 1 & 0 \\ 0 & 0 & 0 & 1 & 0 \\ 1 & 1 & 0 & 0 & 0 \\ 1 & 0 & 0 & 0 & 0 \end{pmatrix}$ | -1 |
| 112. | $(xyx)^3y$     | $s_1 s_3 s_3 s_1 s_3$ | $\begin{pmatrix} 1 & 0 & 0 & 0 & 1 \\ 0 & 0 & 1 & 1 & 0 \\ 0 & 0 & 0 & 1 & 0 \\ 0 & 1 & 0 & 0 & 0 \\ 1 & 0 & 0 & 0 & 0 \end{pmatrix}$ | -1 |
| 113. | $(x^3y)^2x$    | $s_1 s_2 s_1 s_1 s_3$ | $\begin{pmatrix} 0 & 1 & 0 & 0 & 1 \\ 1 & 1 & 1 & 1 & 0 \\ 0 & 0 & 0 & 1 & 0 \\ 0 & 0 & 1 & 0 & 0 \\ 1 & 0 & 0 & 0 & 0 \end{pmatrix}$ | 1  |
| 114. | $xyx$          | $s_1 s_3 s_1 s_1 s_3$ | $\begin{pmatrix} 1 & 0 & 0 & 0 & 1 \\ 0 & 1 & 1 & 1 & 0 \\ 0 & 0 & 0 & 1 & 0 \\ 0 & 0 & 1 & 0 & 0 \\ 1 & 0 & 0 & 0 & 0 \end{pmatrix}$ | 1  |
| 115. | $x^3y$         | $s_1 s_3 s_3 s_2 s_2$ | $\begin{pmatrix} 0 & 0 & 1 & 0 & 1 \\ 0 & 1 & 0 & 1 & 0 \\ 1 & 0 & 0 & 0 & 1 \\ 0 & 0 & 0 & 1 & 0 \\ 1 & 0 & 0 & 0 & 0 \end{pmatrix}$ | 1  |
| 116. | $x^3$          | $s_1 s_2 s_3 s_2 s_2$ | $\begin{pmatrix} 0 & 0 & 1 & 0 & 1 \\ 1 & 1 & 0 & 1 & 0 \\ 0 & 1 & 0 & 0 & 1 \\ 0 & 0 & 0 & 1 & 0 \\ 1 & 0 & 0 & 0 & 0 \end{pmatrix}$ | 1  |
| 117. | $x^2(xy)^2x^4$ | $s_1 s_2 s_1 s_2 s_3$ | $\begin{pmatrix} 0 & 1 & 0 & 0 & 1 \\ 0 & 0 & 1 & 1 & 0 \\ 1 & 1 & 1 & 0 & 0 \\ 0 & 0 & 0 & 1 & 0 \\ 1 & 0 & 0 & 0 & 0 \end{pmatrix}$ | 1  |

|      |                |                   |                                                                                                                                       |    |
|------|----------------|-------------------|---------------------------------------------------------------------------------------------------------------------------------------|----|
| 118. | $x^4yx^4$      | $s_1s_3s_1s_2s_3$ | $\begin{pmatrix} 1 & 0 & 0 & 0 & 1 \\ 0 & 0 & 1 & 1 & 0 \\ 0 & 1 & 1 & 0 & 0 \\ 0 & 0 & 0 & 1 & 0 \\ 1 & 0 & 0 & 0 & 0 \end{pmatrix}$ | 1  |
| 119. | $x(x^2y)^2xyx$ | $s_1s_2s_3s_2s_3$ | $\begin{pmatrix} 0 & 1 & 0 & 0 & 1 \\ 1 & 1 & 0 & 1 & 0 \\ 0 & 0 & 1 & 0 & 0 \\ 0 & 0 & 0 & 1 & 0 \\ 1 & 0 & 0 & 0 & 0 \end{pmatrix}$ | -1 |
| 120. | $(yx)^2$       | $s_1s_3s_3s_2s_3$ | $\begin{pmatrix} 1 & 0 & 0 & 0 & 1 \\ 0 & 1 & 0 & 1 & 0 \\ 0 & 0 & 1 & 0 & 0 \\ 0 & 0 & 0 & 1 & 0 \\ 1 & 0 & 0 & 0 & 0 \end{pmatrix}$ | -1 |
